# Supplementary material for: Data-Driven Extract Method Recommendations: A Study at ING
Source: arXiv:2107.05396 source file (2021-07-22)
Supplement: Supplementary file 1 [file appendix.tex]

\section{Violin plots (RQ1)}
\label{app:Violin plots-data-analysis}

In the following, we list all the violin plots we used to answer RQ1.

\begin{figure*}[htbp]
    \begin{subfigure}[htbp]{0.45\linewidth}
        \centering
        \includegraphics[width=0.65\textwidth]{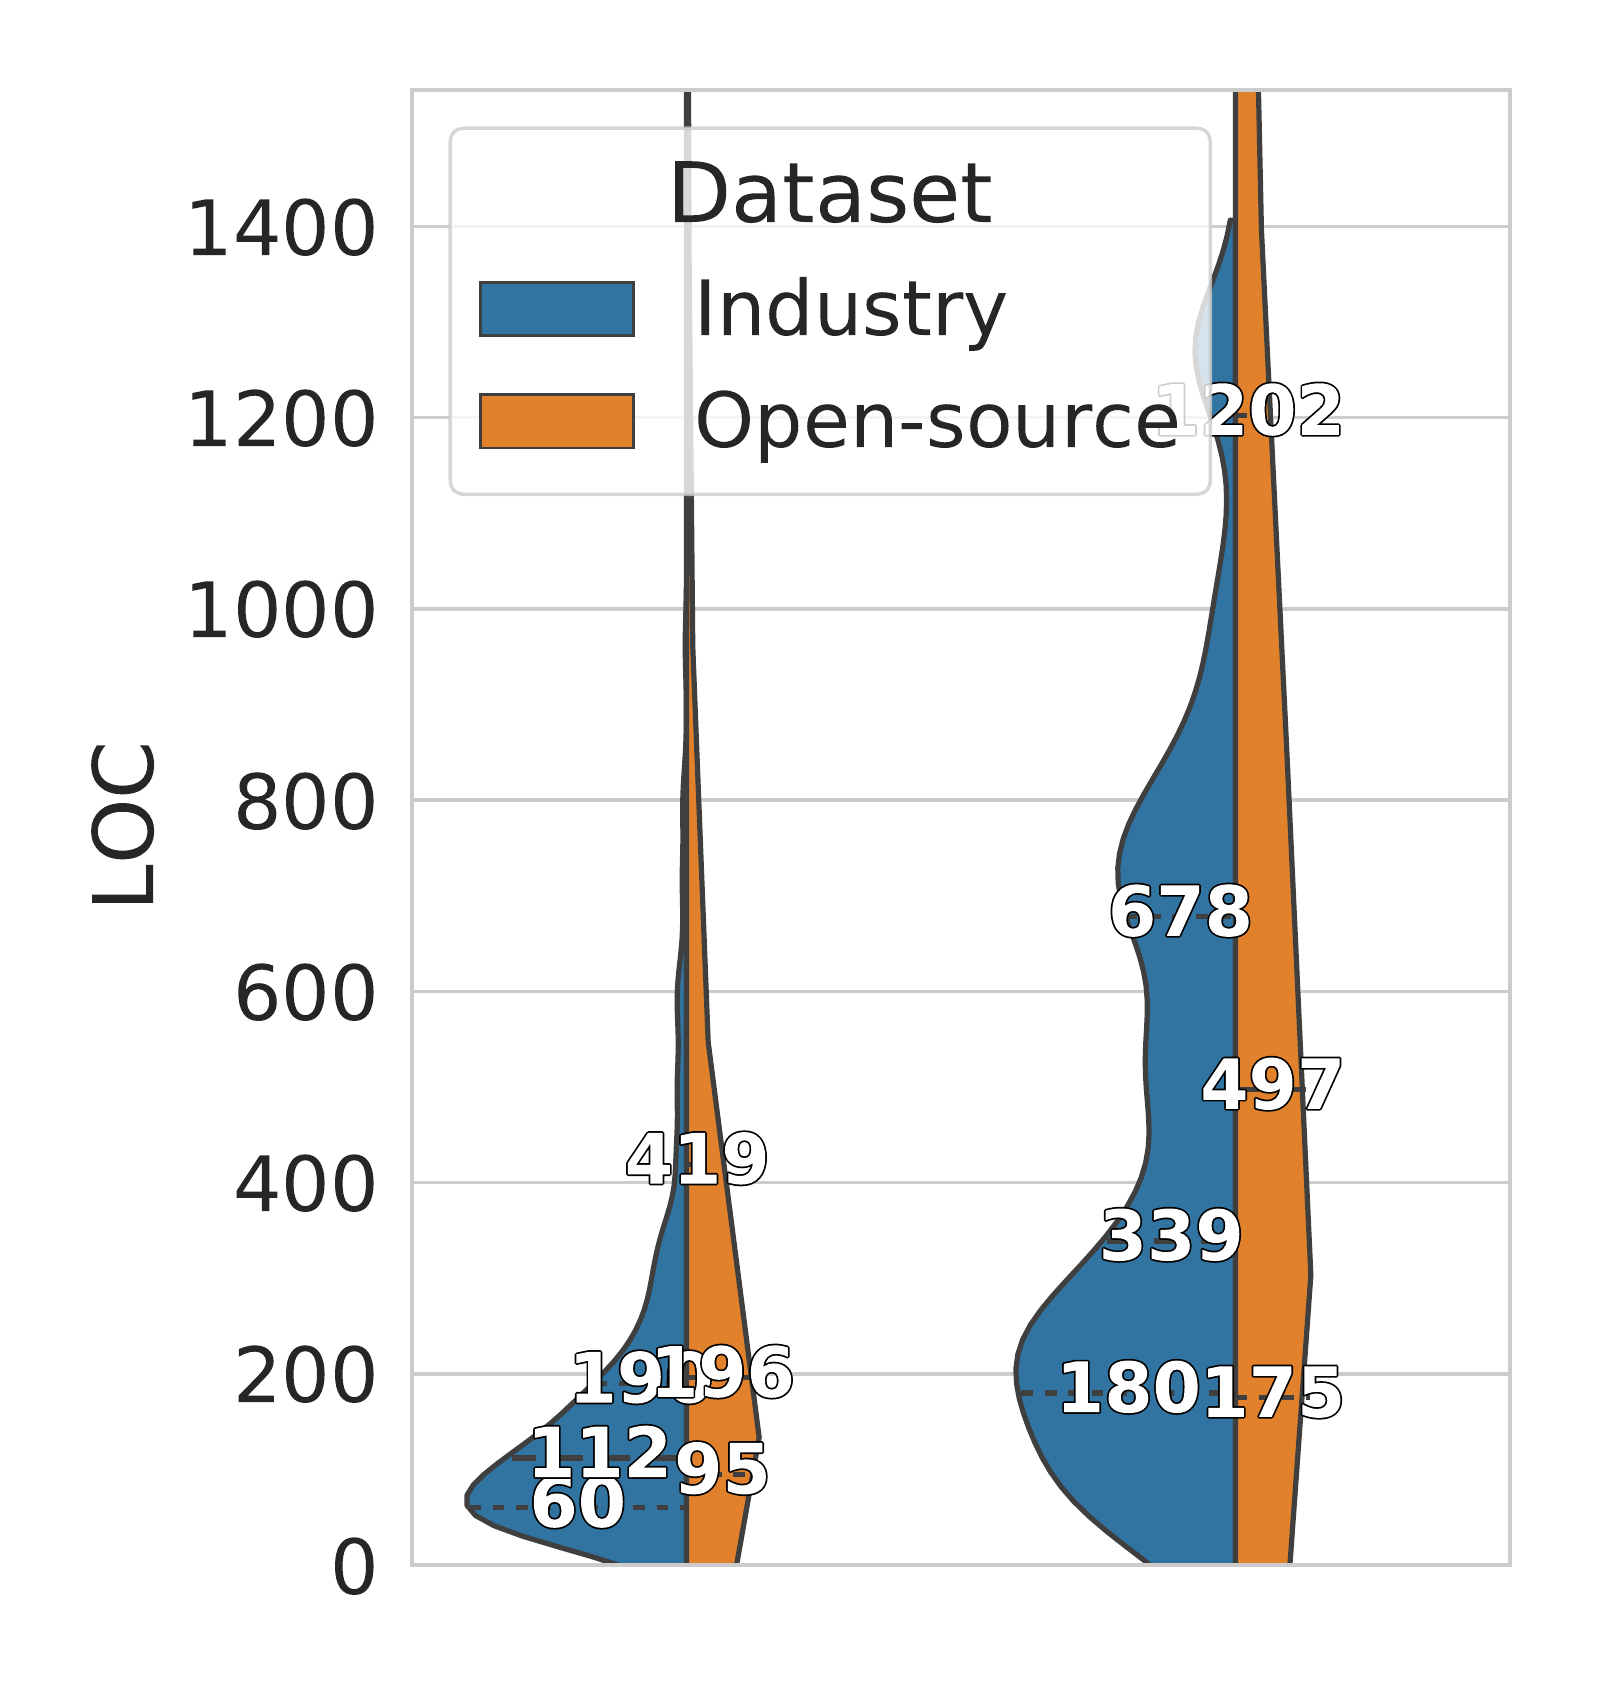}
        \caption{Class-level LOC: The left violin plot indicates classes that contain methods that underwent an Extract Method refactoring.
            The right violin plot indicates classes that do not need to undergo an Extract Method refactoring.}
    \end{subfigure}
    \hfill
    \begin{subfigure}[htbp]{0.45\linewidth}
        \centering
        \includegraphics[width=0.65\textwidth]{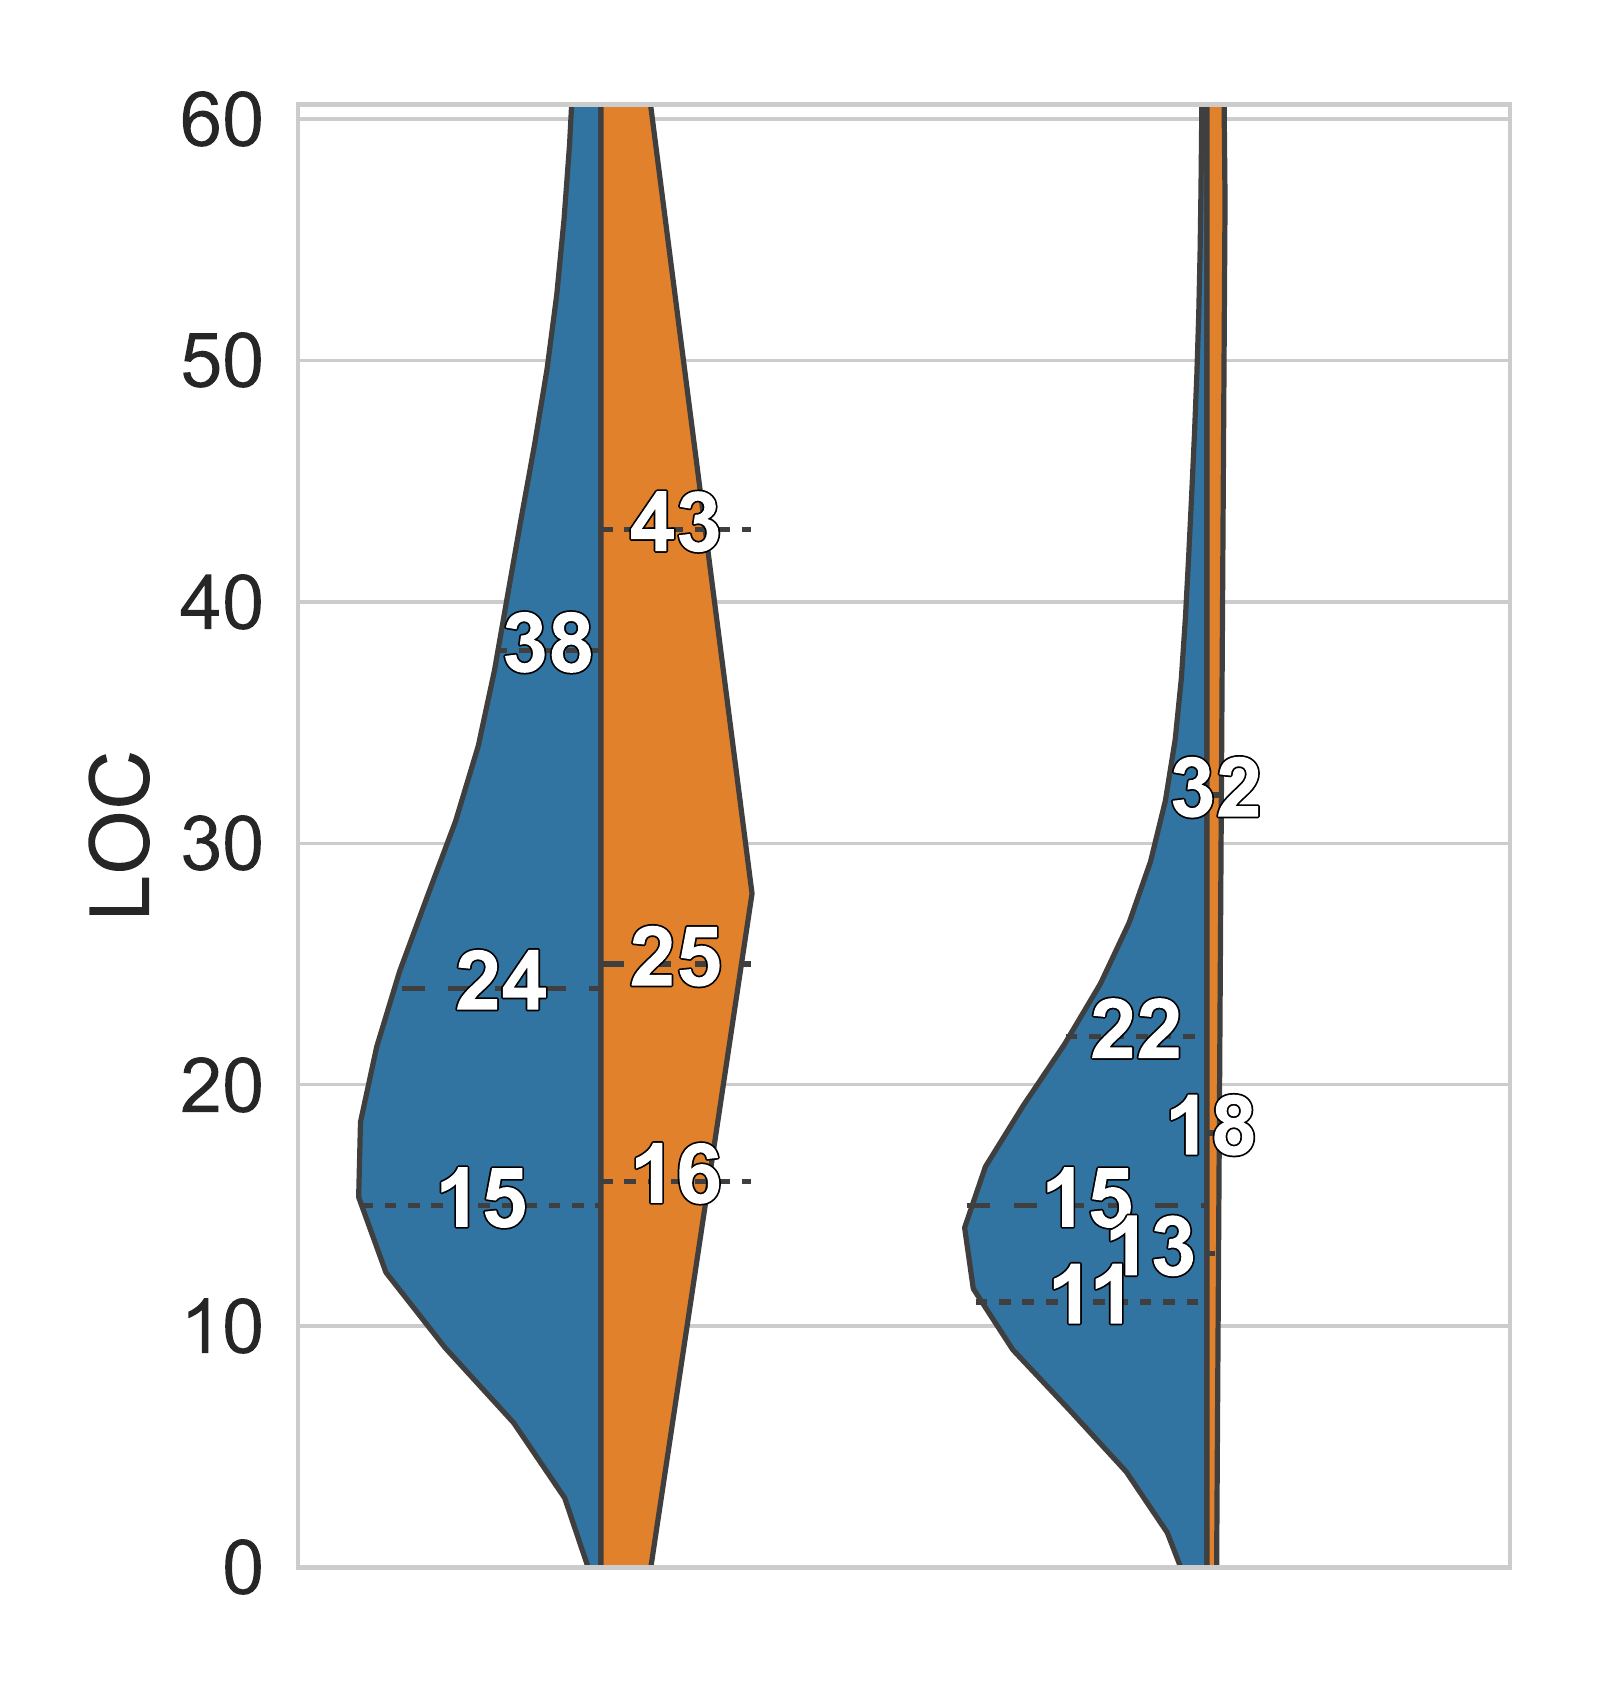}
        \caption{Method-level LOC: The left violin plot indicates methods that underwent an Extract Method refactoring.
            The right violin plot indicates methods that do not need to undergo an Extract Method refactoring.}
    \end{subfigure}
    \caption{LOC distributions for open-source and ING code on both class- and method-level.}
    %\label{fig:only-violin-plot-loc}
\end{figure*}

\begin{figure*}
    \begin{subfigure}[htbp]{0.45\linewidth}
        \centering
        \includegraphics[width=0.65\textwidth]{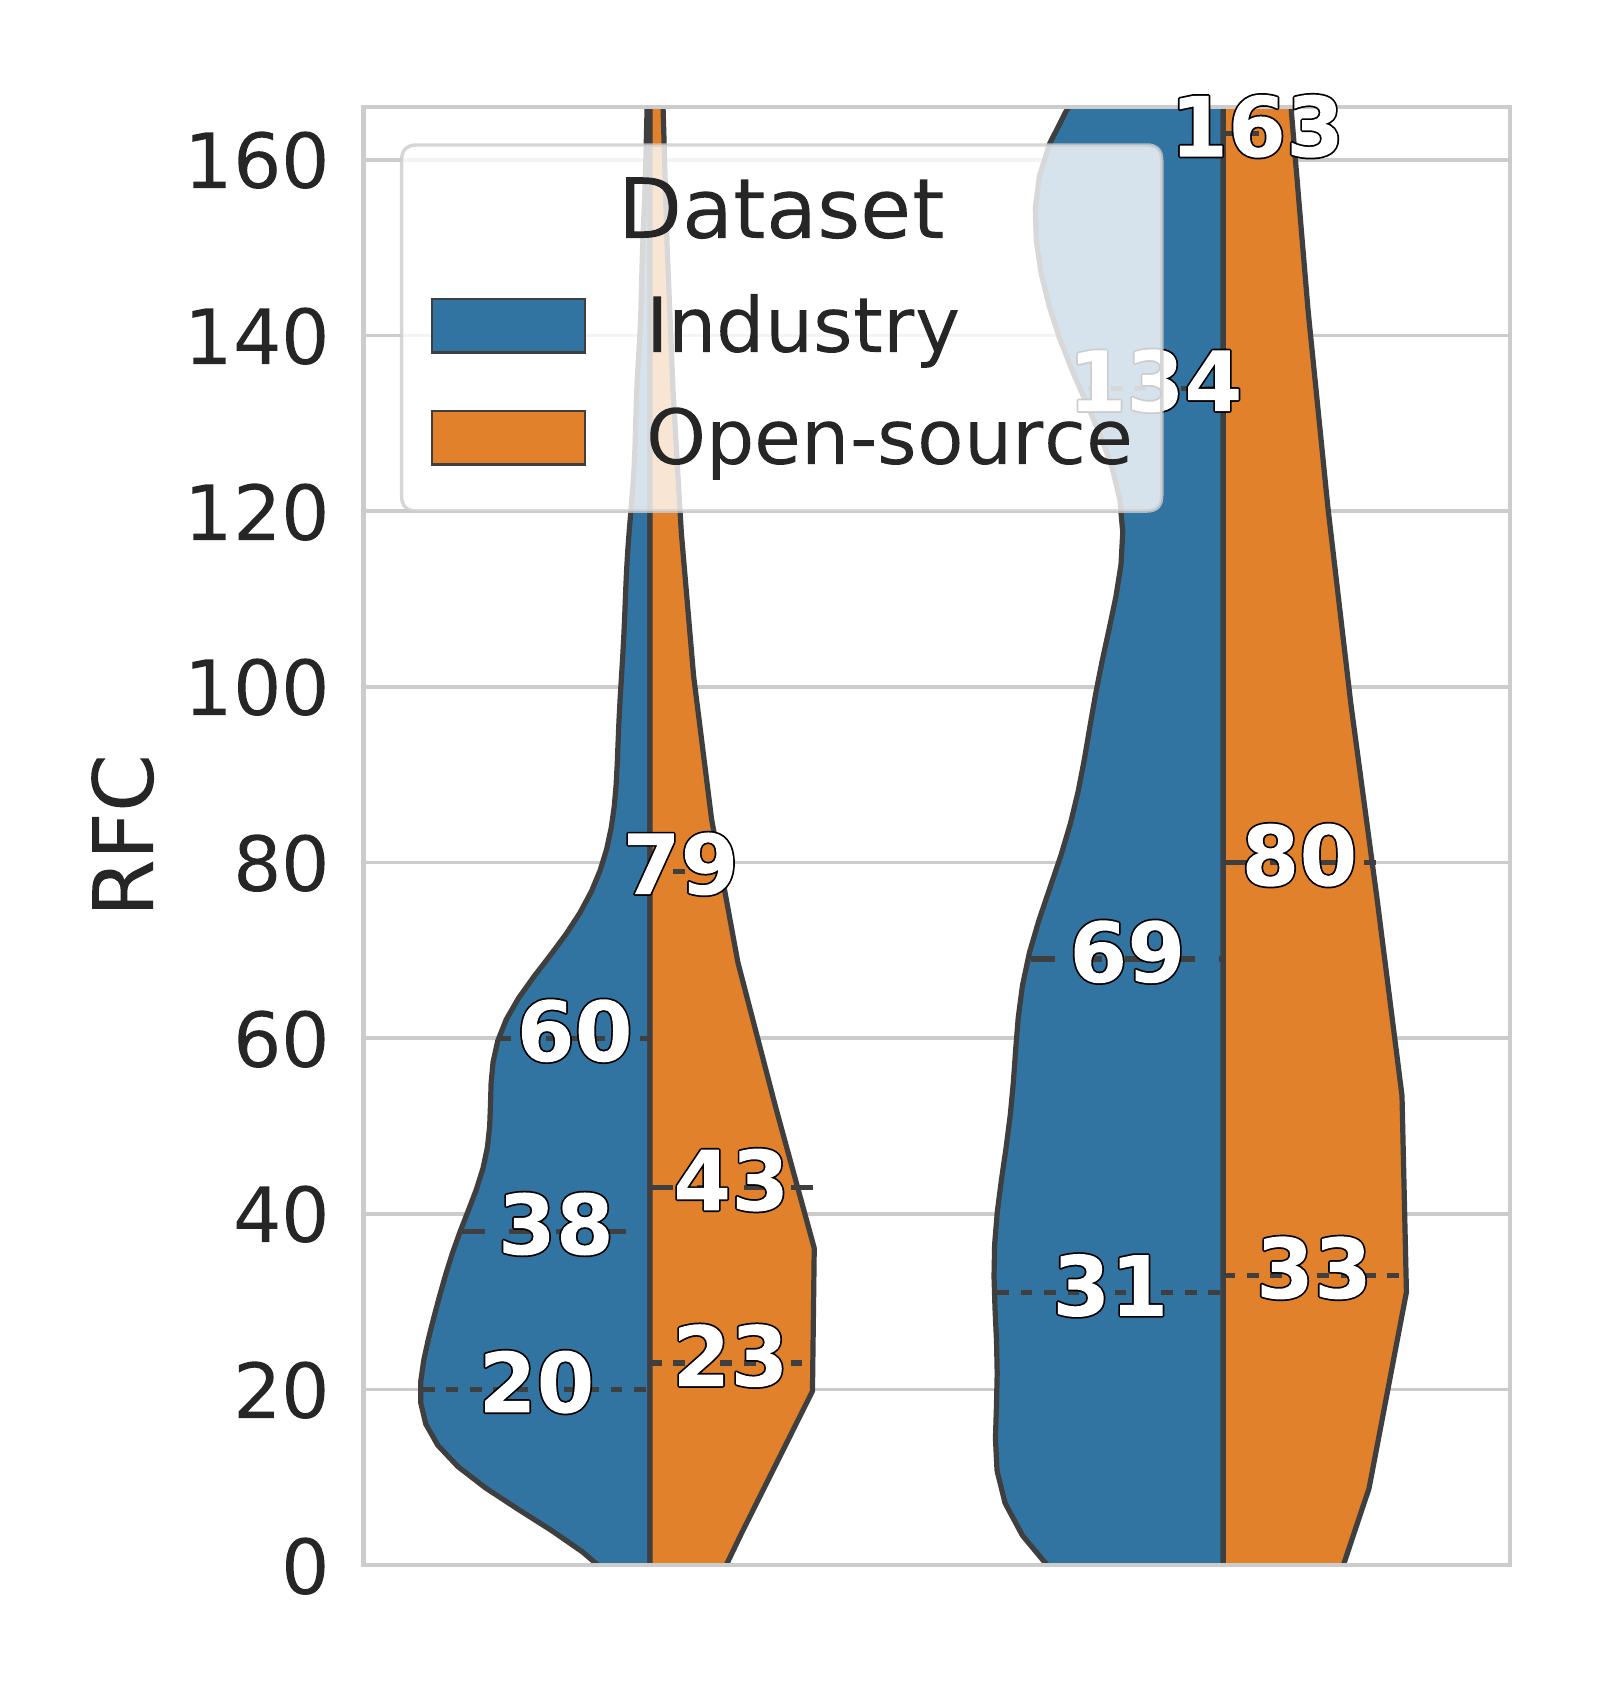}
        \caption{Class-level RFC: The left violin plot indicates classes that contain methods that underwent an Extract Method refactoring.
            The right violin plot indicates classes that do not need to undergo an Extract Method refactoring.}
    \end{subfigure}
    \hfill
    \begin{subfigure}[htbp]{0.45\linewidth}
        \centering
        \includegraphics[width=0.65\textwidth]{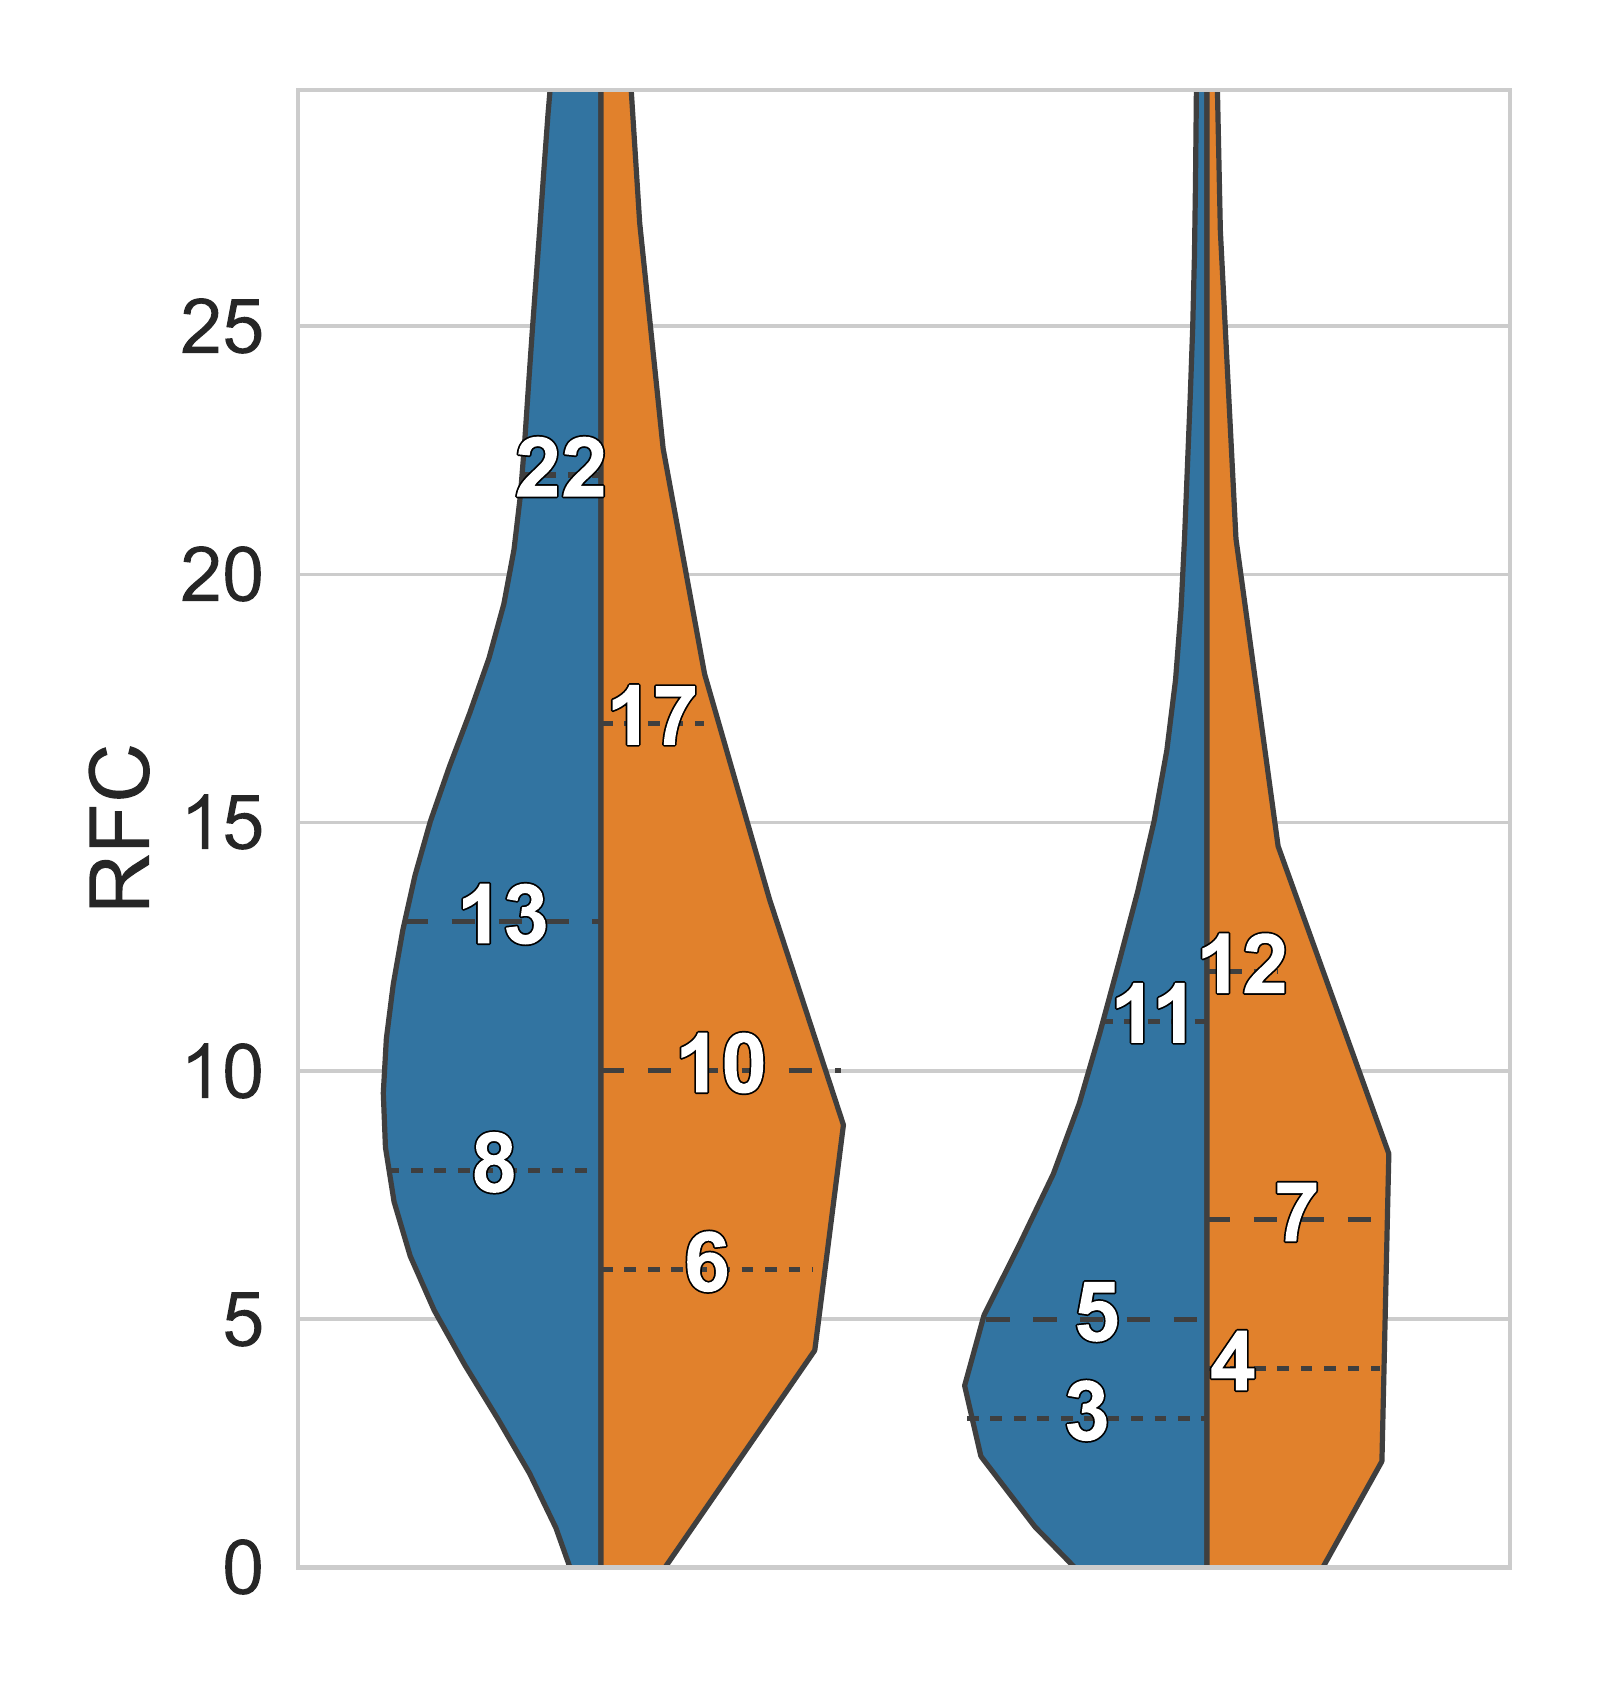}
        \caption{Method-level RFC: The left violin plot indicates methods that underwent an Extract Method refactoring.
            The right violin plot indicates methods that do not need to undergo an Extract Method refactoring.}
    \end{subfigure}
    \caption{RFC distributions for open-source and ING code on both class- and method-level.}
    % \label{fig:only-violin-plot-loc}
\end{figure*}

\begin{figure*}
    \begin{subfigure}[htbp]{0.45\linewidth}
        \centering
        \includegraphics[width=0.65\textwidth]{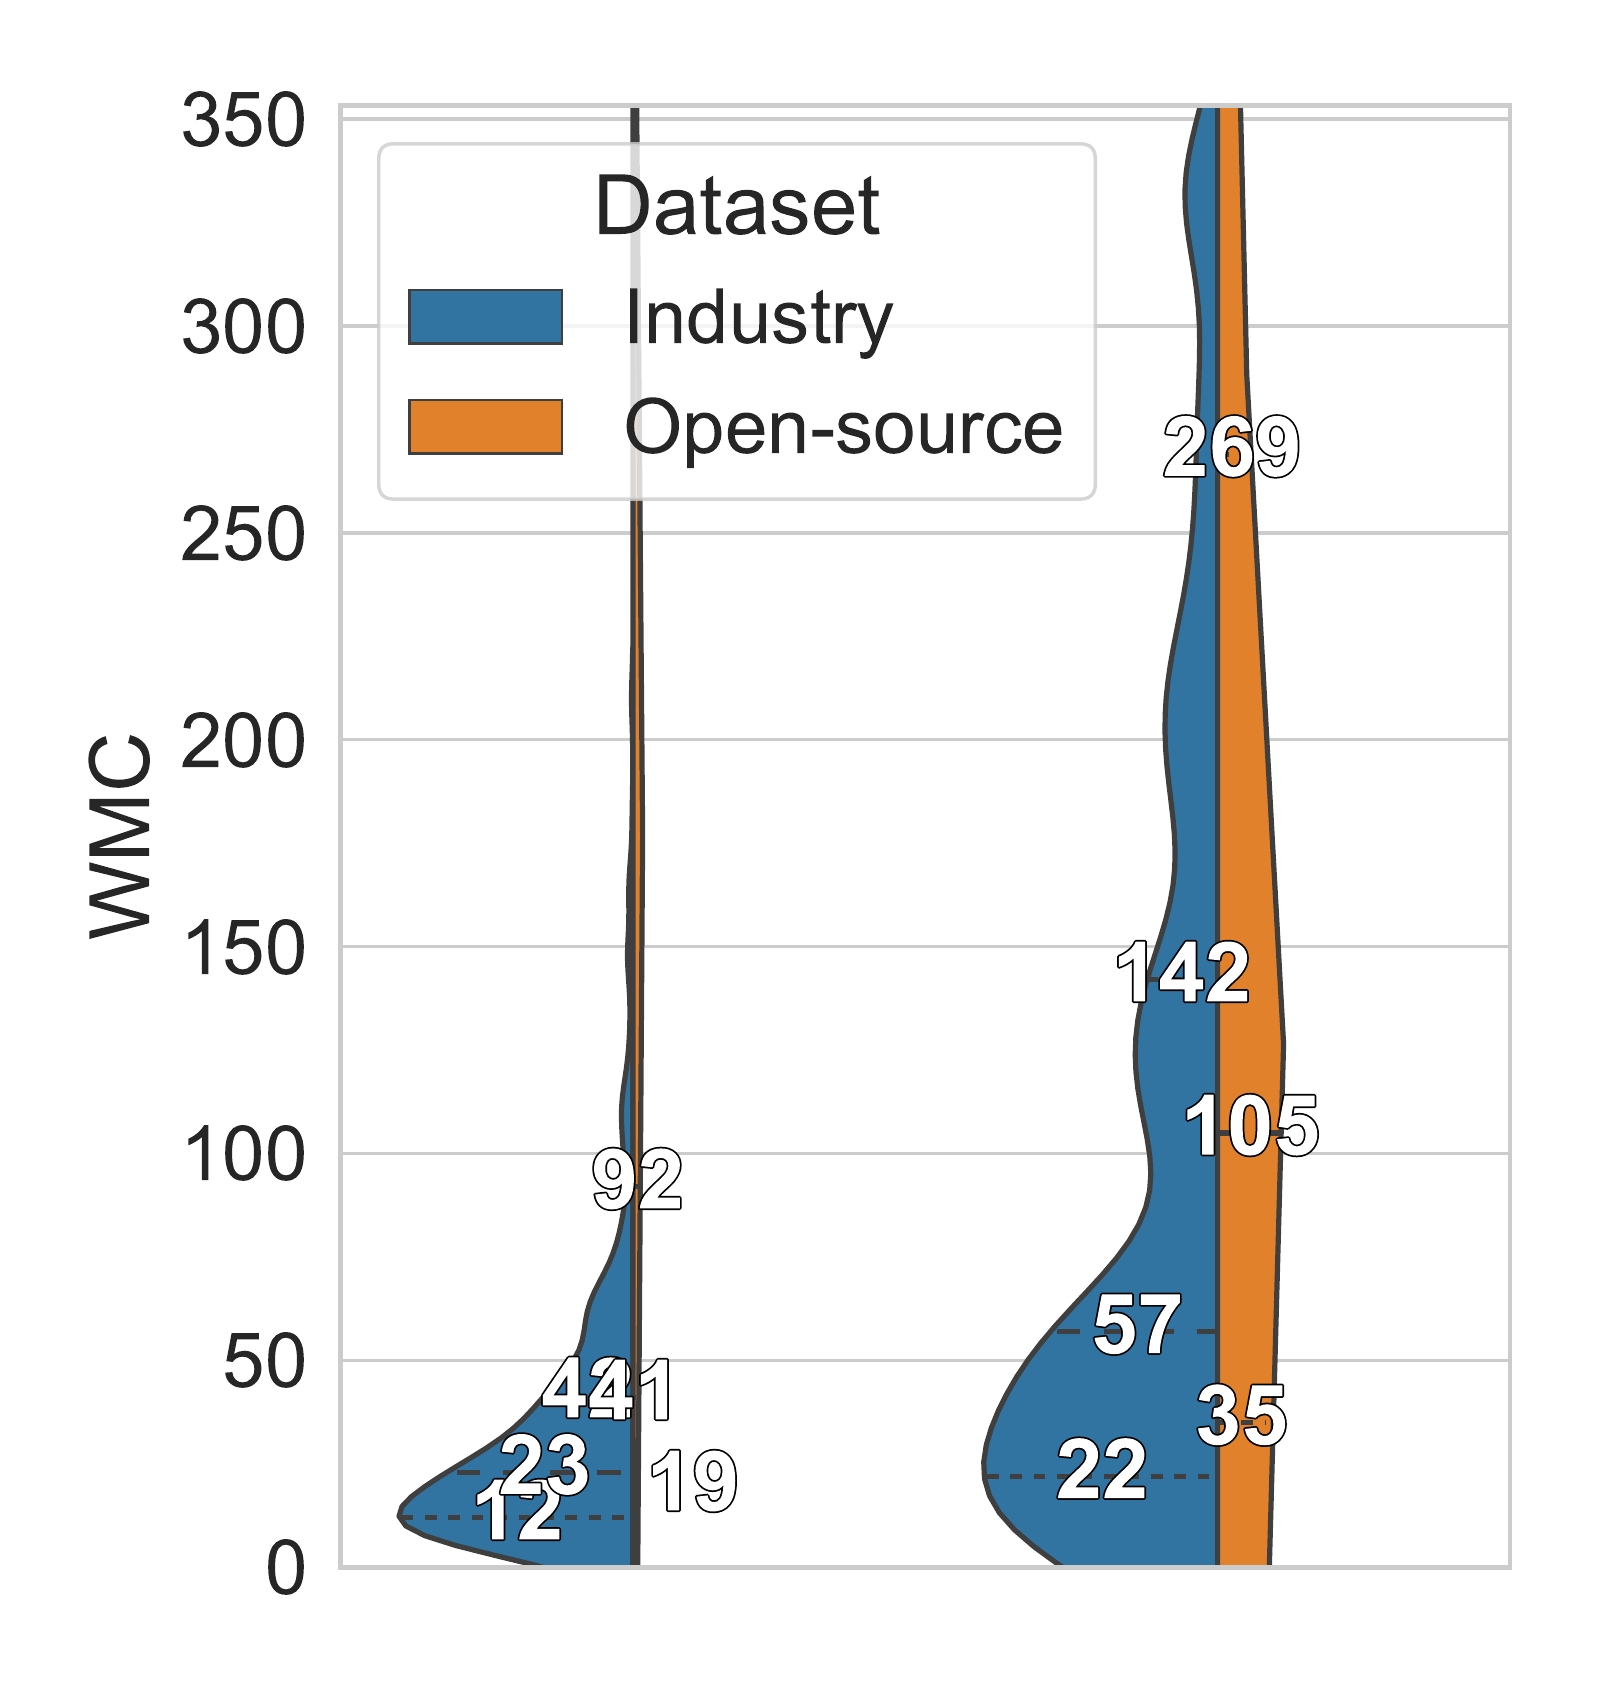}
        \caption{Class-level WMC: The left violin plot indicates classes that contain methods that underwent an Extract Method refactoring.
            The right violin plot indicates classes that do not need to undergo an Extract Method refactoring.}
    \end{subfigure}
    \hfill
    \begin{subfigure}[htbp]{0.45\linewidth}
        \centering
        \includegraphics[width=0.65\textwidth]{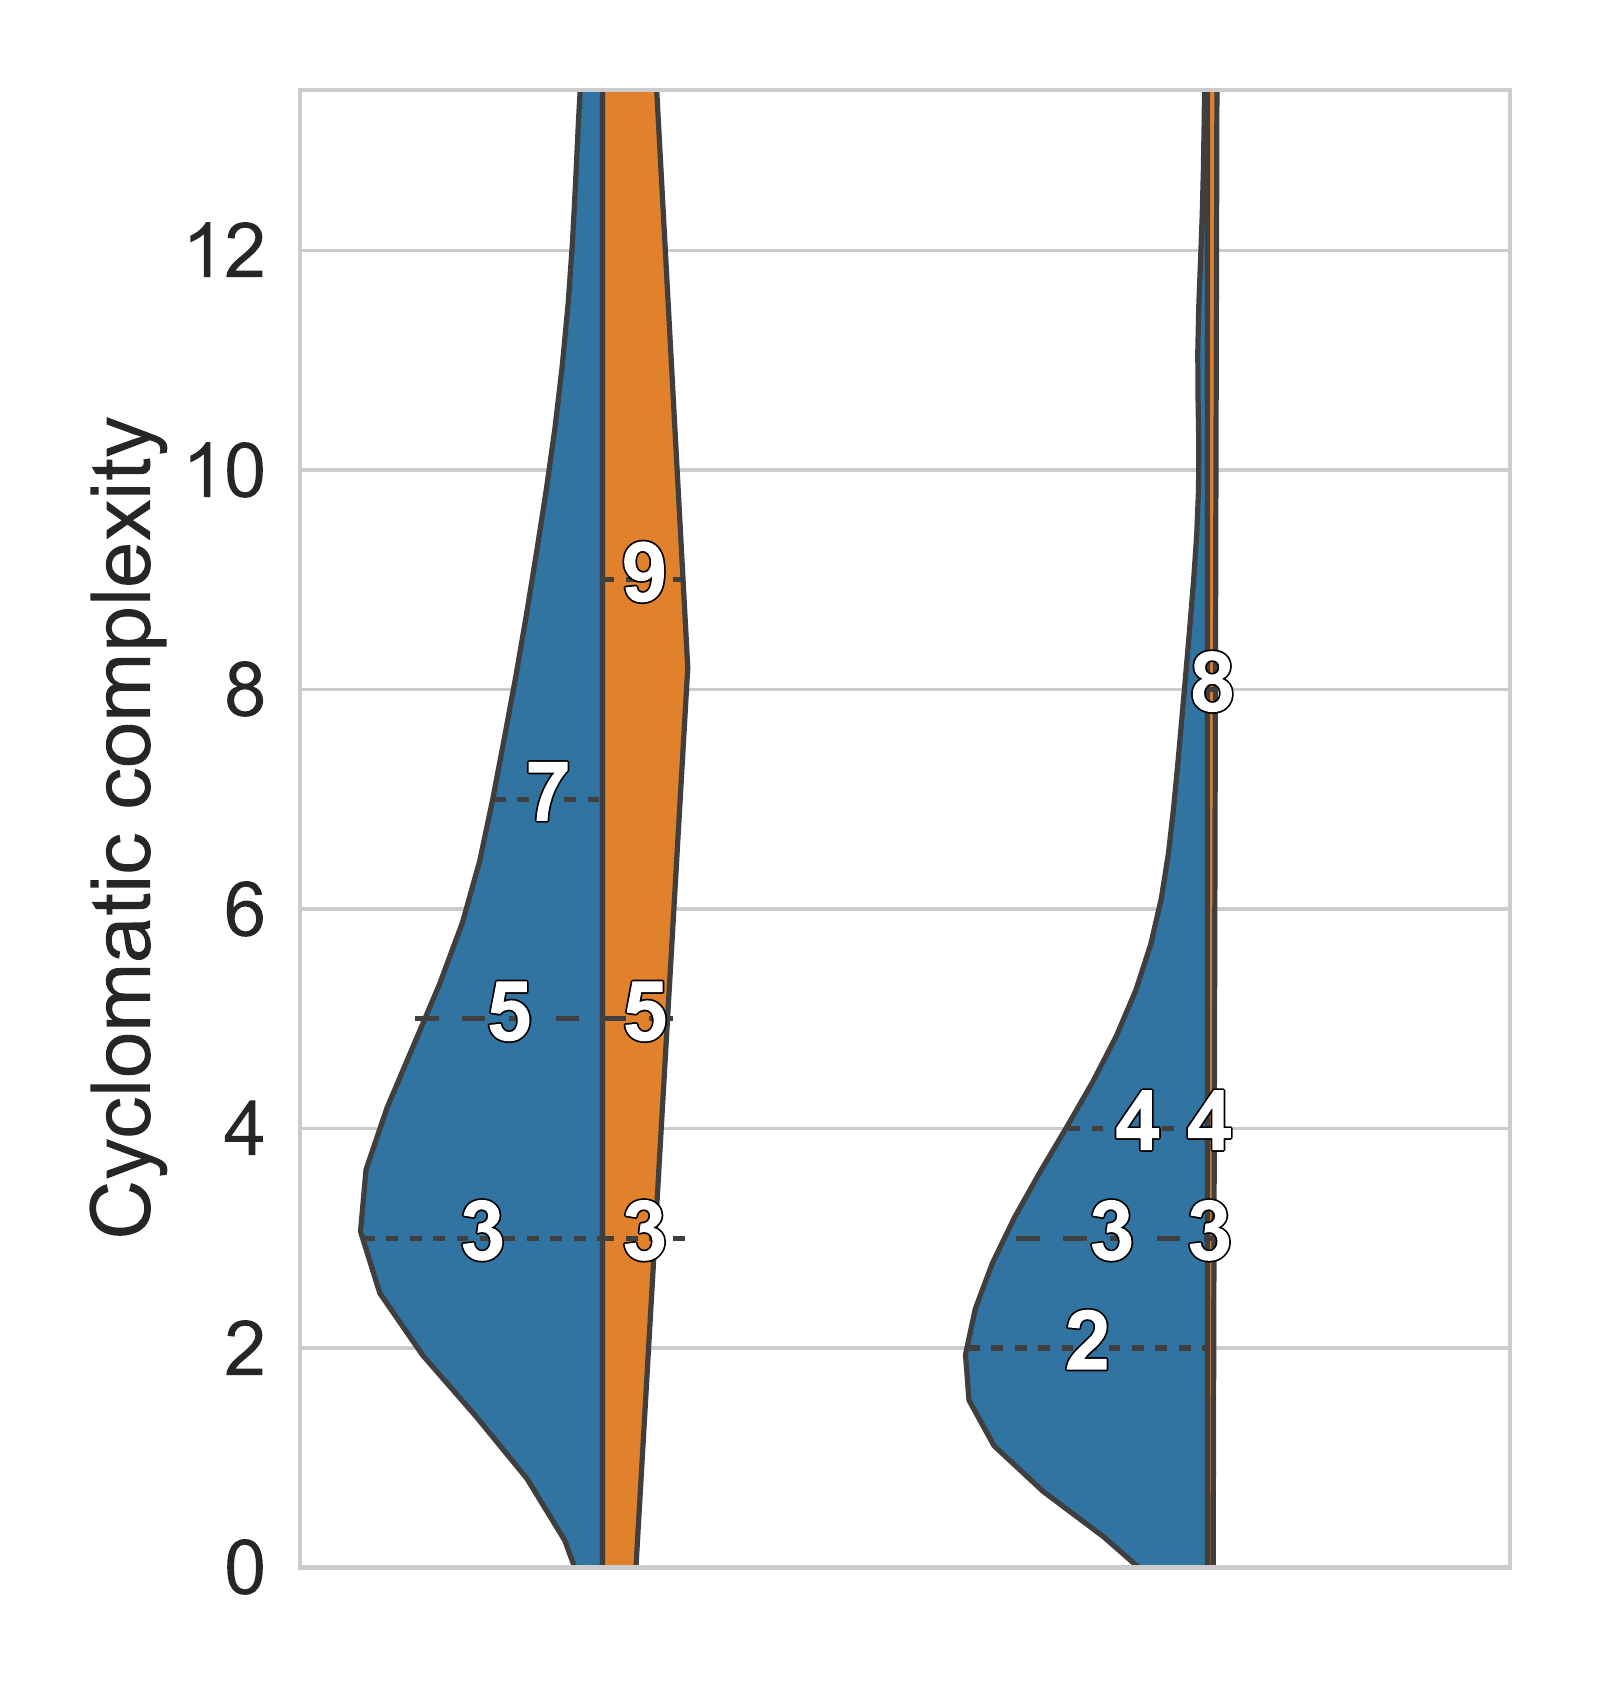}
        \caption{Method-level cyclomatic complexity: The left violin plot indicates methods that underwent an Extract Method refactoring.
            The right violin plot indicates methods that do not need to undergo an Extract Method refactoring.}
    \end{subfigure}
    \caption{WMC and cyclomatic complexity distributions for open-source and ING code on both class- and method-level.}
    %\label{fig:only-violin-plot-loc}
\end{figure*}

\begin{figure*}
    \begin{subfigure}[htbp]{0.45\linewidth}
        \centering
        \includegraphics[width=0.65\textwidth]{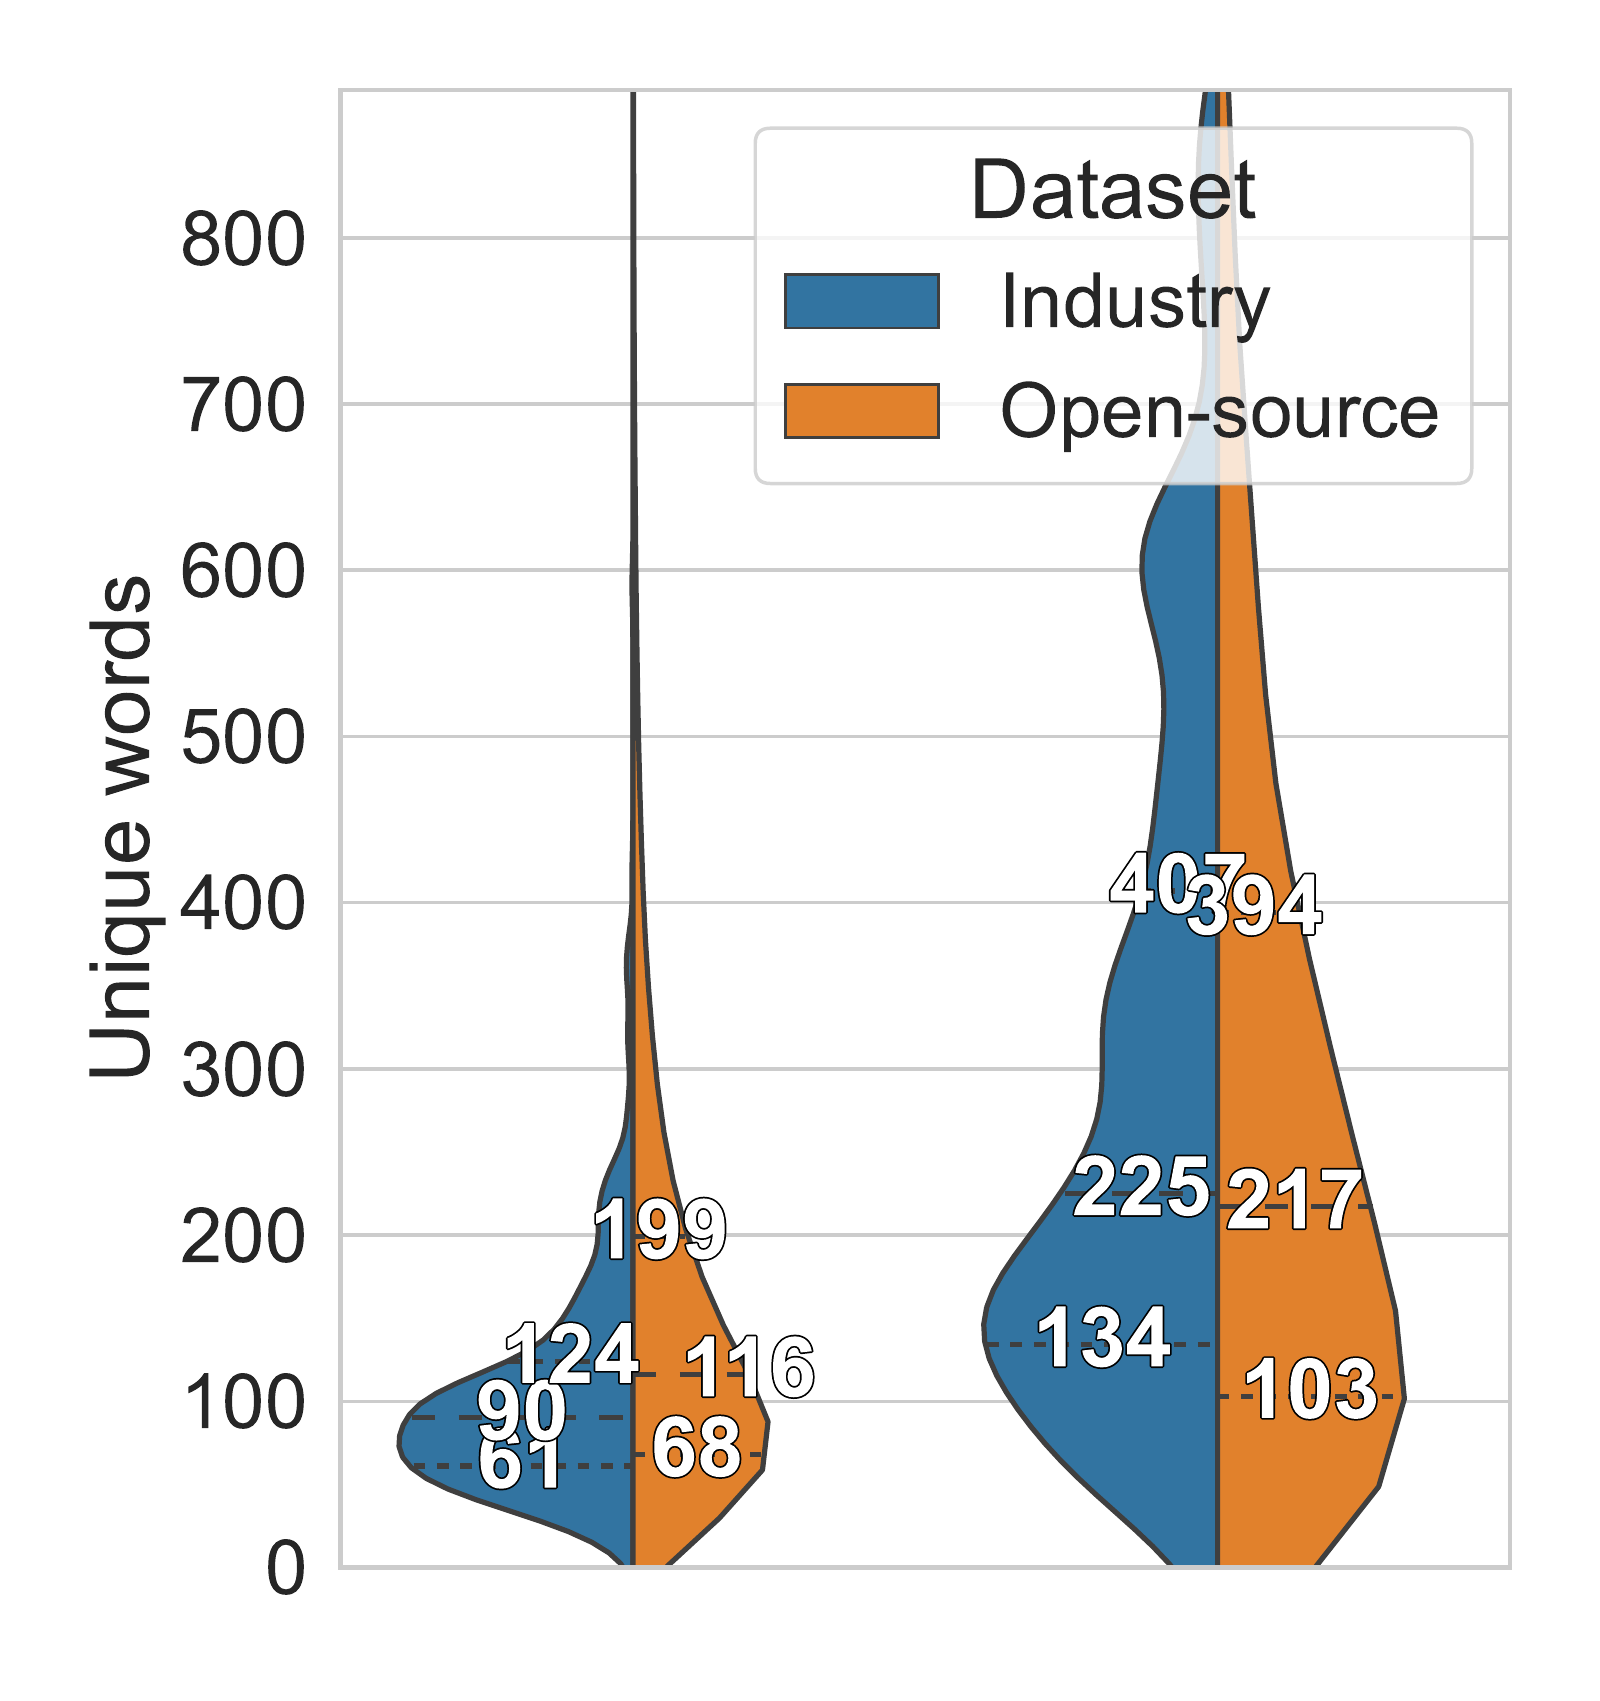}
       \caption{Class-level UniqueWordsQty: The left violin plot indicates classes that contain methods that underwent an Extract Method refactoring.
            The right violin plot indicates classes that do not need to undergo an Extract Method refactoring.}
    \end{subfigure}
    \hfill
    \begin{subfigure}[htbp]{0.45\linewidth}
        \centering
        \includegraphics[width=0.65\textwidth]{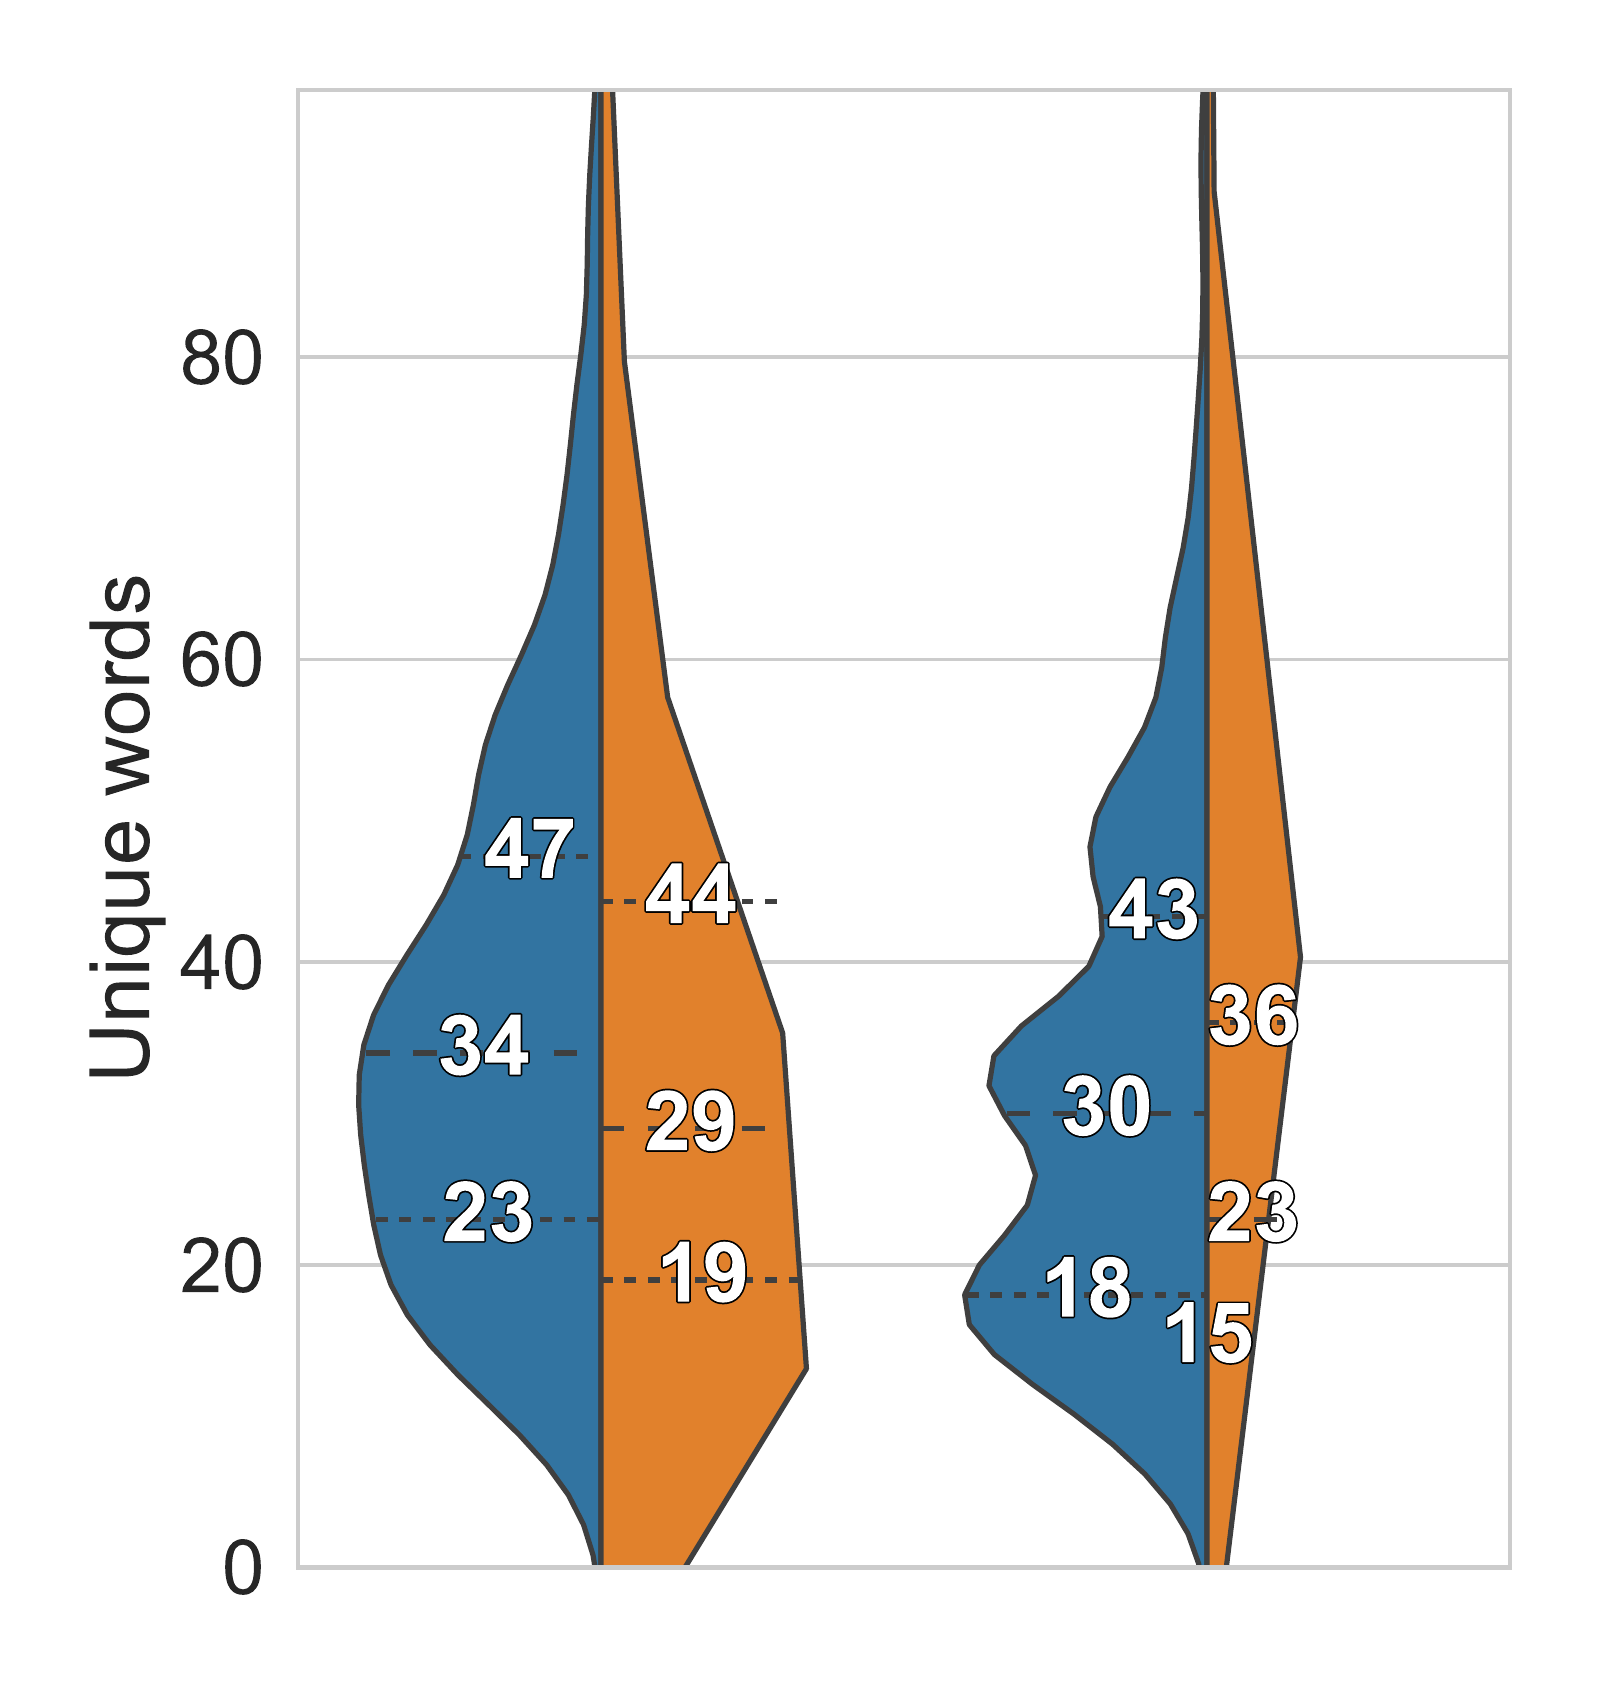}
        \caption{Method-level UniqueWordsQty: The left violin plot indicates methods that underwent an Extract Method refactoring.
            The right violin plot indicates methods that do not need to undergo an Extract Method refactoring.}
    \end{subfigure}
    \caption{UniqueWordsQty distributions for open-source and ING code on both class- and method-level.}
    %\label{fig:only-violin-plot-loc}
\end{figure*}

\begin{figure*}
    \begin{subfigure}[htbp]{0.45\linewidth}
        \centering
        \includegraphics[width=0.65\textwidth]{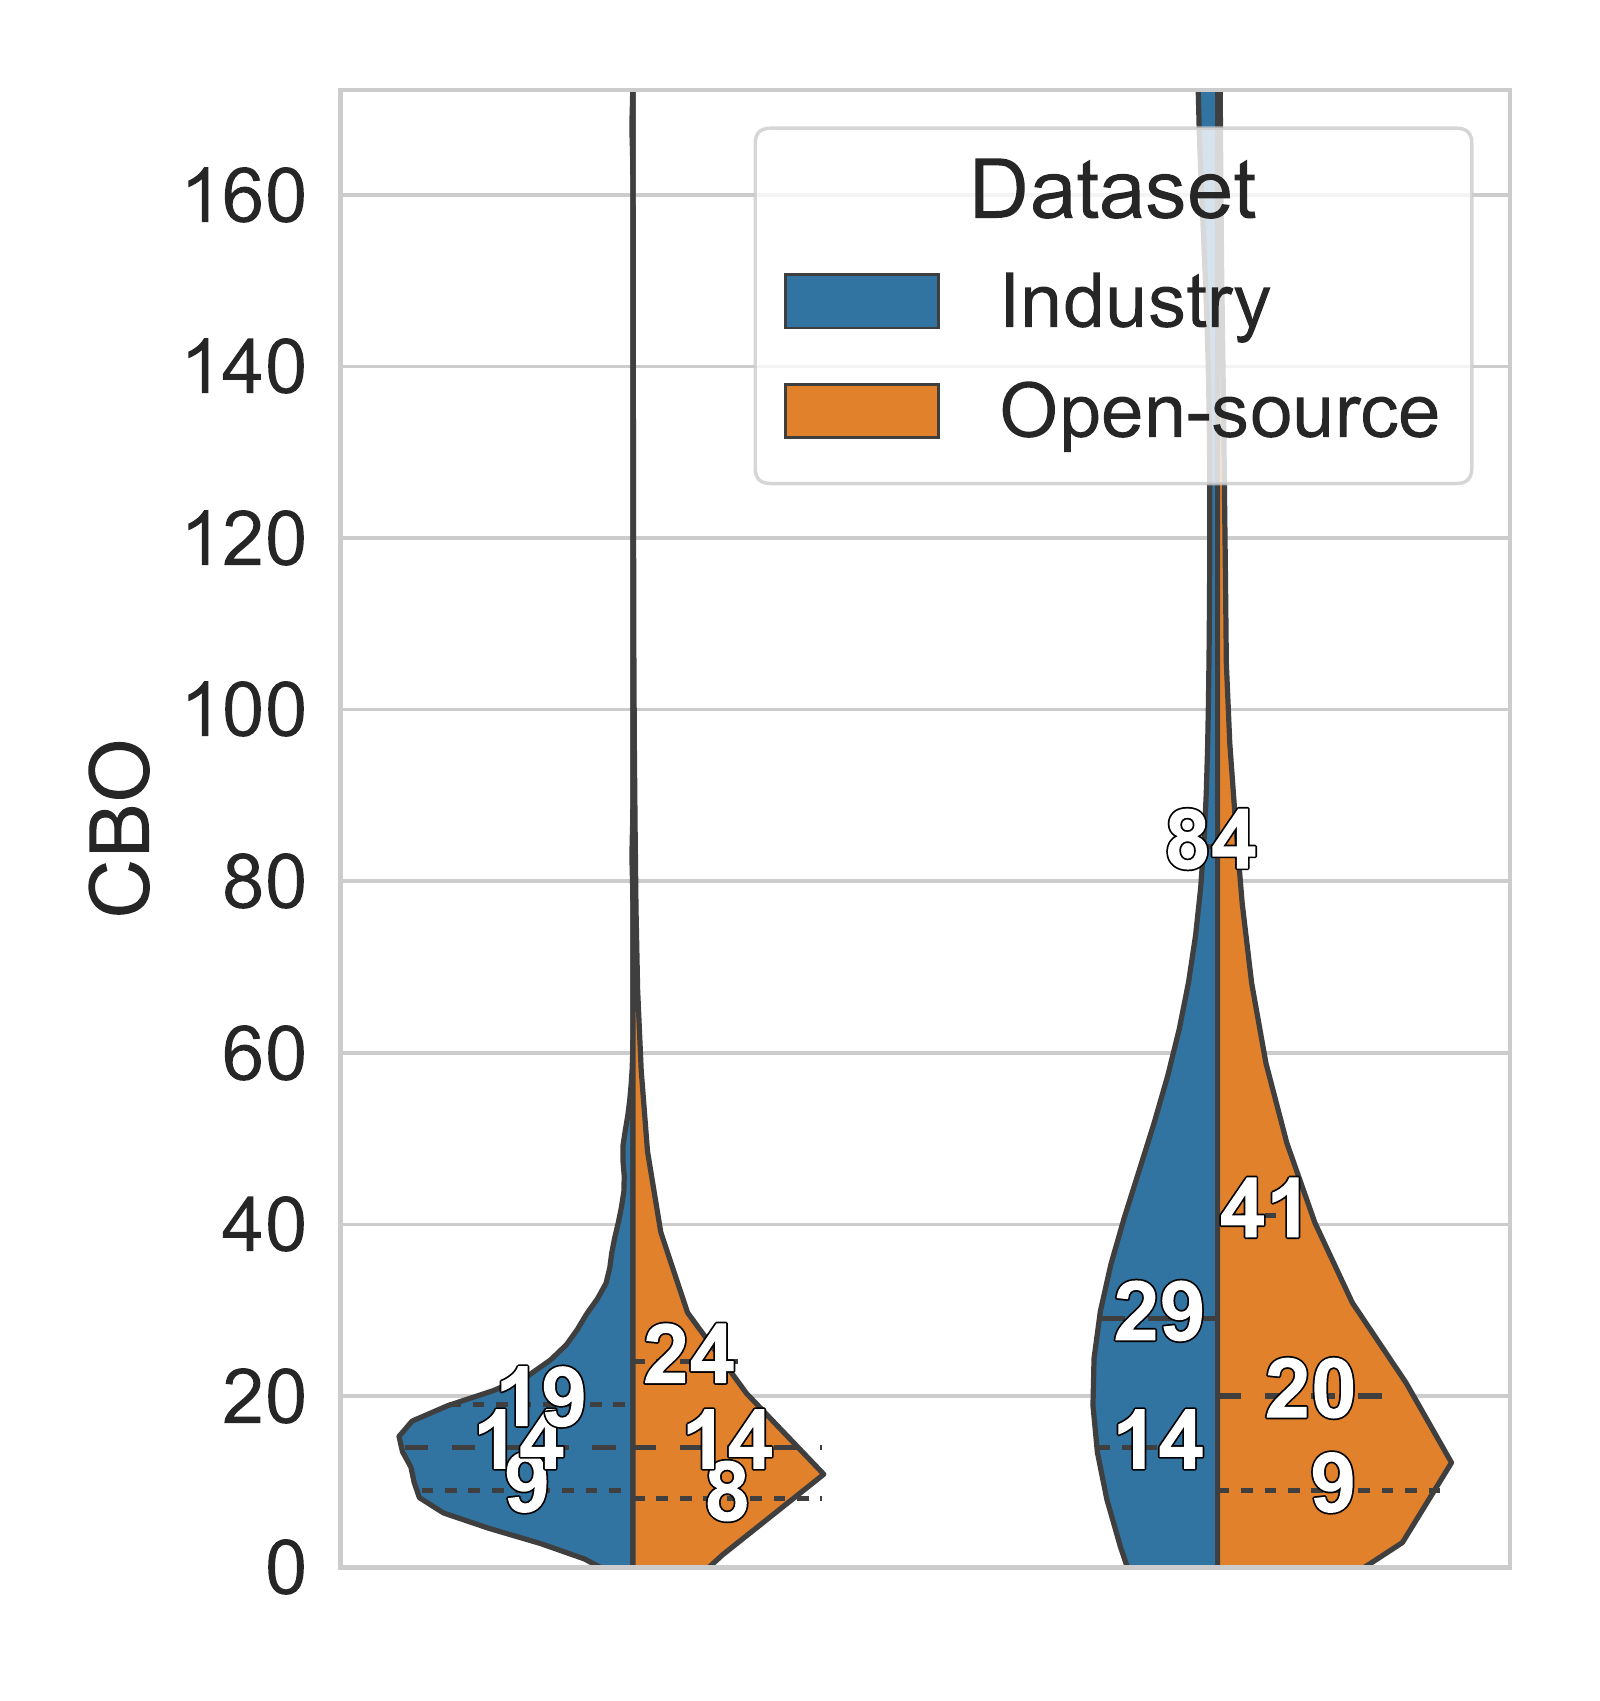}
        \caption{Class-level CBO: The left violin plot indicates classes that contain methods that underwent an Extract Method refactoring.
            The right violin plot indicates classes that do not need to undergo an Extract Method refactoring.}
    \end{subfigure}
    \hfill
    \begin{subfigure}[htbp]{0.45\linewidth}
        \centering
        \includegraphics[width=0.65\textwidth]{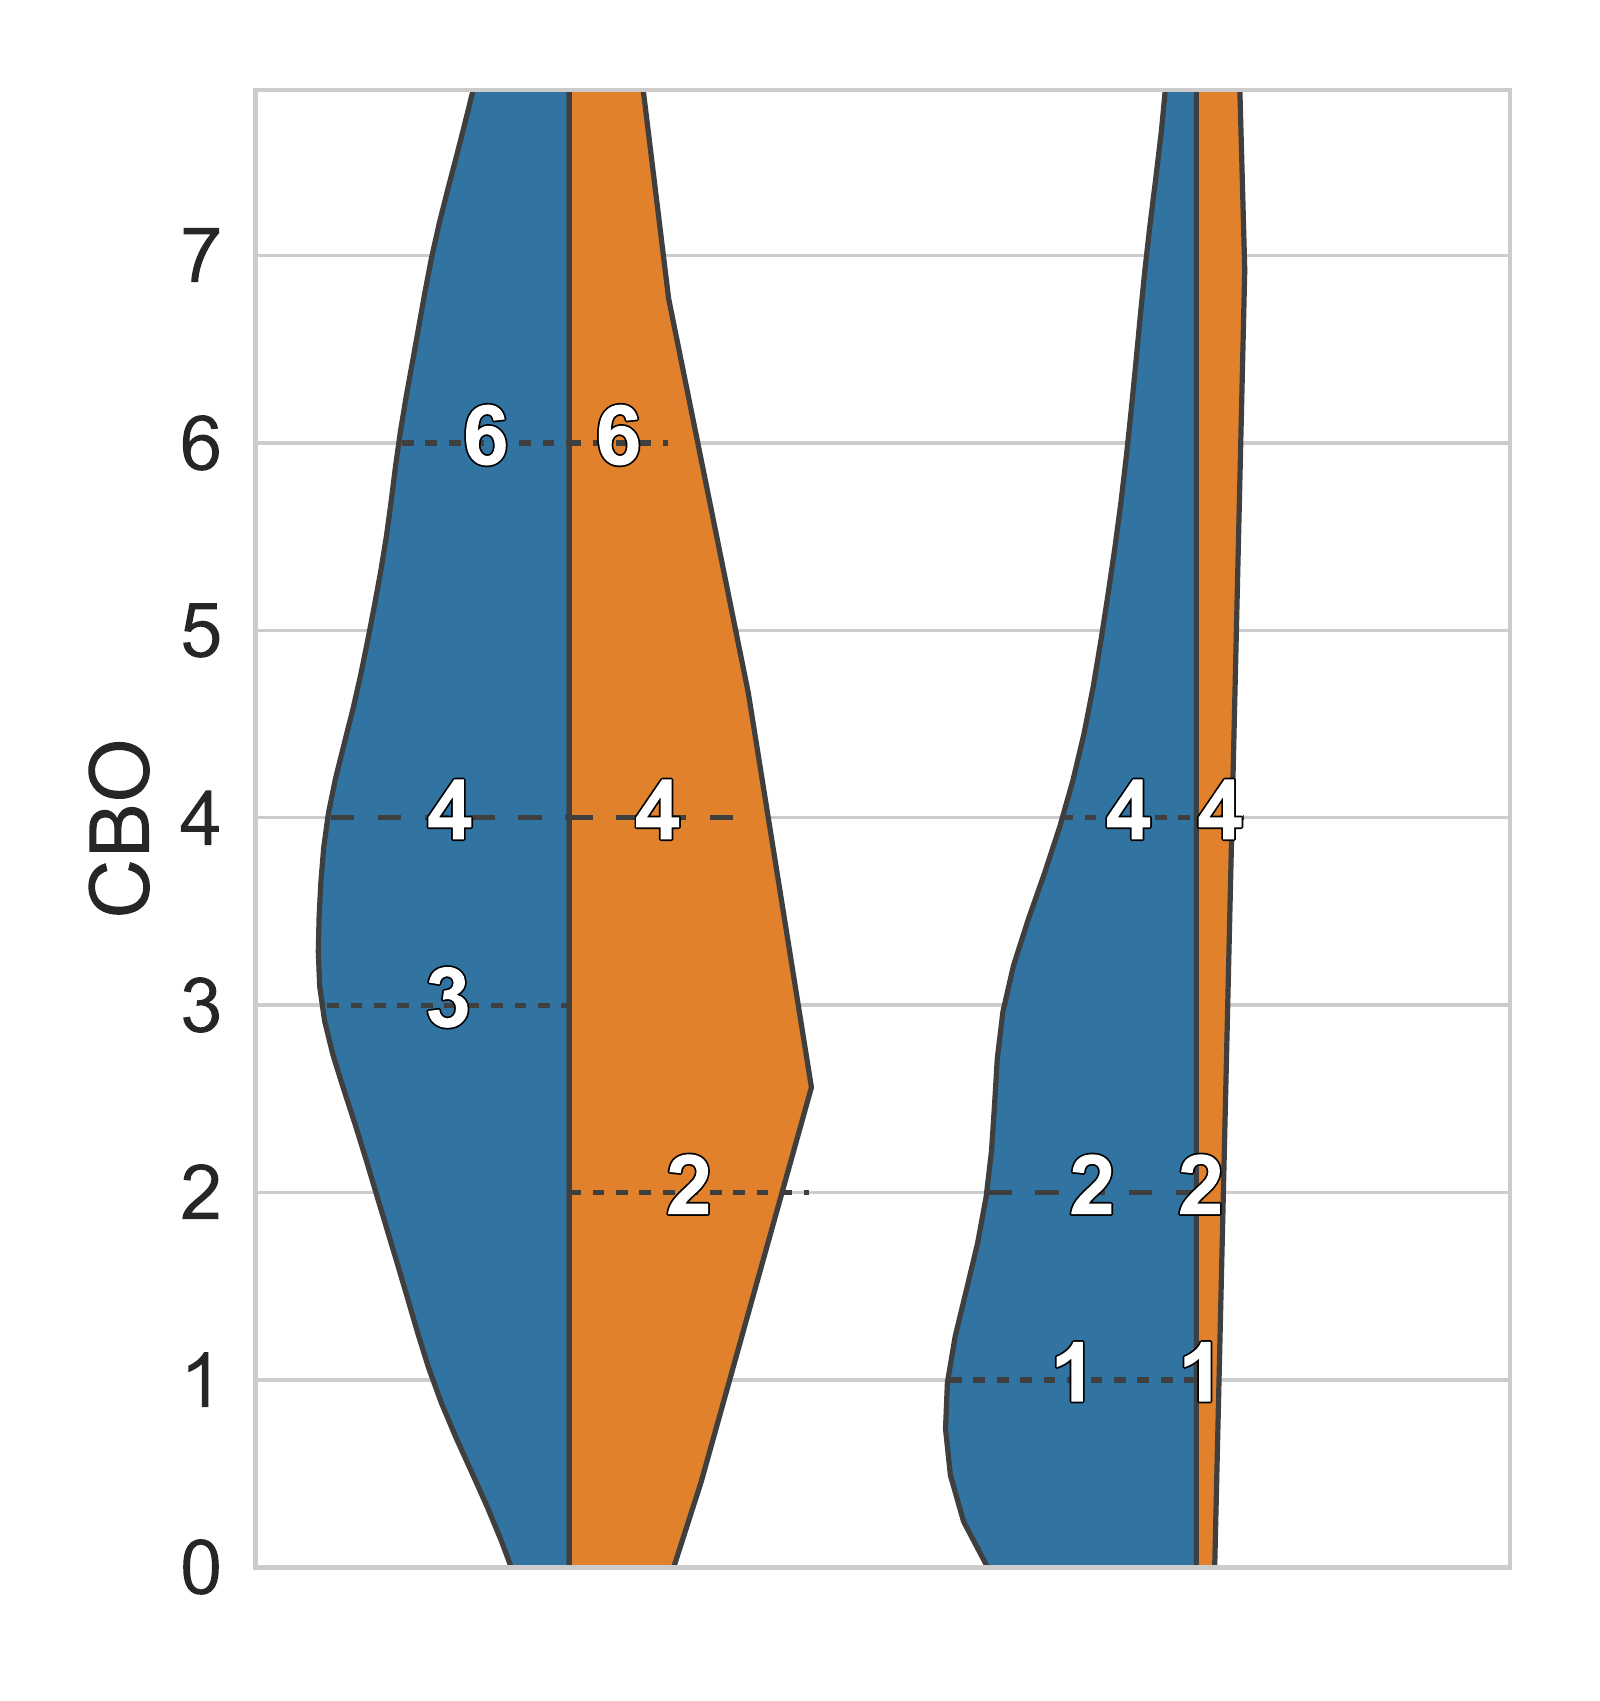}
        \caption{Method-level CBO: The left violin plot indicates methods that underwent an Extract Method refactoring.
            The right violin plot indicates methods that do not need to undergo an Extract Method refactoring.}
    \end{subfigure}
    \caption{CBO distributions for open-source and ING code on both class- and method-level.}
    %\label{fig:only-violin-plot-loc}
\end{figure*}

\begin{figure*}
    \begin{subfigure}[htbp]{0.45\linewidth}
        \centering
        \includegraphics[width=0.65\textwidth]{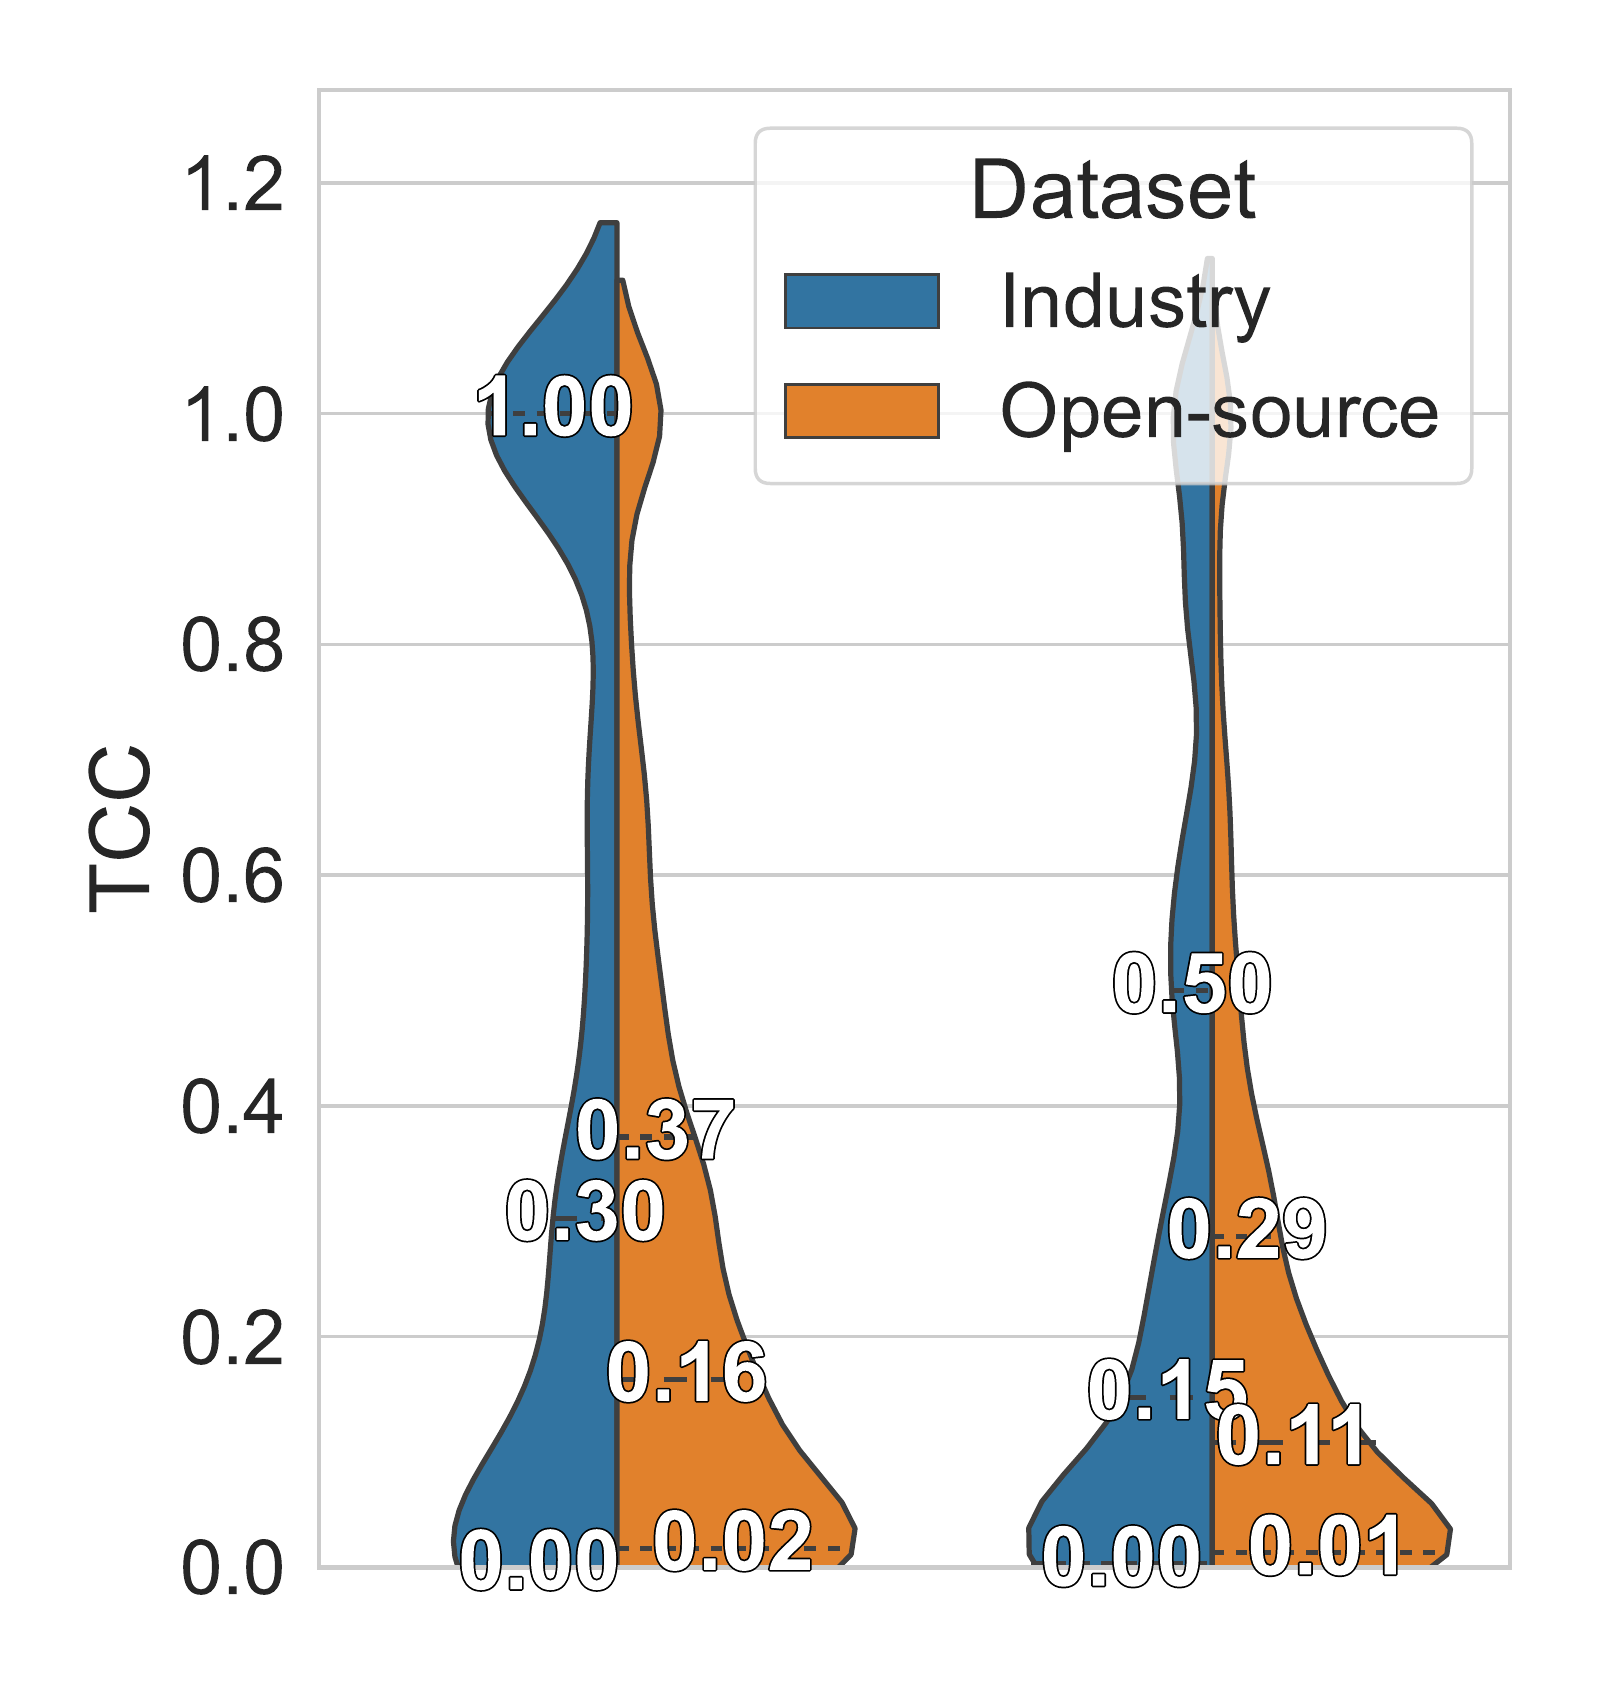}
        \caption{Class-level TCC: The left violin plot indicates classes that contain methods that underwent an Extract Method refactoring.
            The right violin plot indicates classes that do not need to undergo an Extract Method refactoring.}
    \end{subfigure}
    \hfill
    \begin{subfigure}[htbp]{0.45\linewidth}
        \centering
        \includegraphics[width=0.65\textwidth]{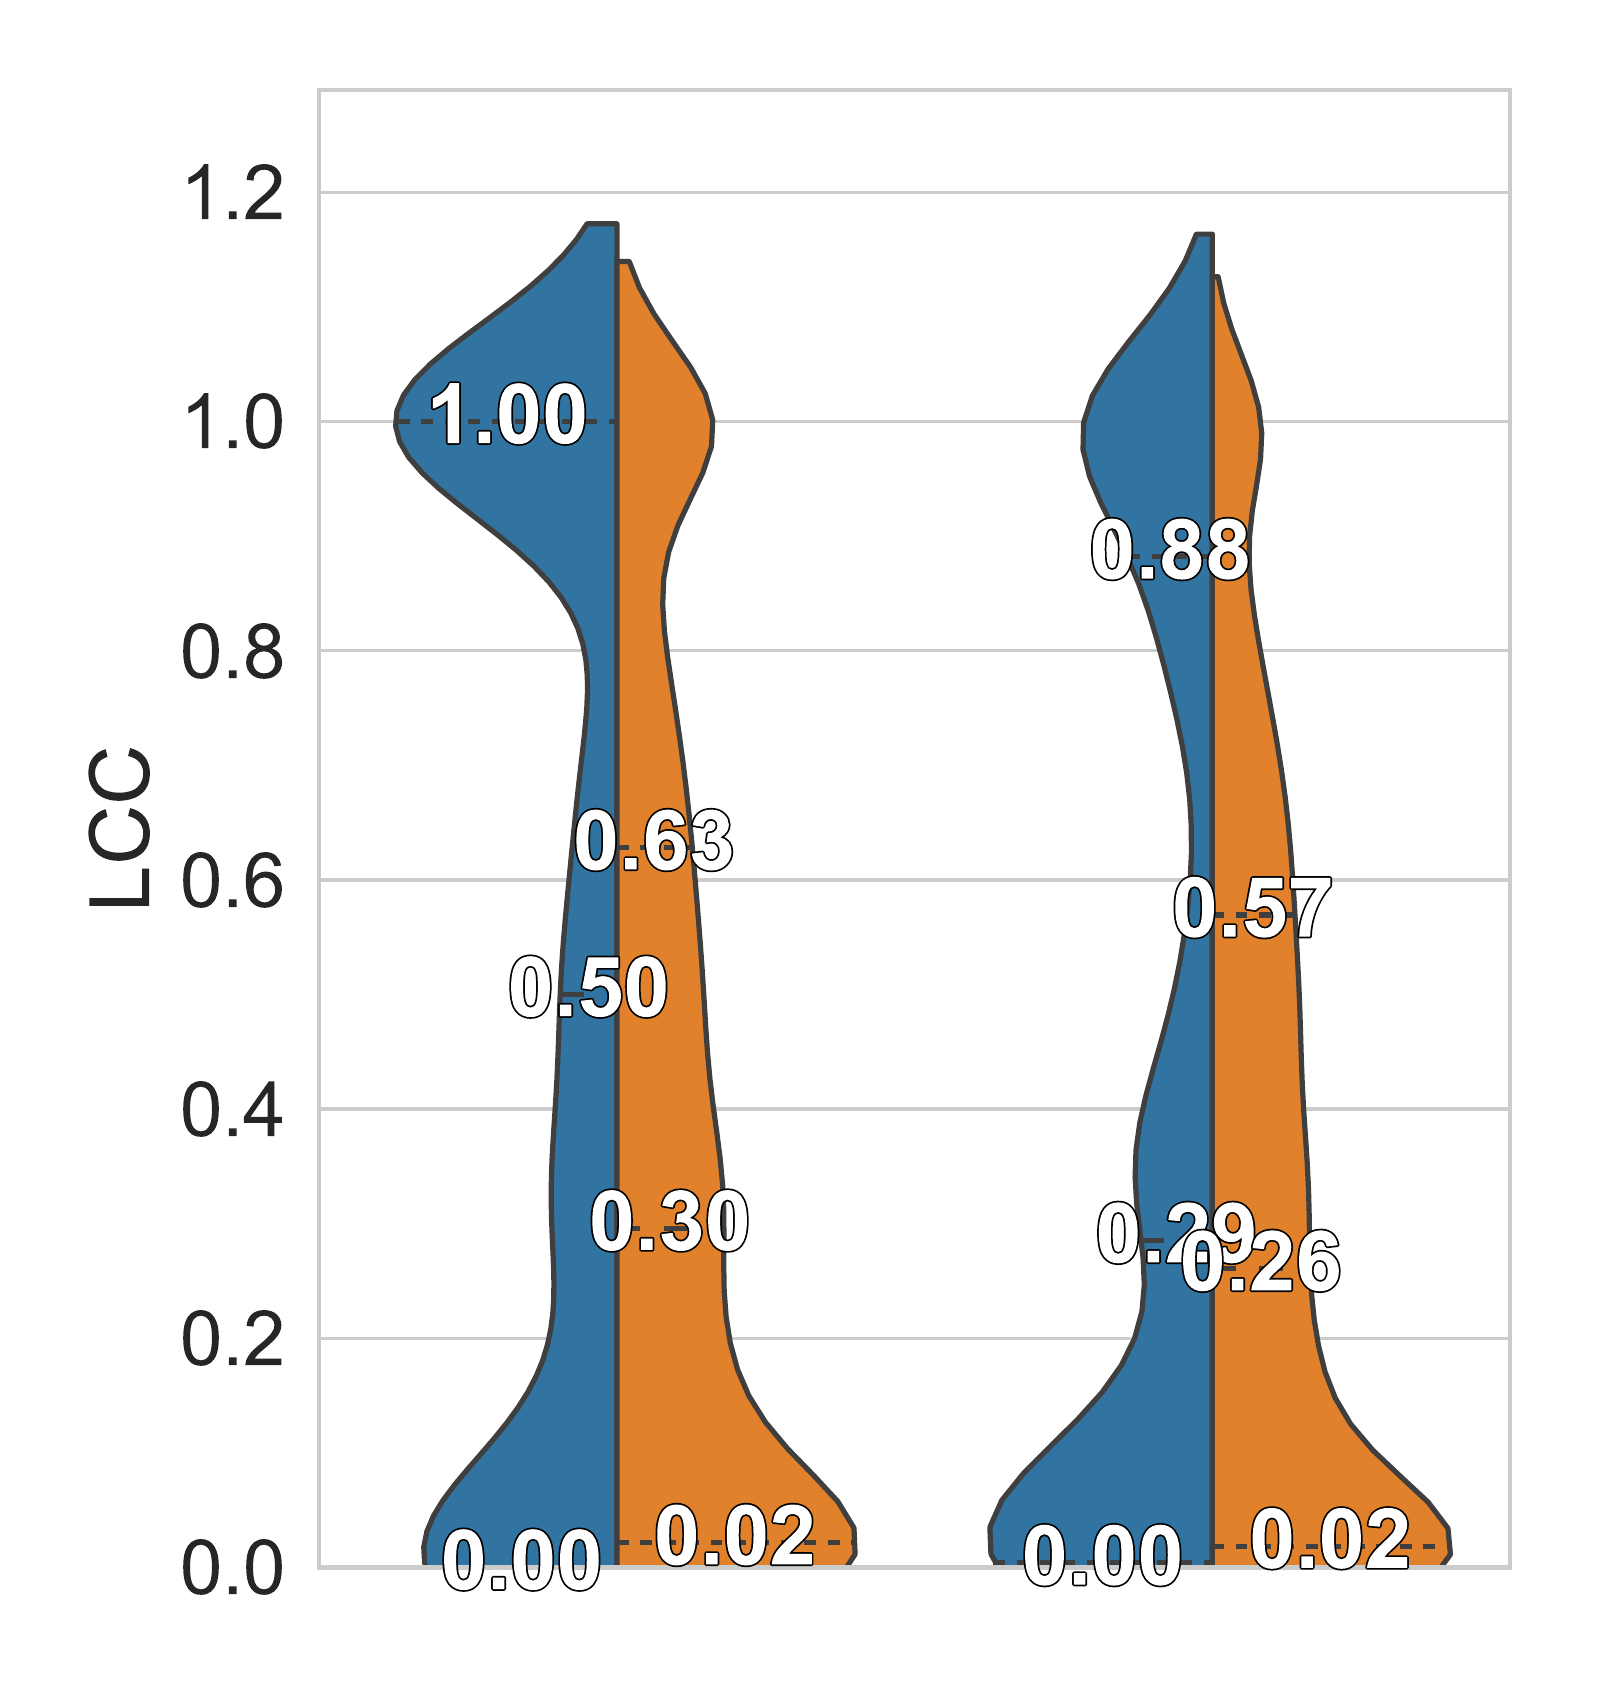}
        \caption{Class-level LCC: The left violin plot indicates classes that contain methods that underwent an Extract Method refactoring.
            The right violin plot indicates classes that do not need to undergo an Extract Method refactoring.}
    \end{subfigure}
    \caption{TCC and LCC distributions for open-source and ING code on class-level.}
    %\label{fig:only-violin-plot-loc}
\end{figure*}
% \FloatBarrier{}
% \subsection{Per project}
\begin{figure}[hbpt]
    \centering
     \begin{subfigure}[htbp]{0.30\textwidth}
        \includegraphics[width=\textwidth]{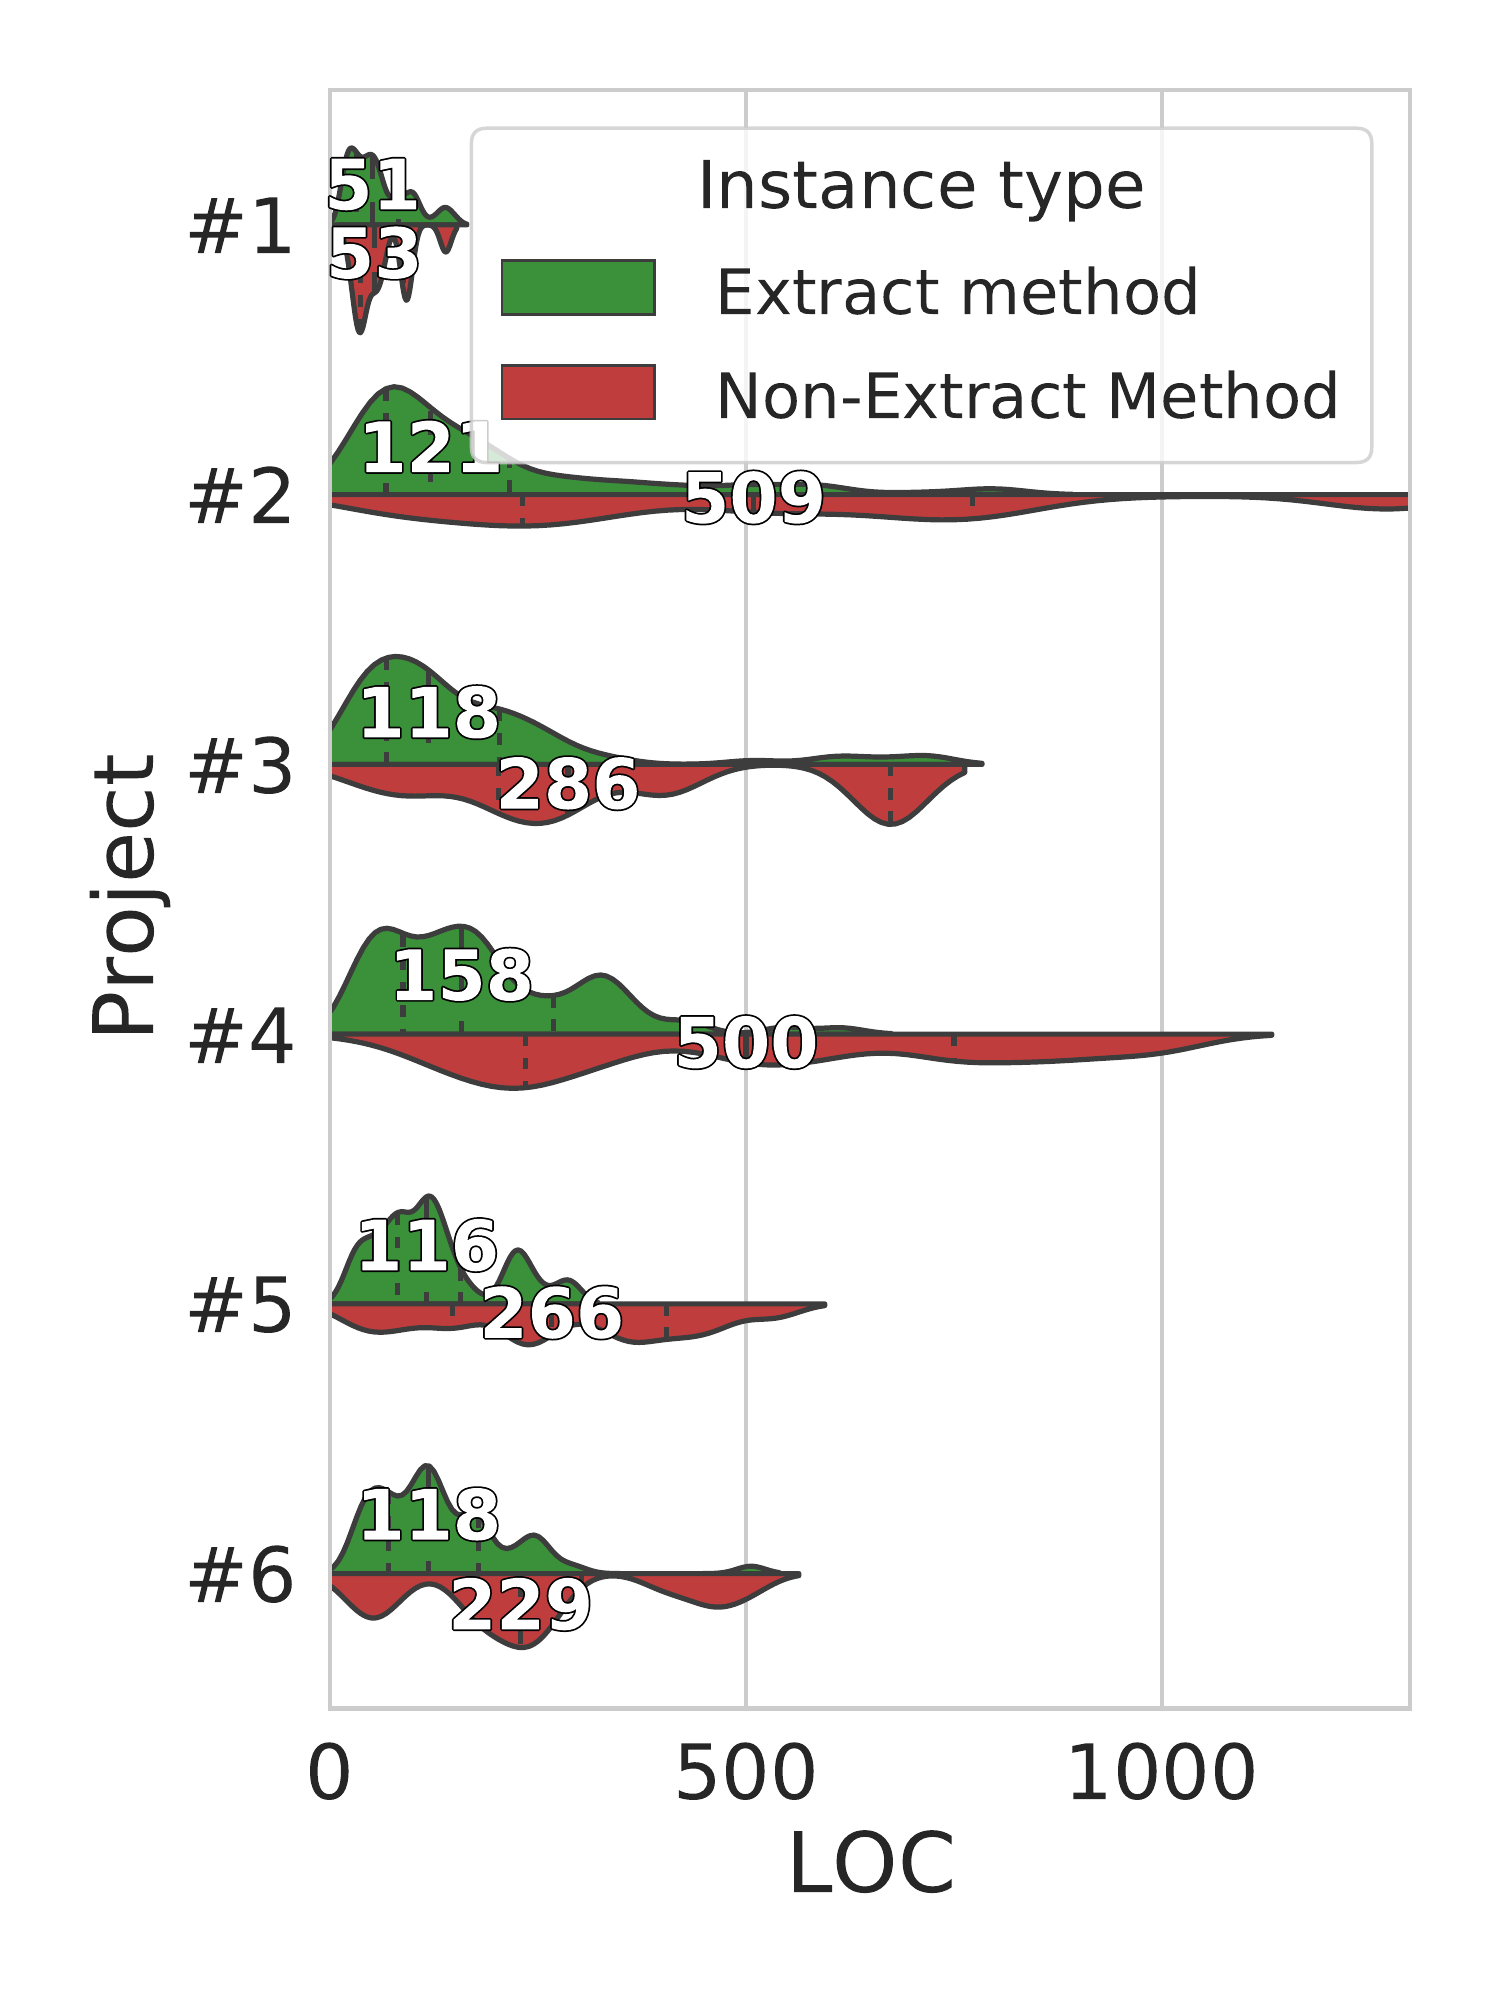}
        \caption{Class-level LOC: The top violin plot indicates classes that contain methods that underwent an Extract Method refactoring.
            The bottom violin plot indicates classes that do not need to undergo an Extract Method refactoring.}\label{fig:app-per-project-classloc}
    \end{subfigure}
        \hfill{}
        \begin{subfigure}[htbp]{0.30\textwidth}
        \includegraphics[width=\textwidth]{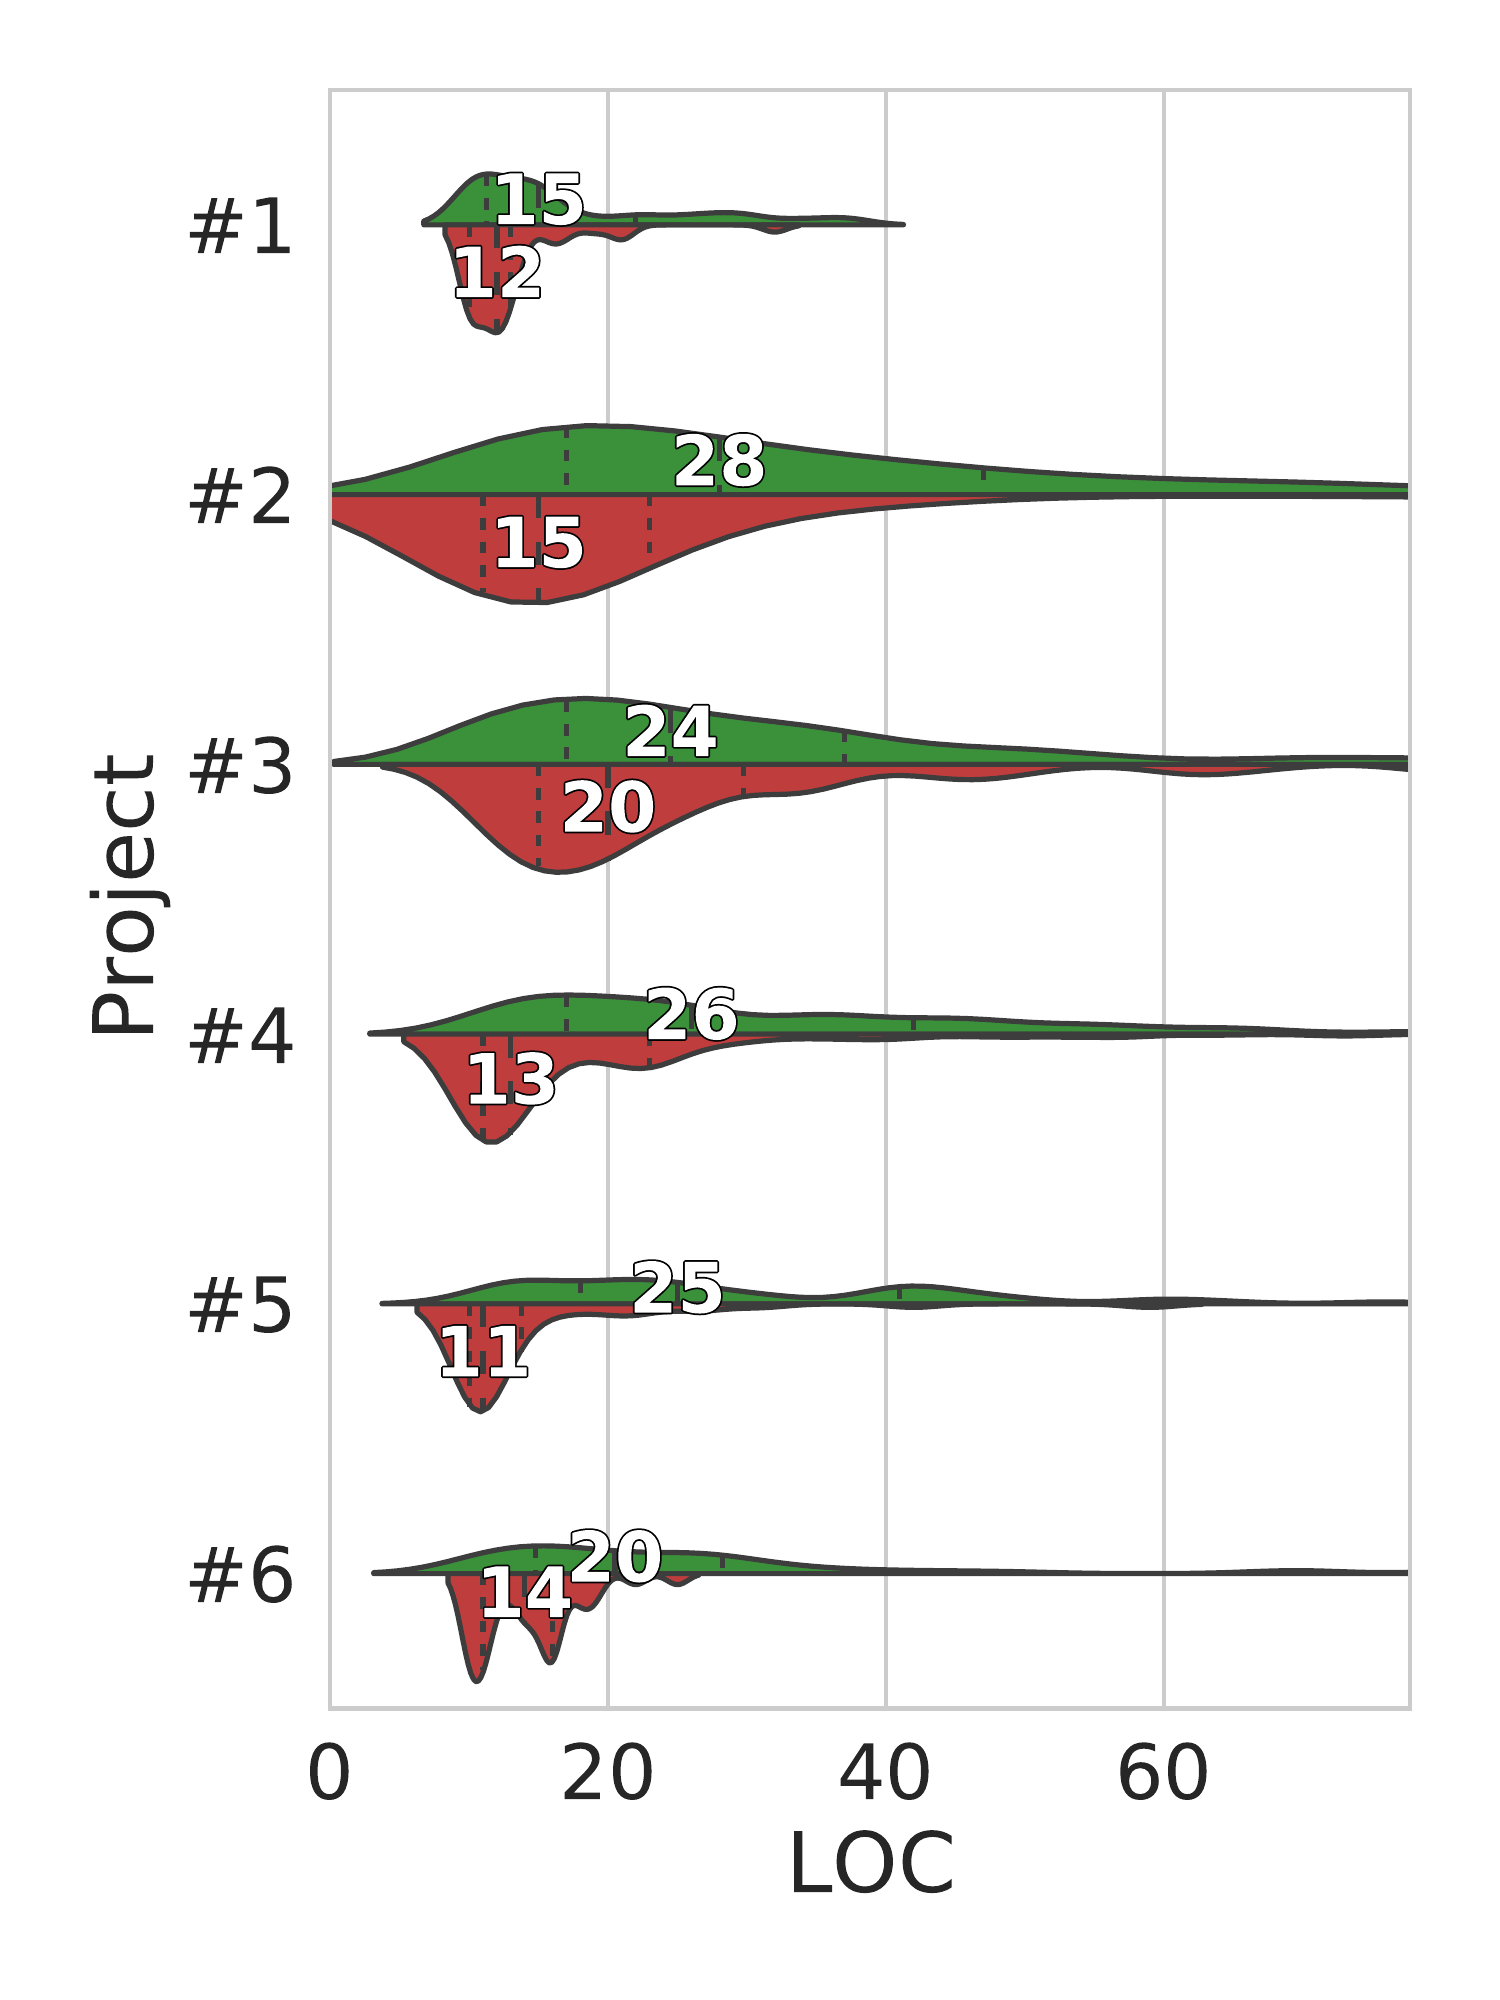}
        \caption{Method-level LOC: The top violin plot indicates methods that underwent an Extract Method refactoring.
            The bottom violin plot indicates methods that do not need to undergo an Extract Method refactoring.}\label{fig:app-per-project-methodloc}
    \end{subfigure}
    \caption{LOC distributions for open-source and ING code on both class- and method-level per project.}
\end{figure}
\begin{figure}[hbpt]
    \centering
    \begin{subfigure}[htbp]{0.35\textwidth}
        \includegraphics[width=\textwidth]{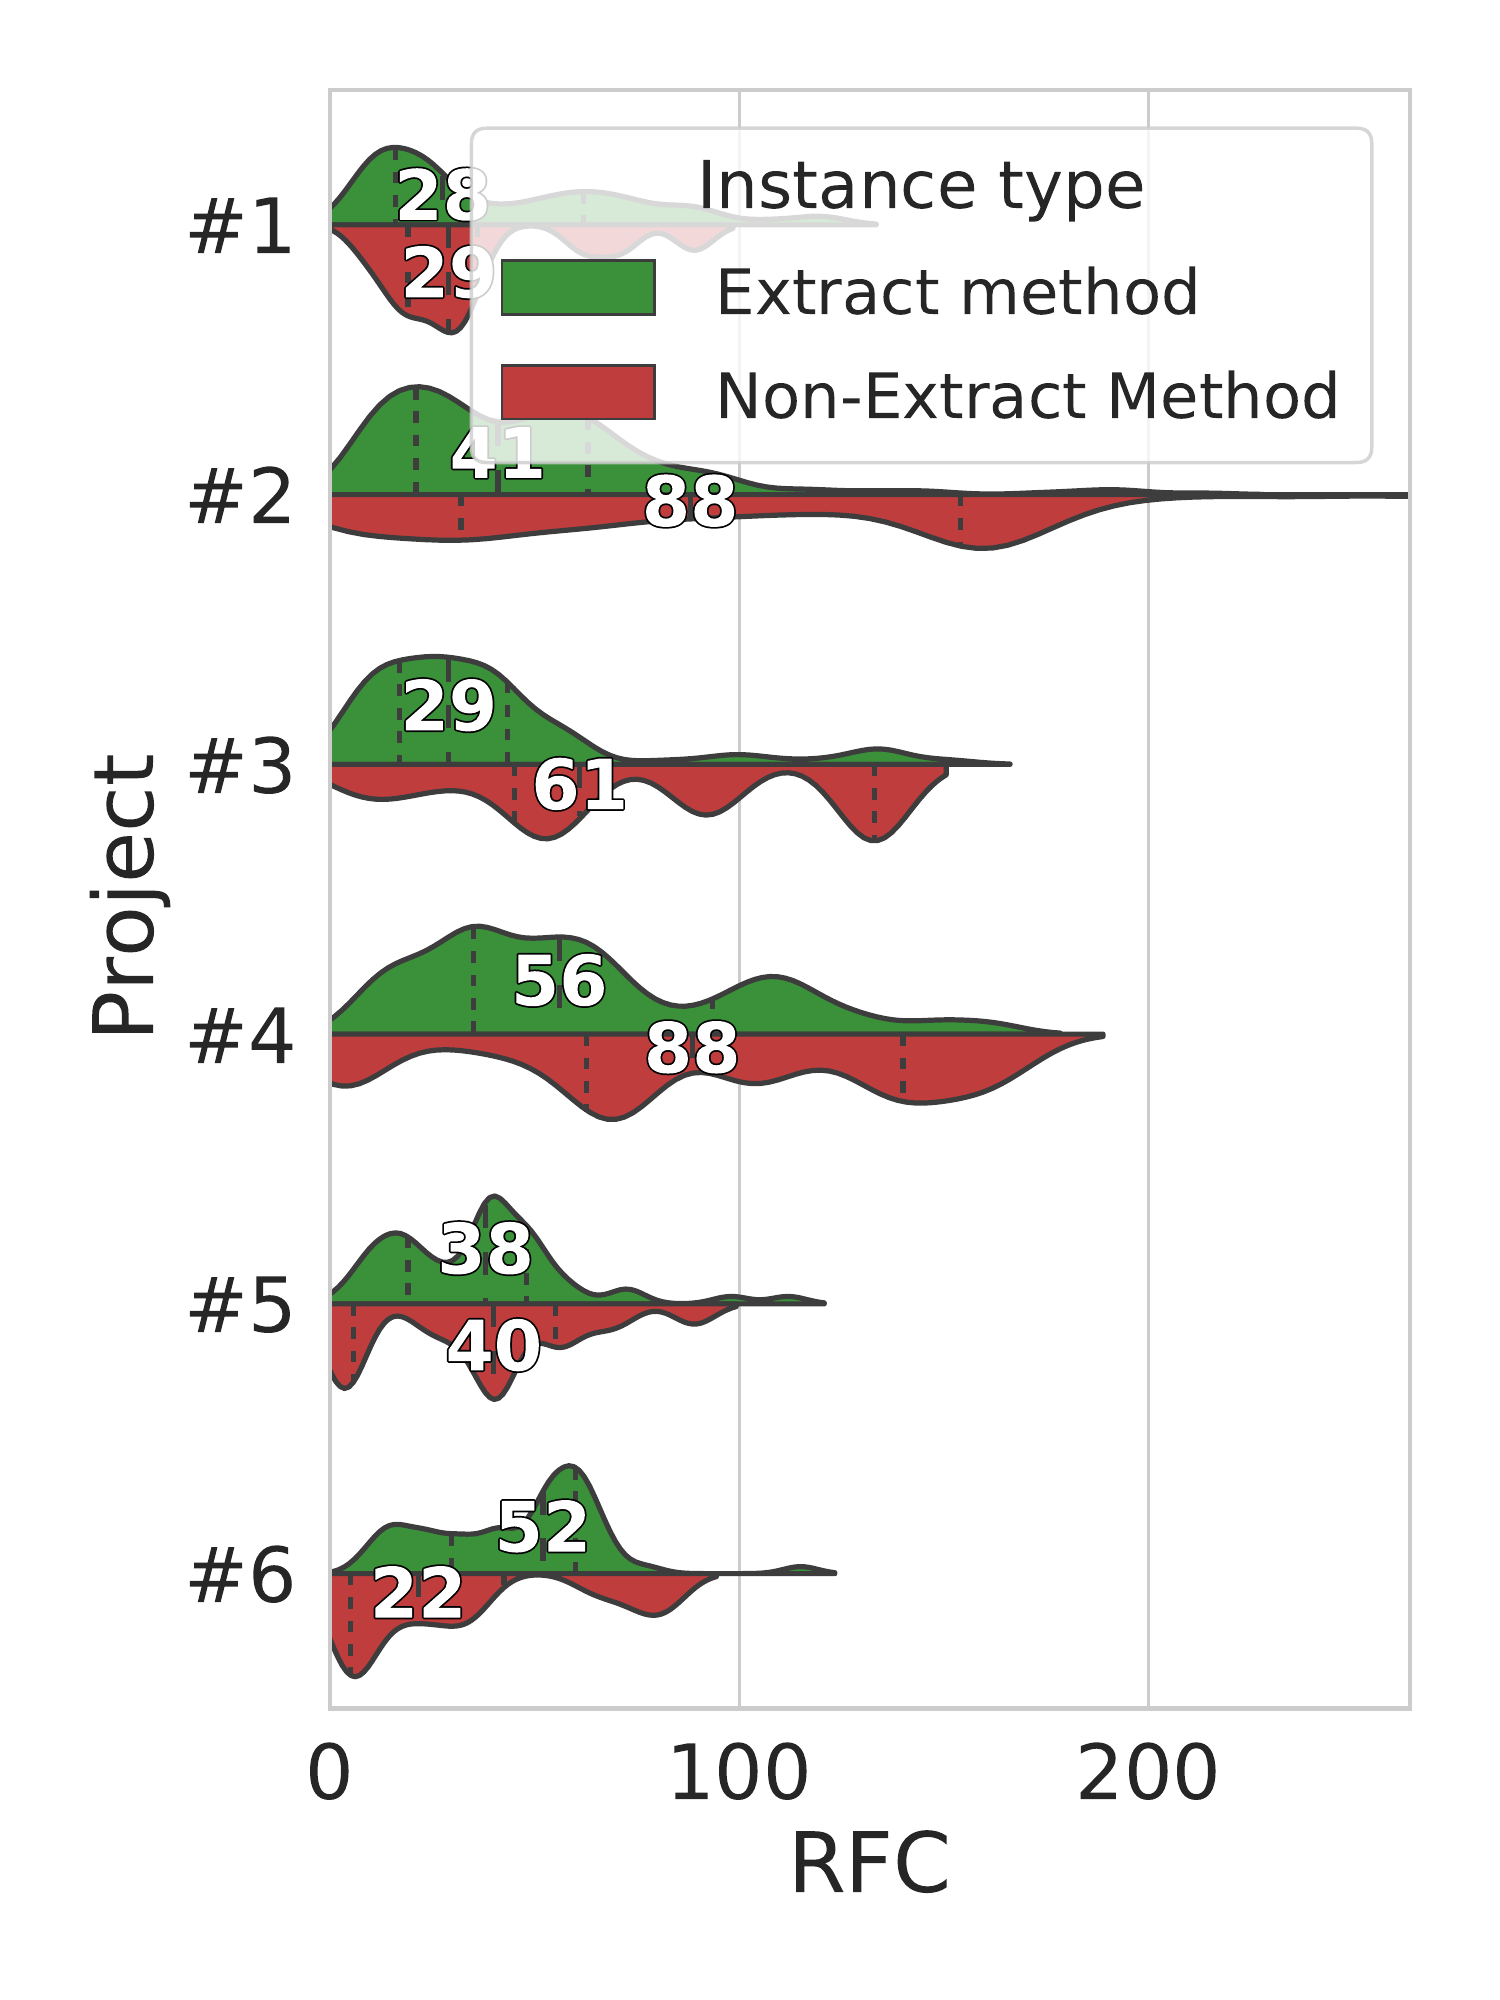}
        \caption{Class-level RFC: The top violin plot indicates classes that contain methods that underwent an Extract Method refactoring.
            The bottom violin plot indicates classes that do not need to undergo an Extract Method refactoring.}\label{fig:app-per-project-classrfc}
    \end{subfigure}
        \hfill{}
         \begin{subfigure}[htbp]{0.35\textwidth}
        \includegraphics[width=\textwidth]{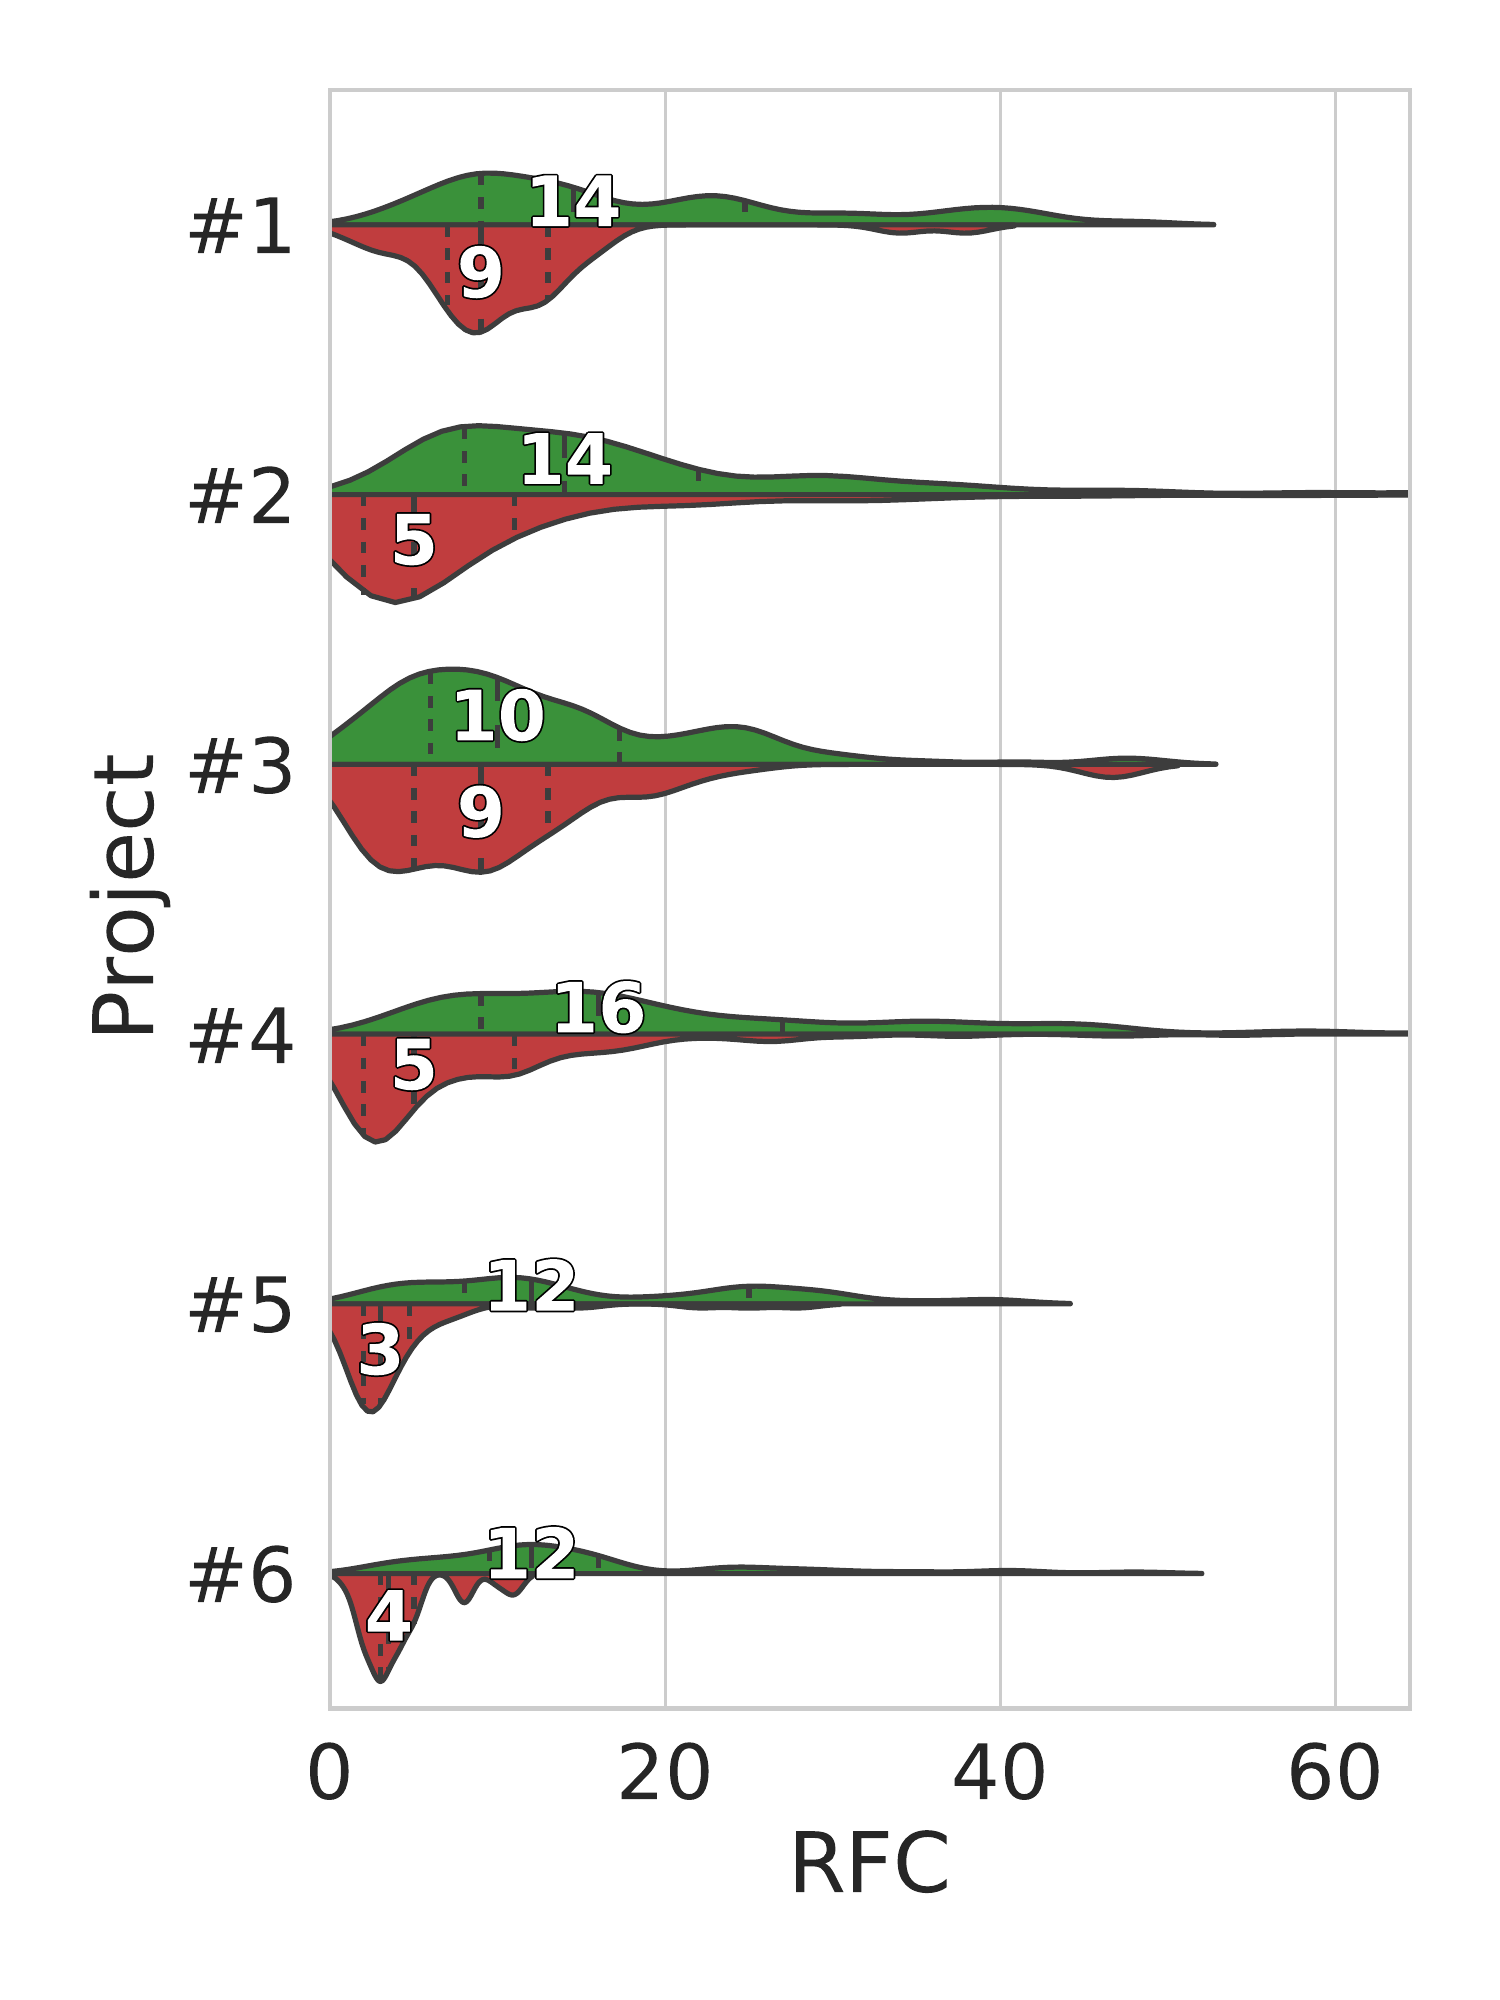}
        \caption{Method-level RFC: The top violin plot indicates methods that underwent an Extract Method refactoring.
            The bottom violin plot indicates methods that do not need to undergo an Extract Method refactoring.}\label{fig:app-per-project-methodrfc}
    \end{subfigure}
    \caption{RFC distributions for open-source and ING code on both class- and method-level per project.}
\end{figure}

\begin{figure}[hbpt]
    \centering
        \begin{subfigure}[htbp]{0.35\textwidth}
        \includegraphics[width=\textwidth]{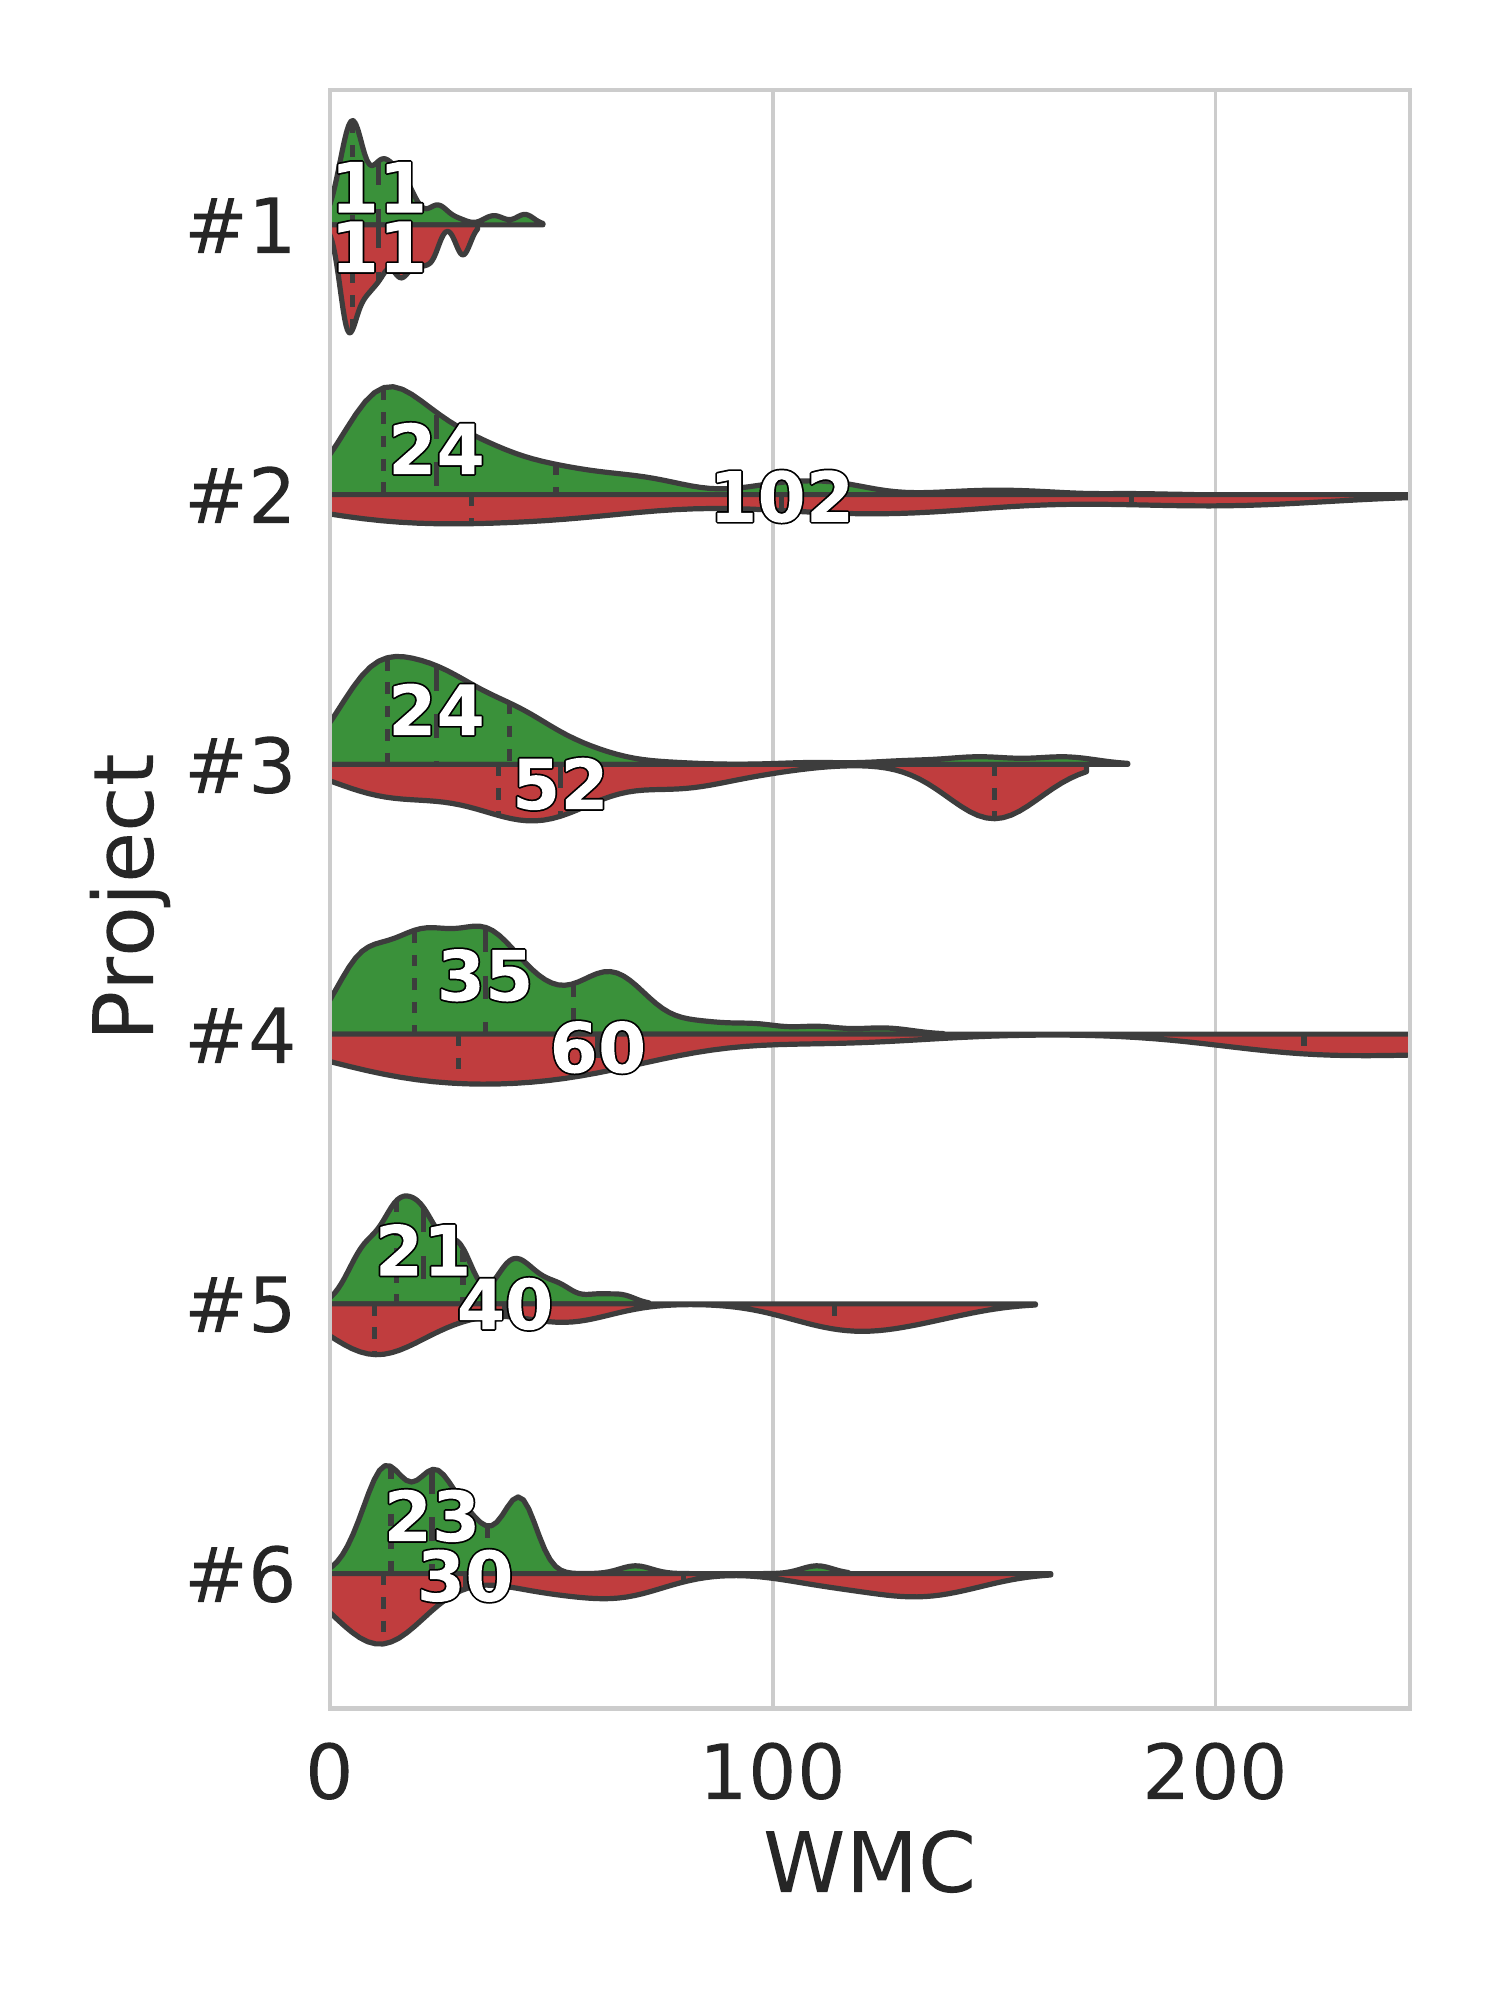}
        \caption{Class-level WMC: The top violin plot indicates classes that contain methods that underwent an Extract Method refactoring.
            The bottom violin plot indicates classes that do not need to undergo an Extract Method refactoring.}\label{fig:app-per-project-classwmc}
    \end{subfigure}
        \hfill{}
        \begin{subfigure}[htbp]{0.35\textwidth}
        \includegraphics[width=\textwidth]{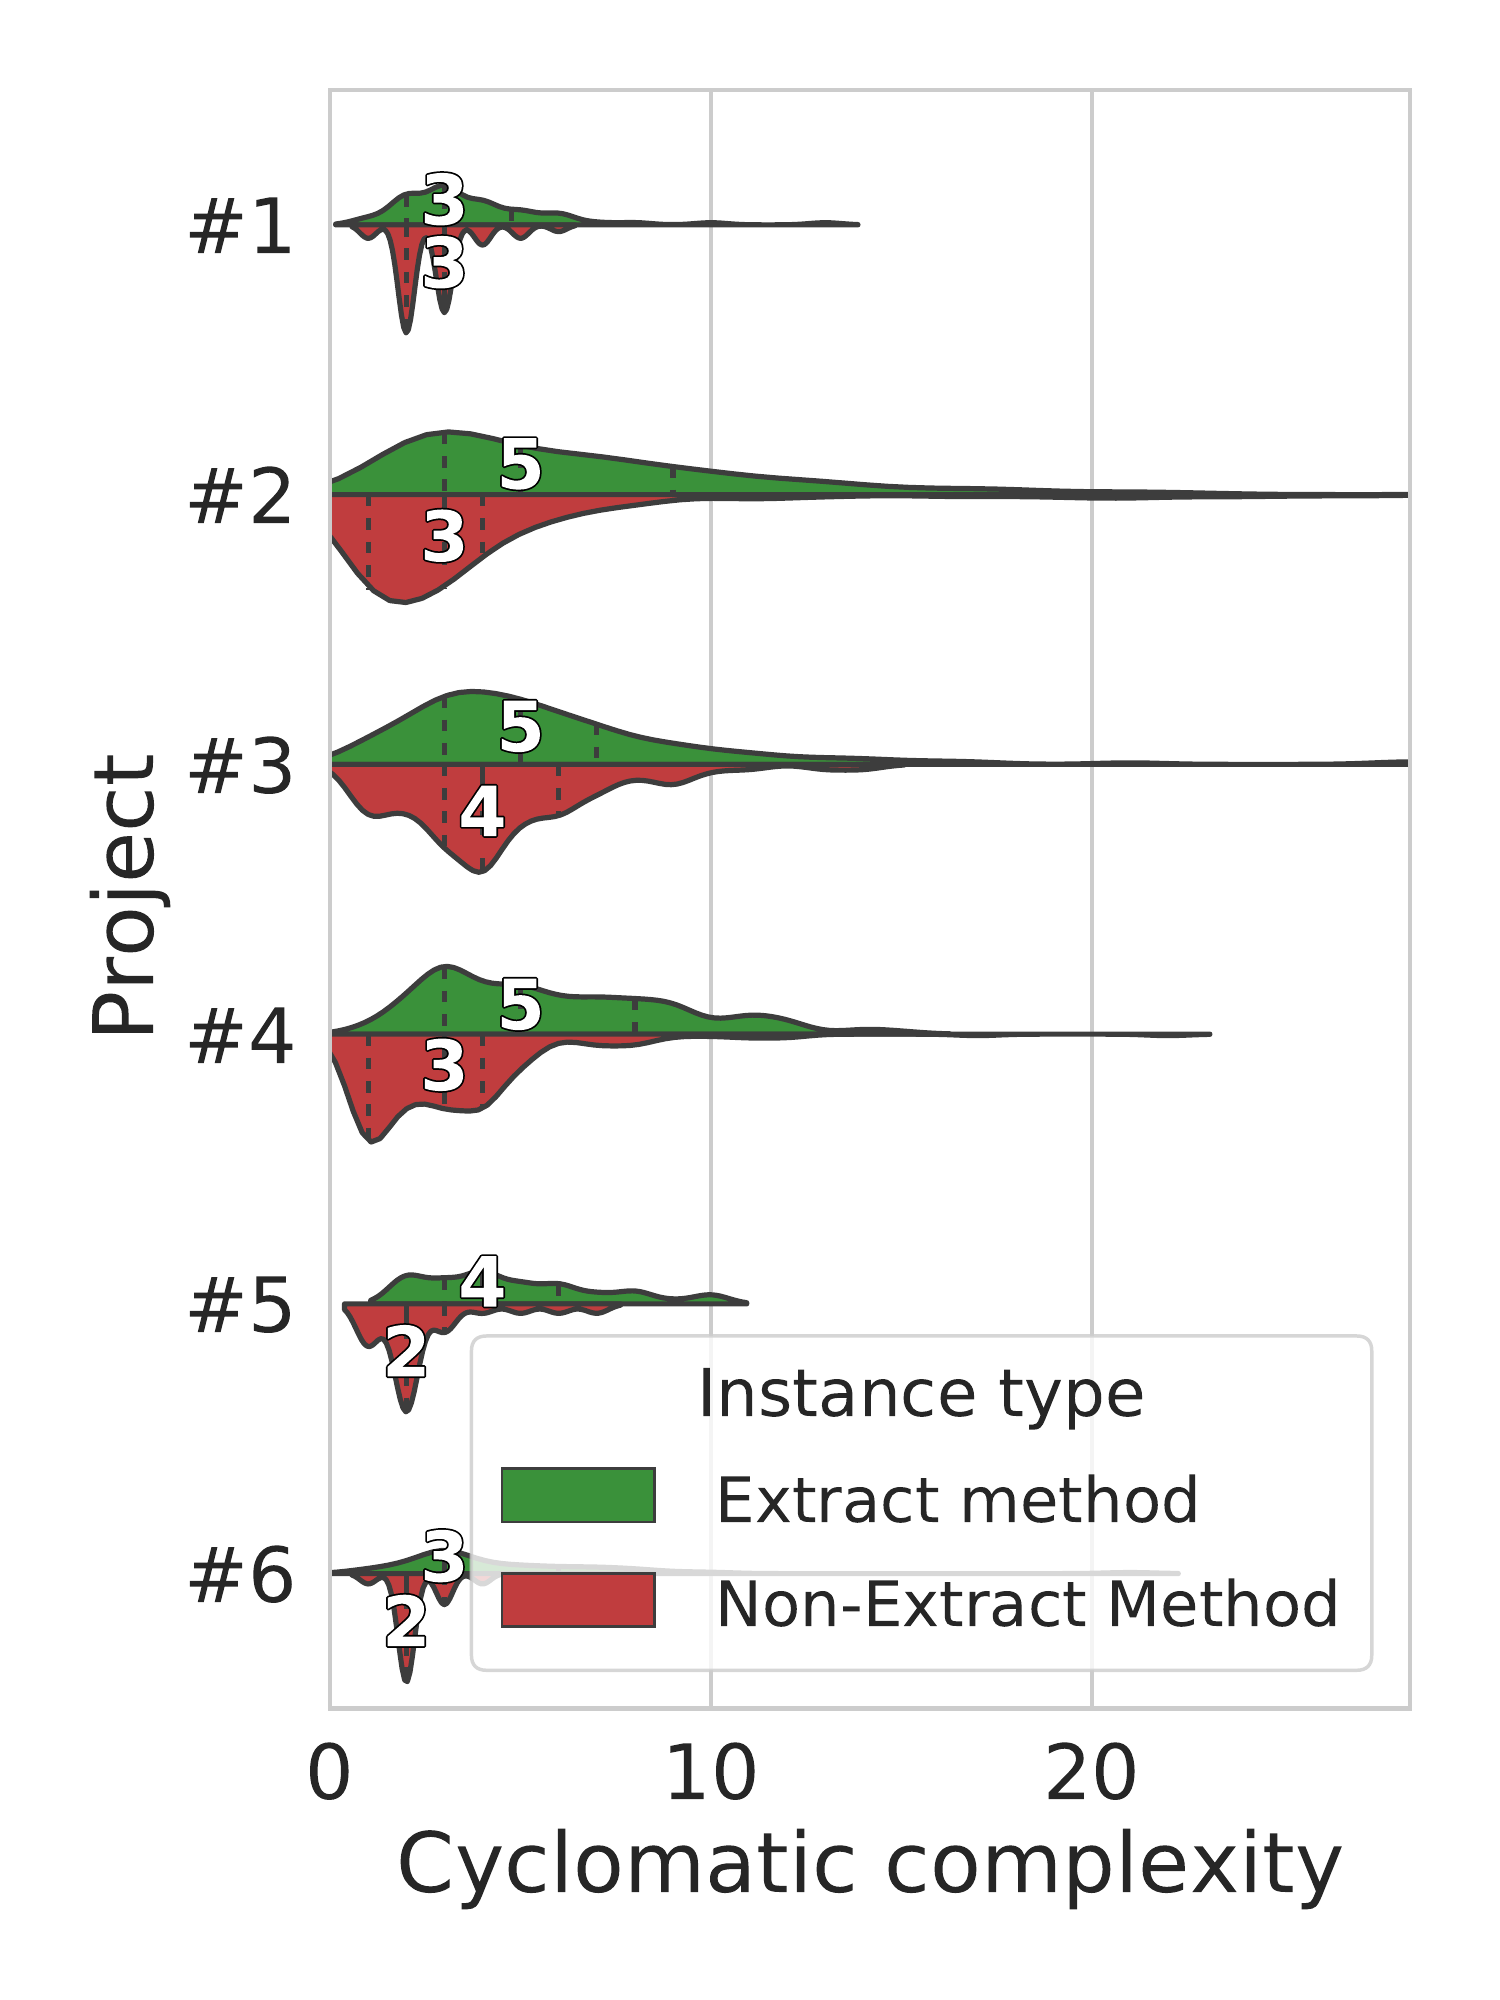}
        \caption{Method-level cyclomatic complexity: The top violin plot indicates methods that underwent an Extract Method refactoring.
            The bottom violin plot indicates methods that do not need to undergo an Extract Method refactoring.}\label{fig:app-per-project-methodwmc}
    \end{subfigure}

    \caption{WMC and cyclomatic complexity distributions for open-source and ING code on both class- and method-level per project.}
\end{figure}

\begin{figure}
    \centering
            \begin{subfigure}[htbp]{0.35\textwidth}
        \includegraphics[width=\textwidth]{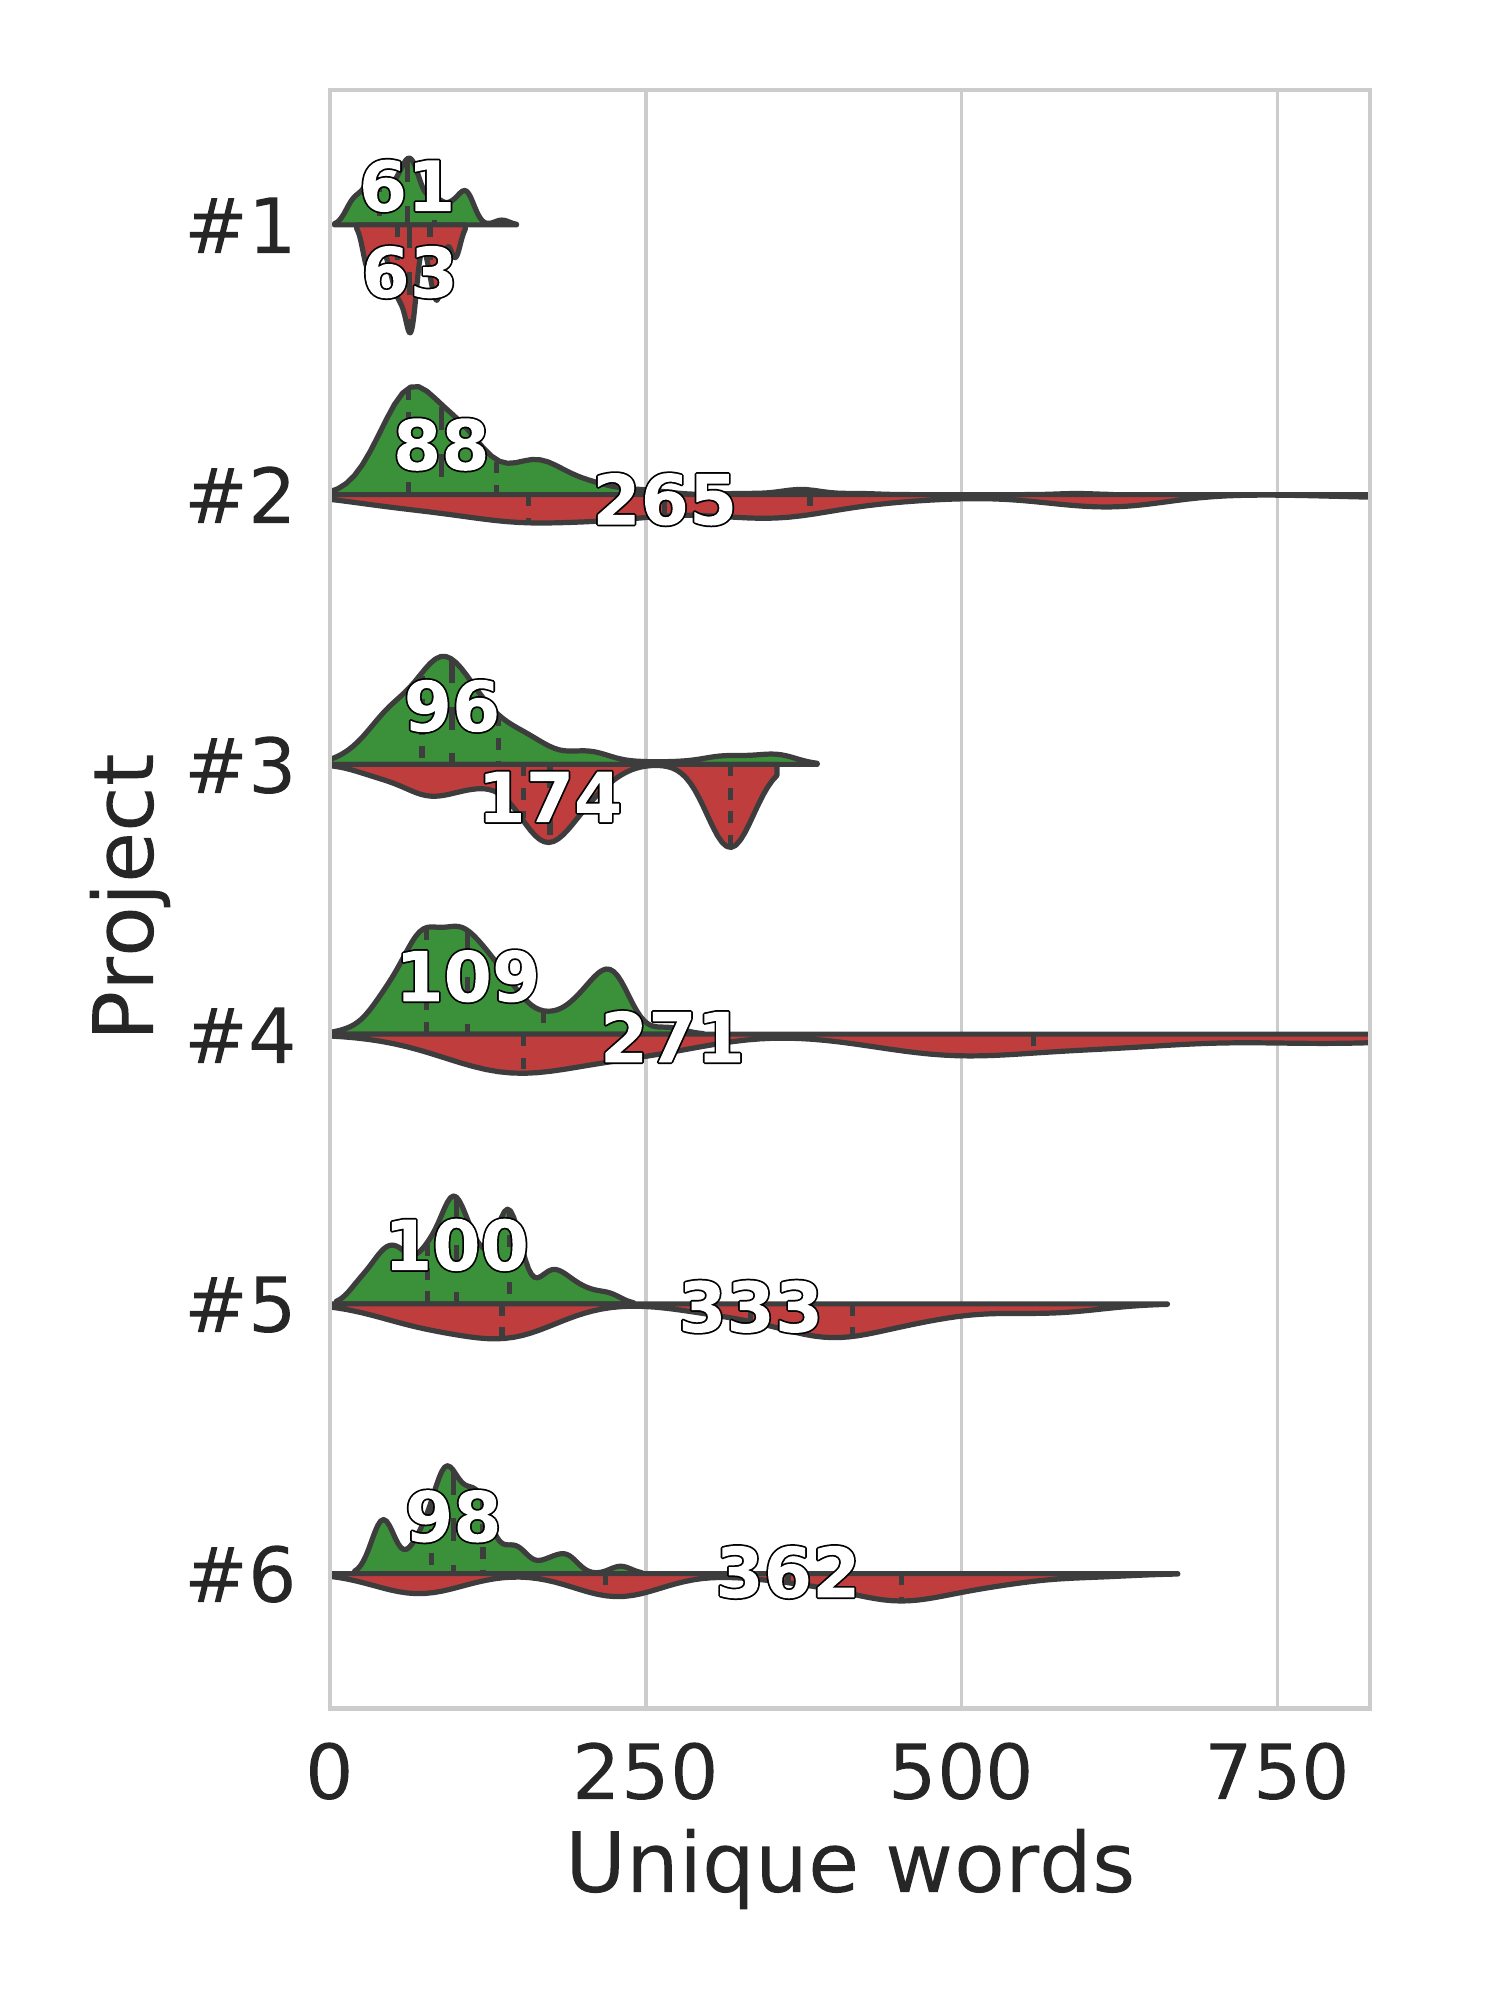}
        \caption{Class-level UniqueWordsQty: The top violin plot indicates classes that contain methods that underwent an Extract Method refactoring.
            The bottom violin plot indicates classes that do not need to undergo an Extract Method refactoring.}\label{fig:app-per-project-classuw}
    \end{subfigure}
    \hfill{}
        \begin{subfigure}[htbp]{0.35\textwidth}
        \includegraphics[width=\textwidth]{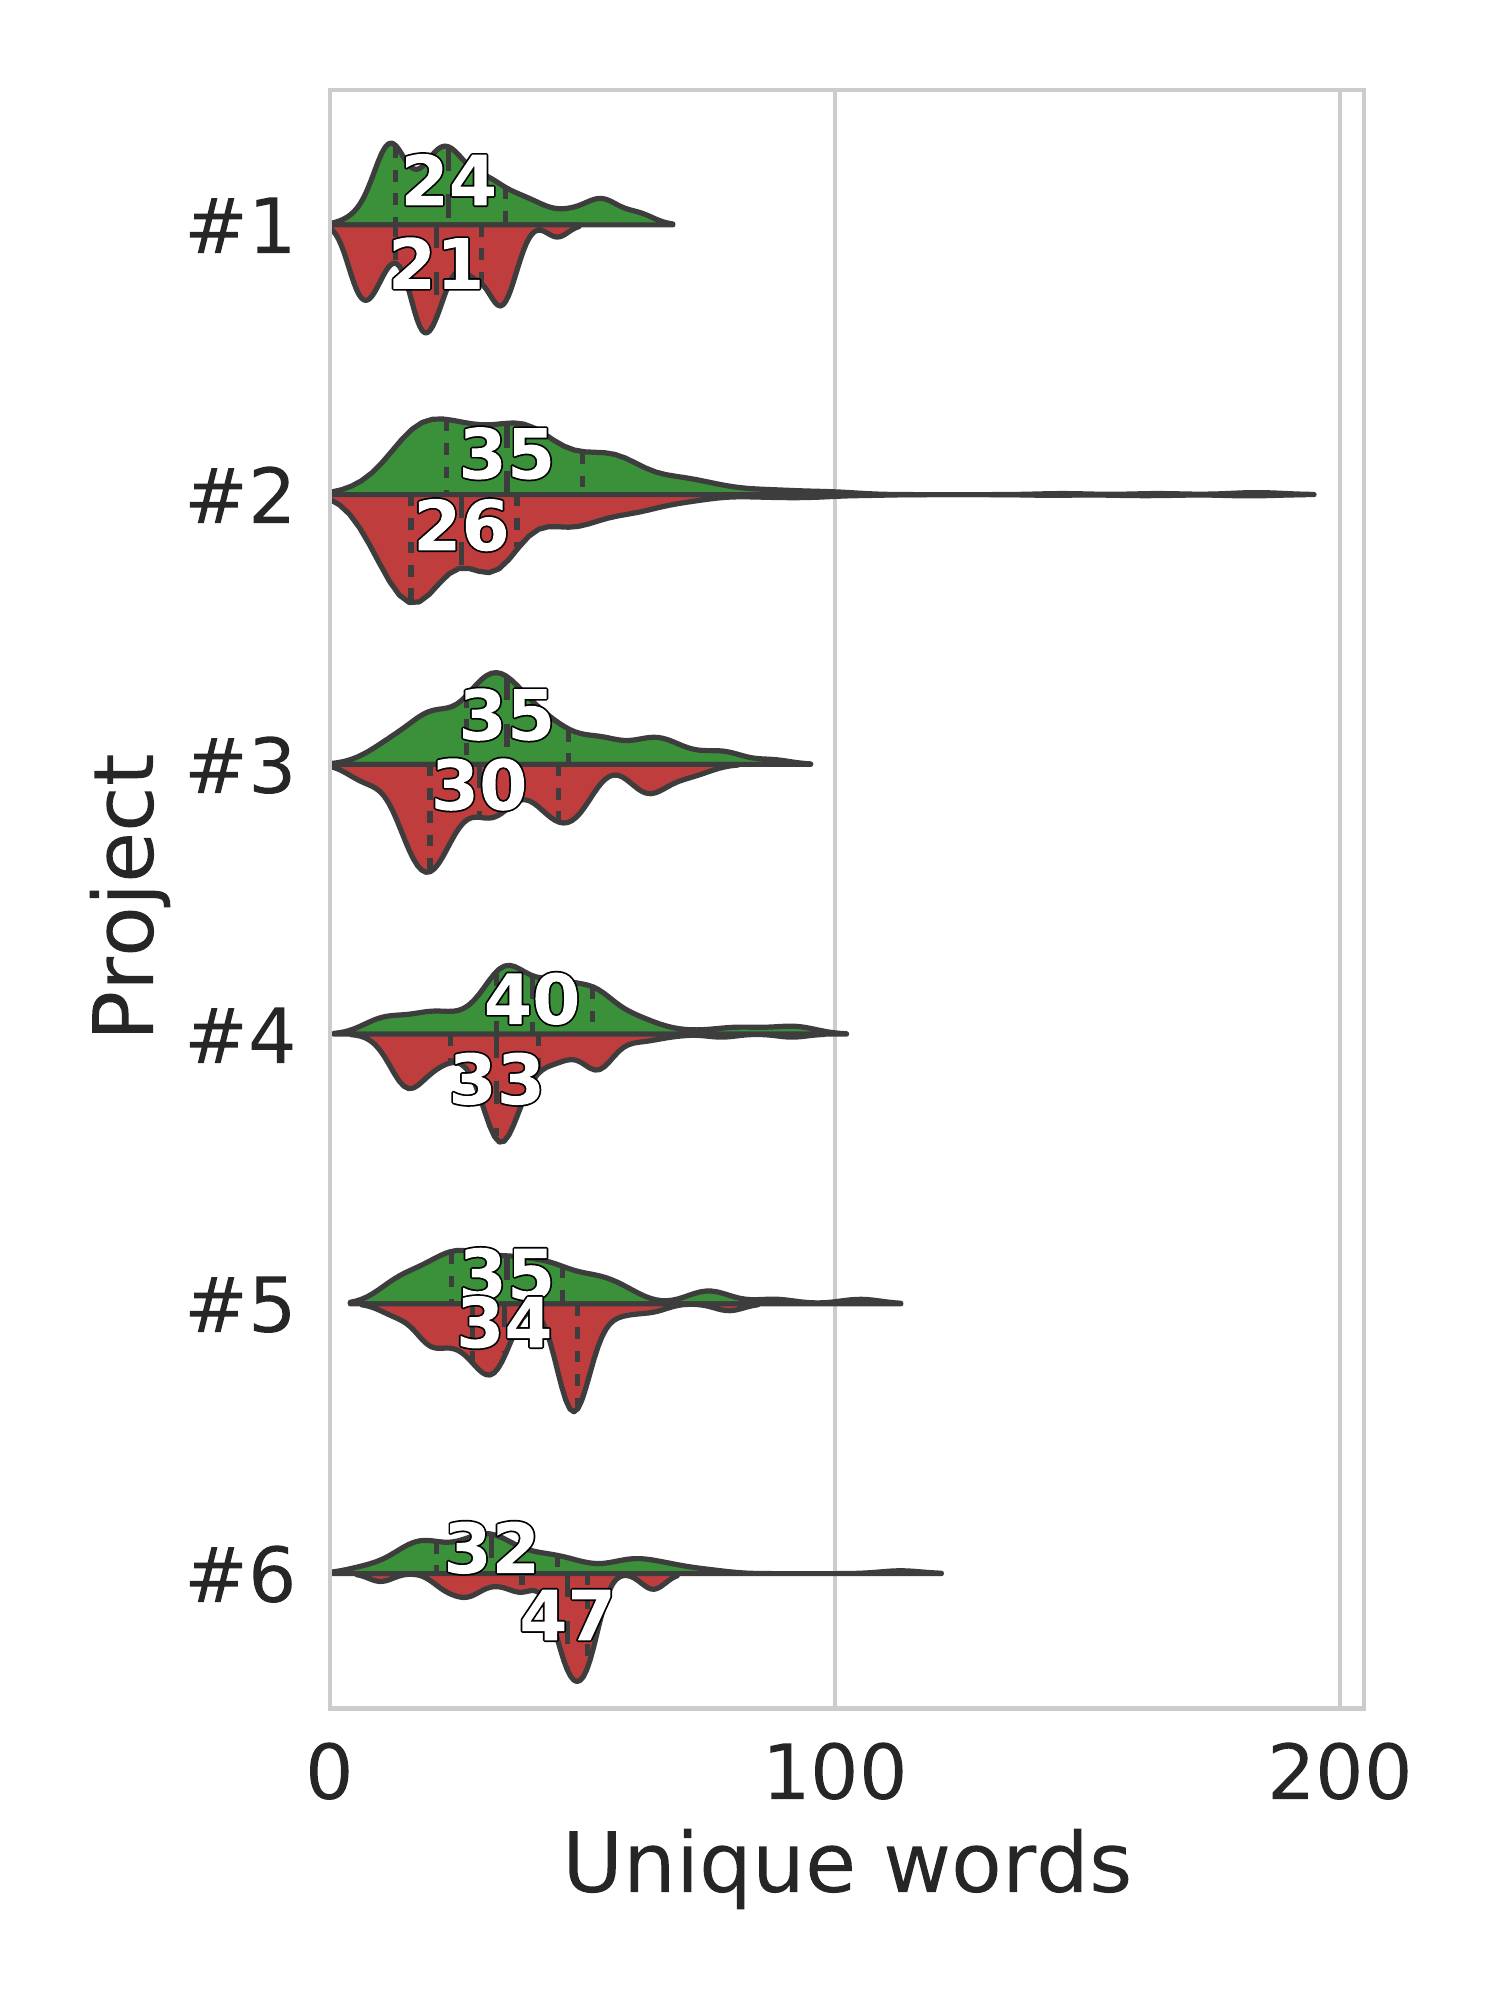}
        \caption{Method-level UniqueWordsQty: The top violin plot indicates methods that underwent an Extract Method refactoring.
            The bottom violin plot indicates methods that do not need to undergo an Extract Method refactoring.}\label{fig:app-per-project-methoduw}
    \end{subfigure}
    \caption{UniqueWordsQty distributions for open-source and ING code on both class- and method-level per project.}
\end{figure}

\begin{figure}[hbpt]
    \centering

       \begin{subfigure}[htbp]{0.35\textwidth}
        \includegraphics[width=\textwidth]{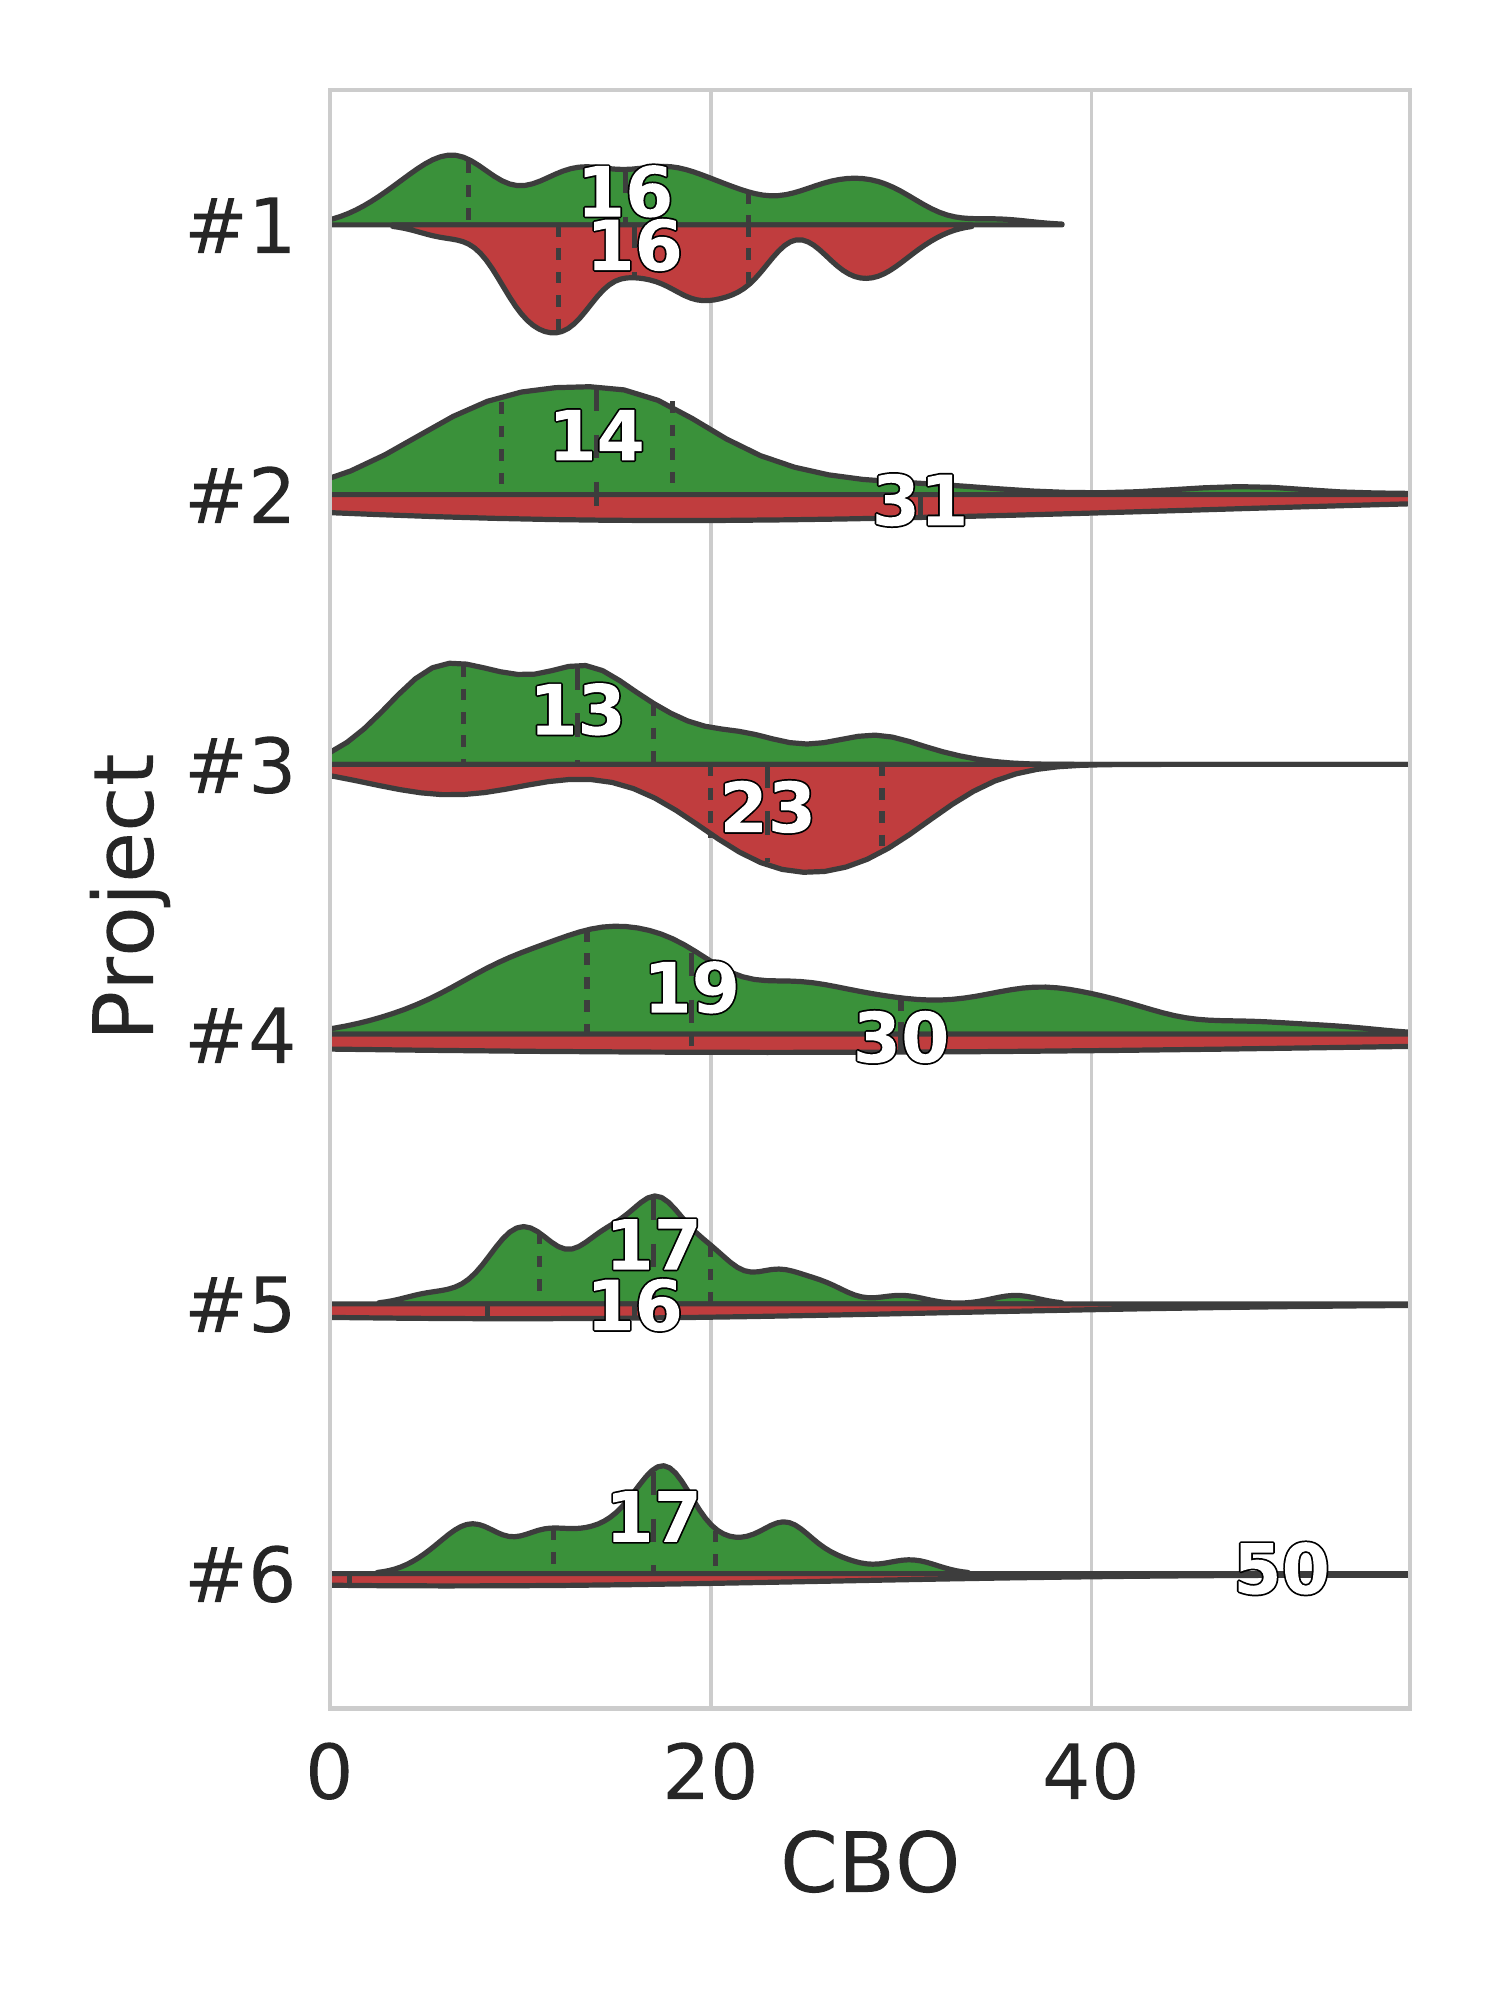}
        \caption{Class-level CBO: The top violin plot indicates classes that contain methods that underwent an Extract Method refactoring.
            The bottom violin plot indicates classes that do not need to undergo an Extract Method refactoring.}\label{fig:app-per-project-classcbo}
    \end{subfigure}
        \hfill{}
        \begin{subfigure}[htbp]{0.35\textwidth}
        \includegraphics[width=\textwidth]{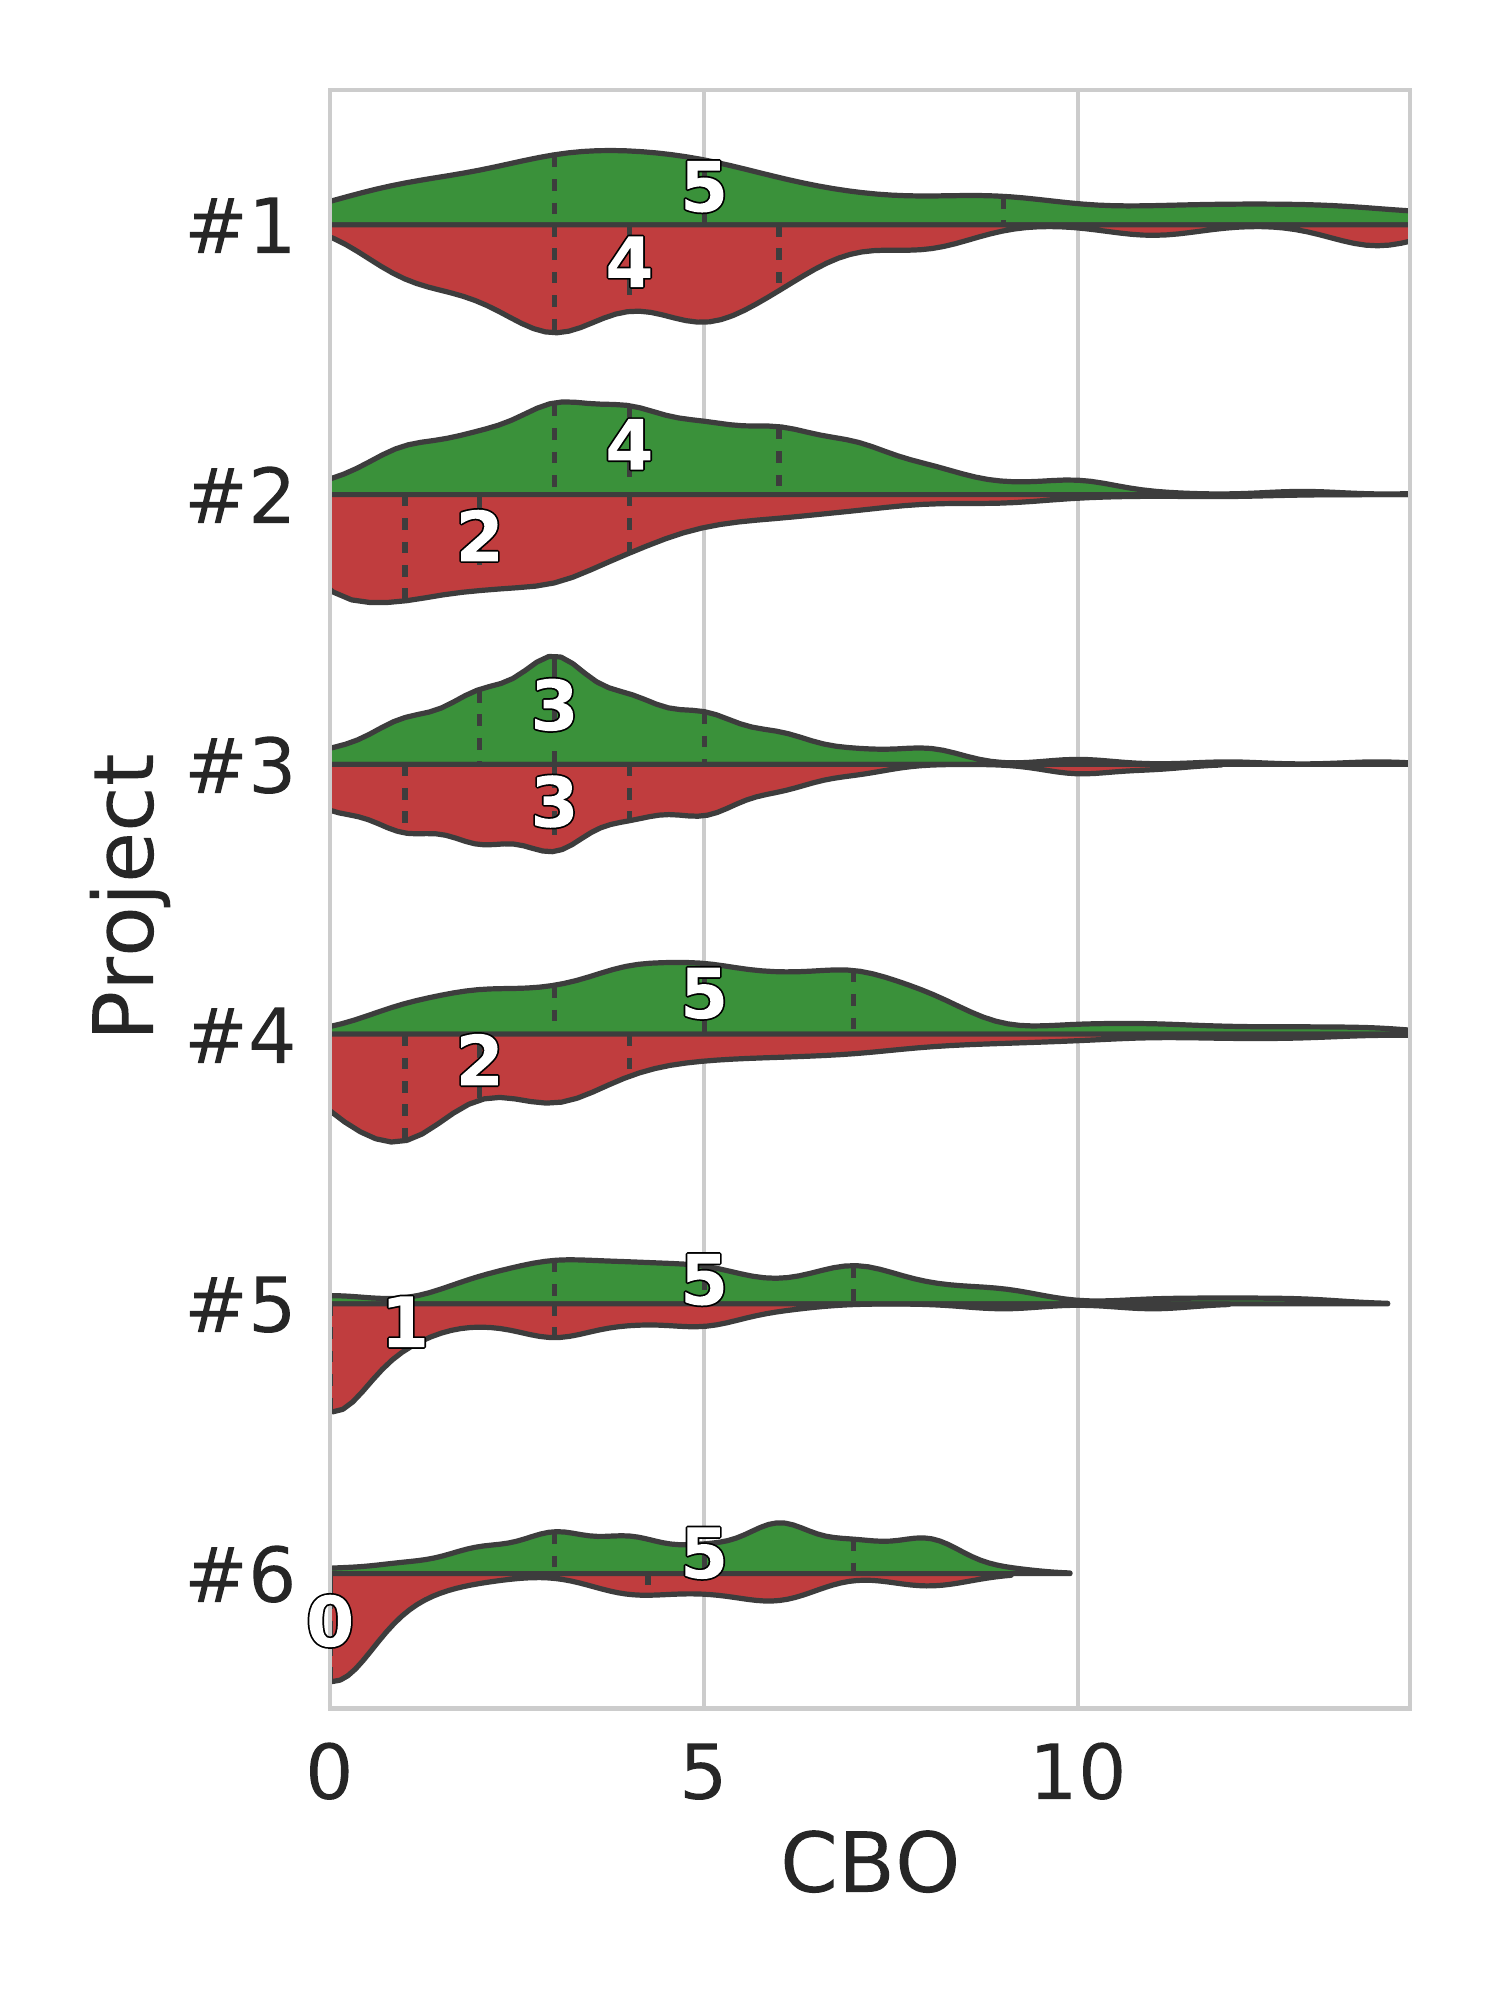}
        \caption{Method-level CBO: The top violin plot indicates methods that underwent an Extract Method refactoring.
            The bottom violin plot indicates methods that do not need to undergo an Extract Method refactoring.}\label{fig:app-per-project-methodcbo}
    \end{subfigure}
    \caption{CBO distributions for open-source and ING code on both class- and method-level per project.}
\end{figure}

\begin{figure}[hbpt]
    \centering
      \begin{subfigure}[htbp]{0.35\textwidth}
        \includegraphics[width=\textwidth]{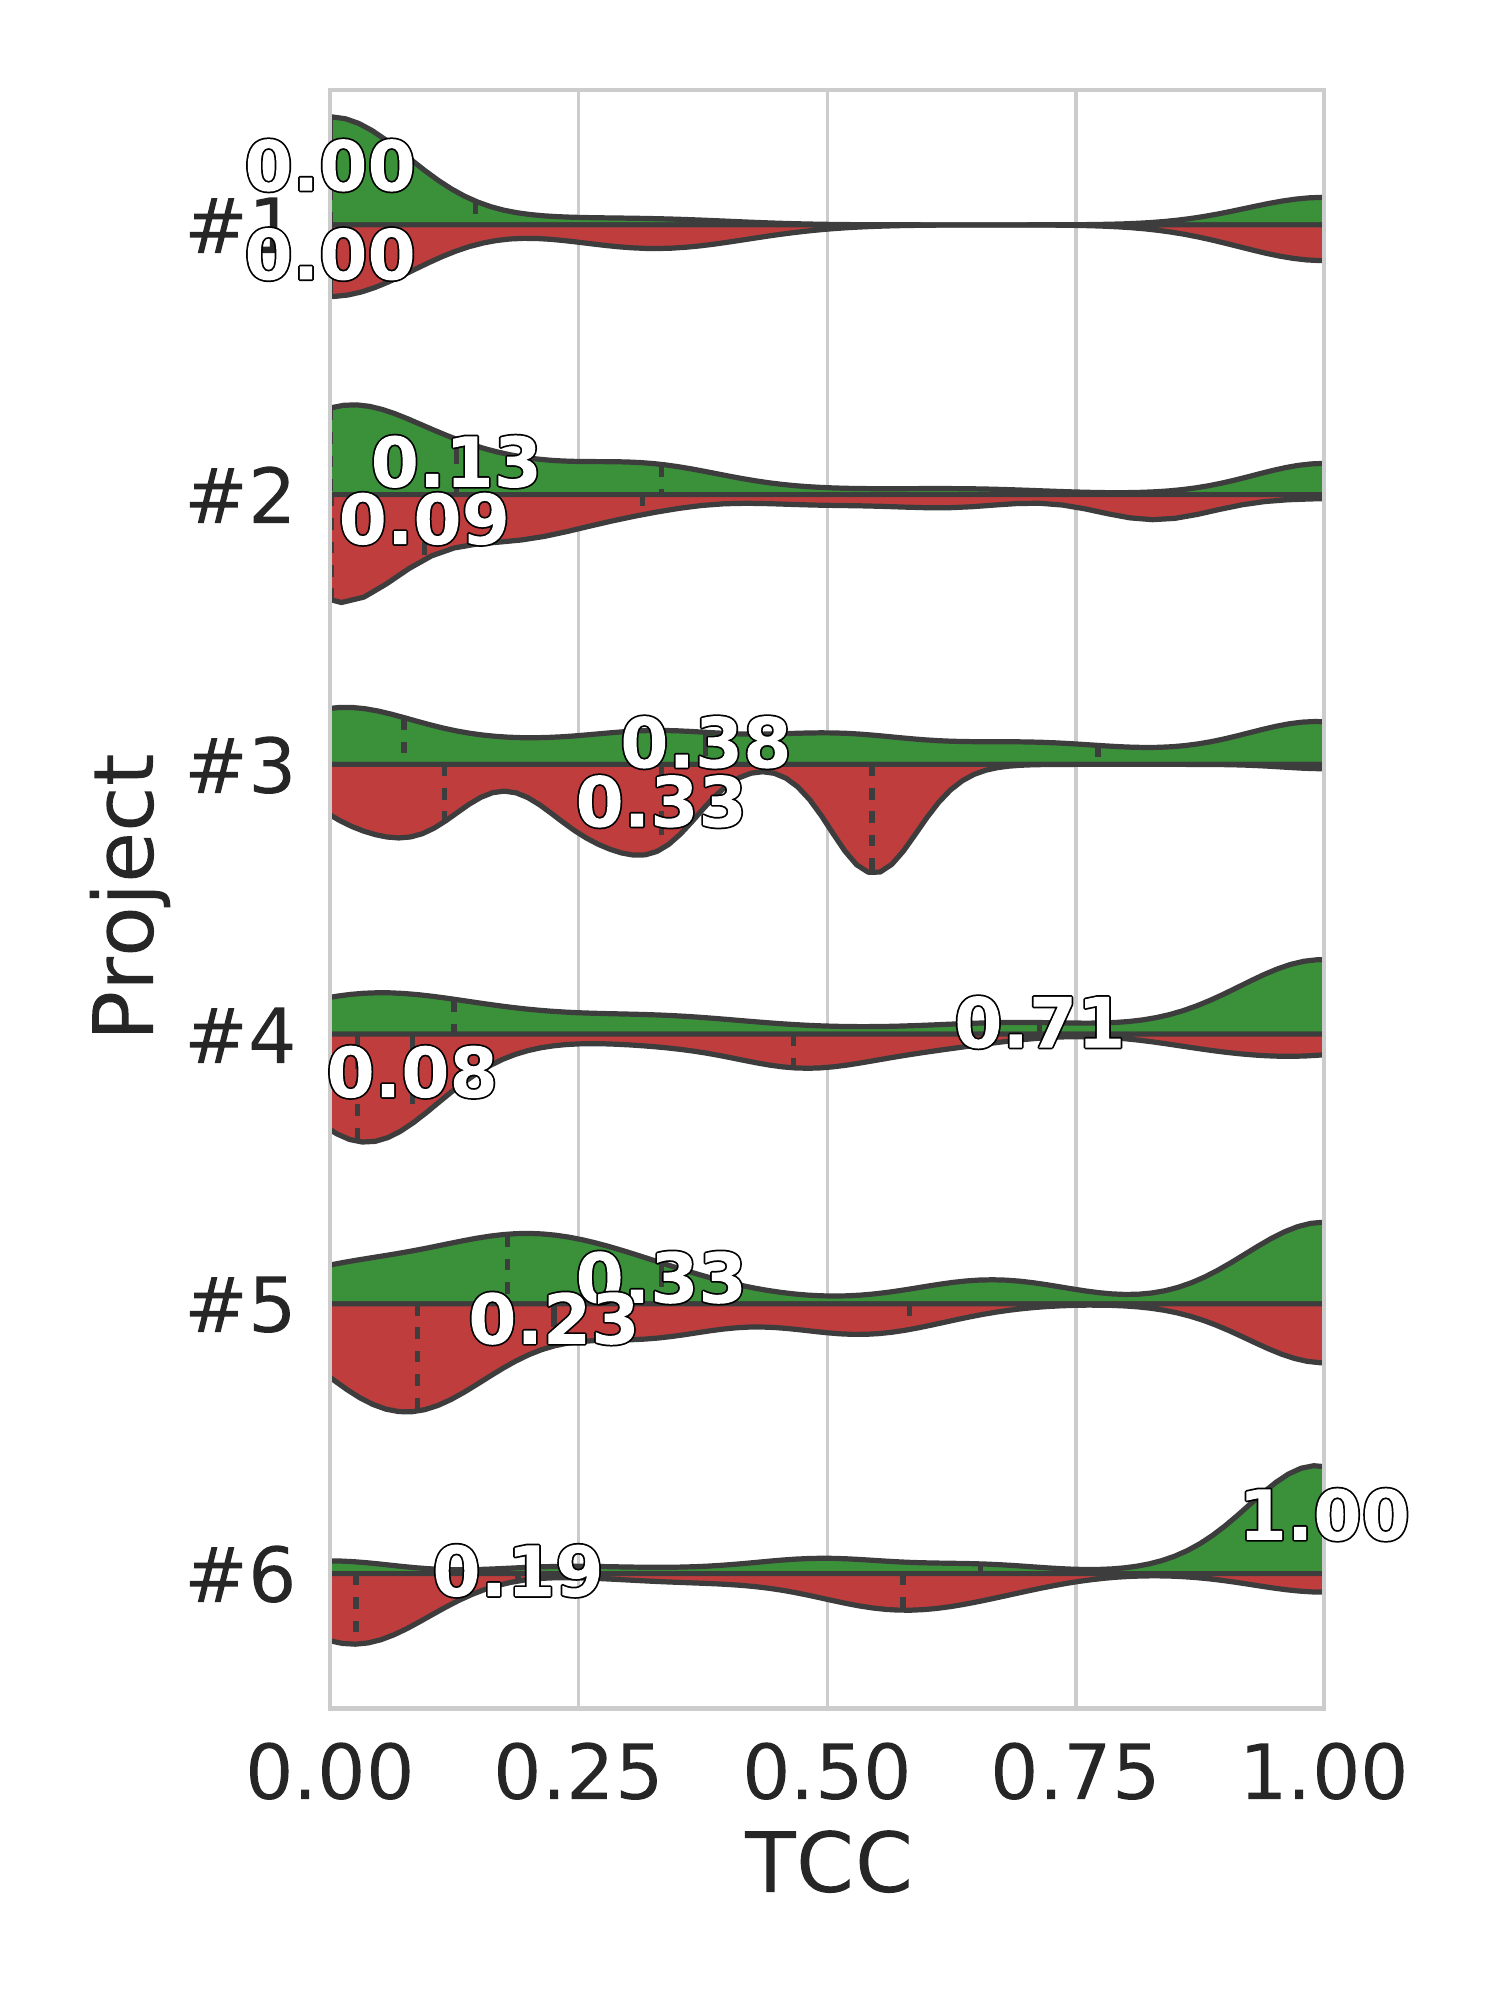}
        \caption{Class-level TCC: The top violin plot indicates classes that contain methods that underwent an Extract Method refactoring.
            The right violin plot indicates classes that do not need to undergo an Extract Method refactoring.}\label{fig:app-per-project-classtcc}
    \end{subfigure}
        \hfill{}
        \begin{subfigure}[htbp]{0.35\textwidth}
        \includegraphics[width=\textwidth]{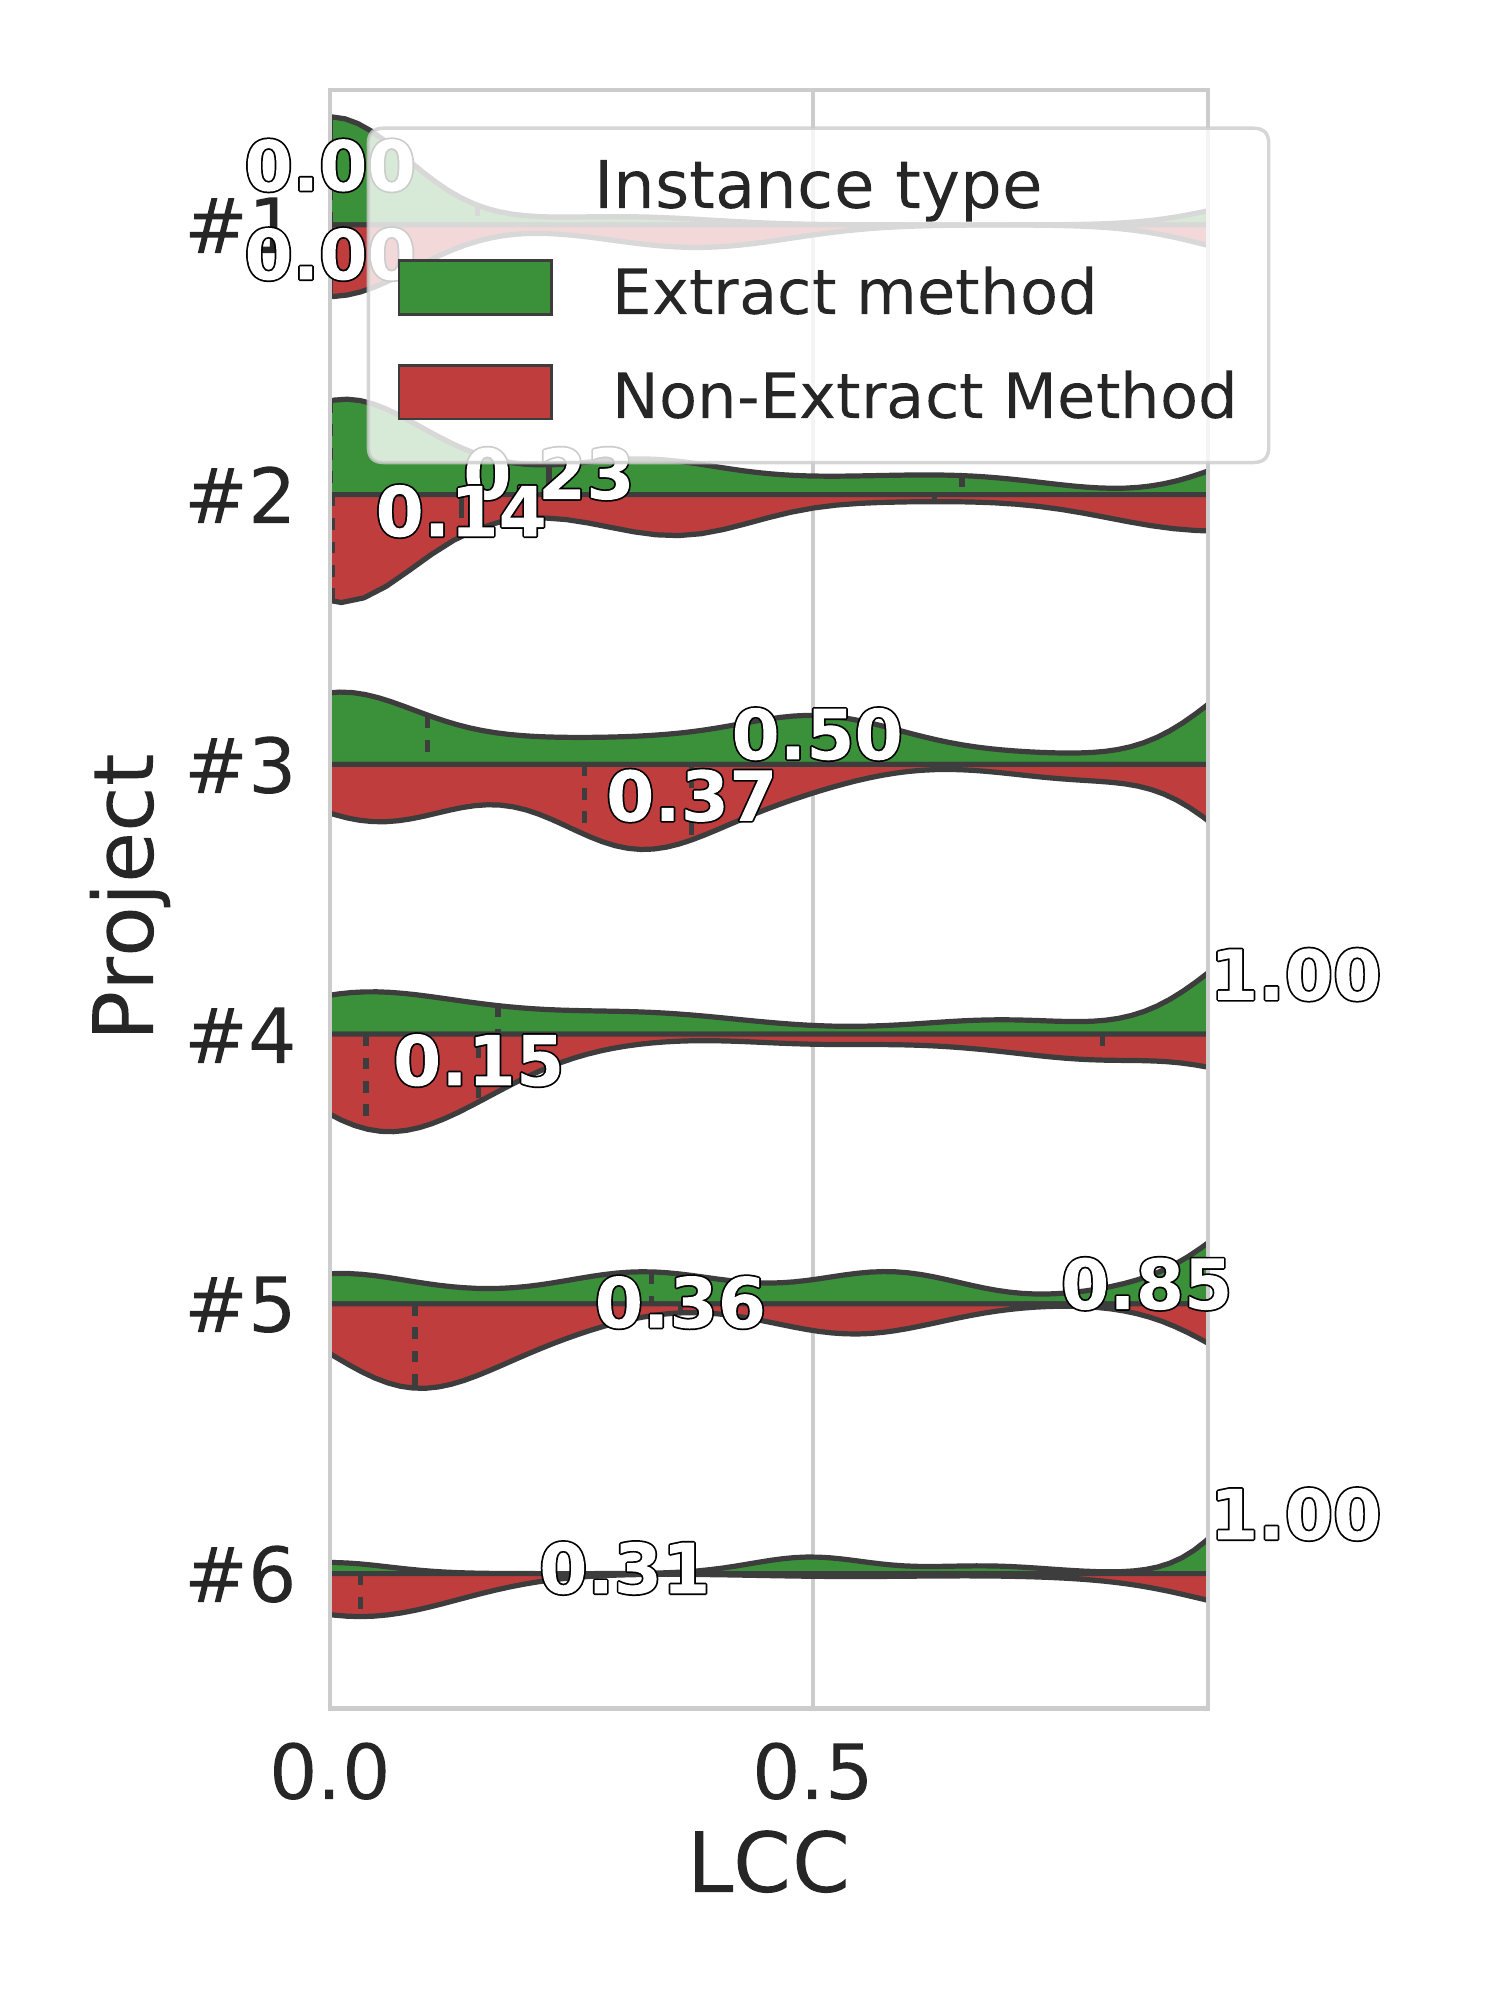}
        \caption{Class-level LCC: The top violin plot indicates classes that contain methods that underwent an Extract Method refactoring.
            The bottom violin plot indicates classes that do not need to undergo an Extract Method refactoring.}\label{fig:app-per-project-classlcc}
    \end{subfigure}
    \caption{TCC and LCC distributions for open-source and ING code on both class-level per project.}
\end{figure}

\FloatBarrier{}
\section{Features used}\label{app:features-used-data-analysis}
Explanations on features can be found in the CK documentation\footnote{\url{https://github.com/mauricioaniche/ck}}.
\subsection{Class level metrics}
    \begin{itemize}[noitemsep]
        \item AnonymousClassesQty
        \item AssignmentsQty
        \item Cbo
        \item ComparisonsQty
        \item LambdasQty
        \item Lcom
        \item Loc
        \item LCC
        \item LoopQty
        \item MathOperationsQty
        \item MaxNestedBlocks
        \item Nosi
        \item NumberOfAbstractMethods
        \item NumberOfDefaultFields
        \item NumberOfDefaultMethods
        \item NumberOfFields
        \item NumberOfFinalFields
        \item NumberOfFinalMethods
        \item NumberOfMethods
        \item NumberOfPrivateFields
        \item NumberOfPrivateMethods
        \item NumberOfProtectedFields
        \item NumberOfProtectedMethods
        \item NumberOfPublicFields
        \item NumberOfPublicMethods
        \item NumberOfStaticFields
        \item NumberOfStaticMethods
        \item NumberOfSynchronizedFields
        \item NumberOfSynchronizedMethods
        \item NumbersQty
        \item ParenthesizedExpsQty
        \item ReturnQty
        \item Rfc
        \item StringLiteralsQty
        \item SubClassesQty
        \item TryCatchQty
        \item UniqueWordsQty
        \item VariablesQty
        \item Wmc
        \item TCC
        \item isInnerClass
    \end{itemize}
\newpage
\subsection{Method level}
\begin{itemize}[noitemsep]
    \item AnonymousClassesQty
    \item AssignmentsQty
    \item Cbo
    \item ComparisonsQty
    \item LambdasQty
    \item Loc
    \item LoopQty
    \item MathOperationsQty
    \item MaxNestedBlocks
    \item NumbersQty
    \item ParametersQty
    \item ParenthesizedExpsQty
    \item ReturnQty
    \item Rfc
    \item StringLiteralsQty
    \item SubClassesQty
    \item TryCatchQty
    \item UniqueWordsQty
    \item VariablesQty
    \item Wmc
\end{itemize}
\FloatBarrier{}

\section{Feature importances and linear coefficients}\label{app:featimp-coef}
All features are class-level except when prefixed with \textit{method}.
\subsection{ING trained models}
\begin{figure}[htbp]
    \includegraphics[width=0.45\textwidth]{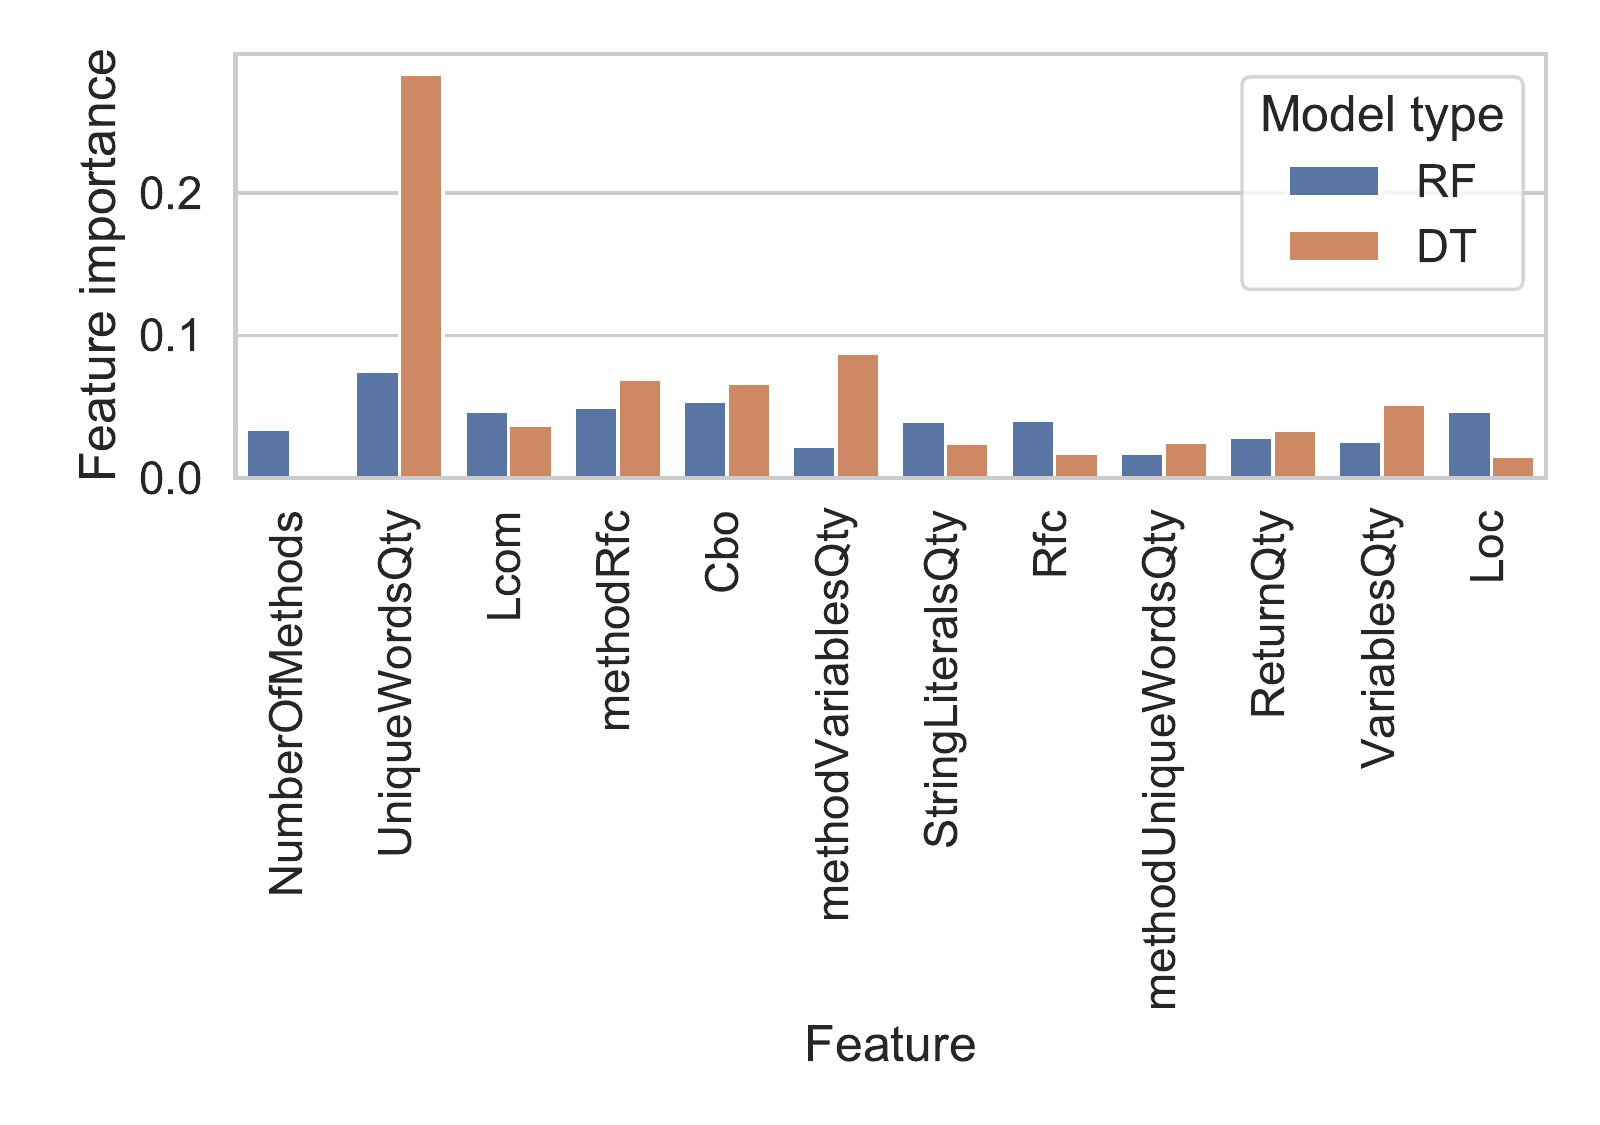}
    \caption[Feature importances ING trained model]{Feature importance for models trained on ING data}\label{fig:feat-importances-ING}
\end{figure}

\begin{figure}[htbp]
    \includegraphics[width=0.45\textwidth]{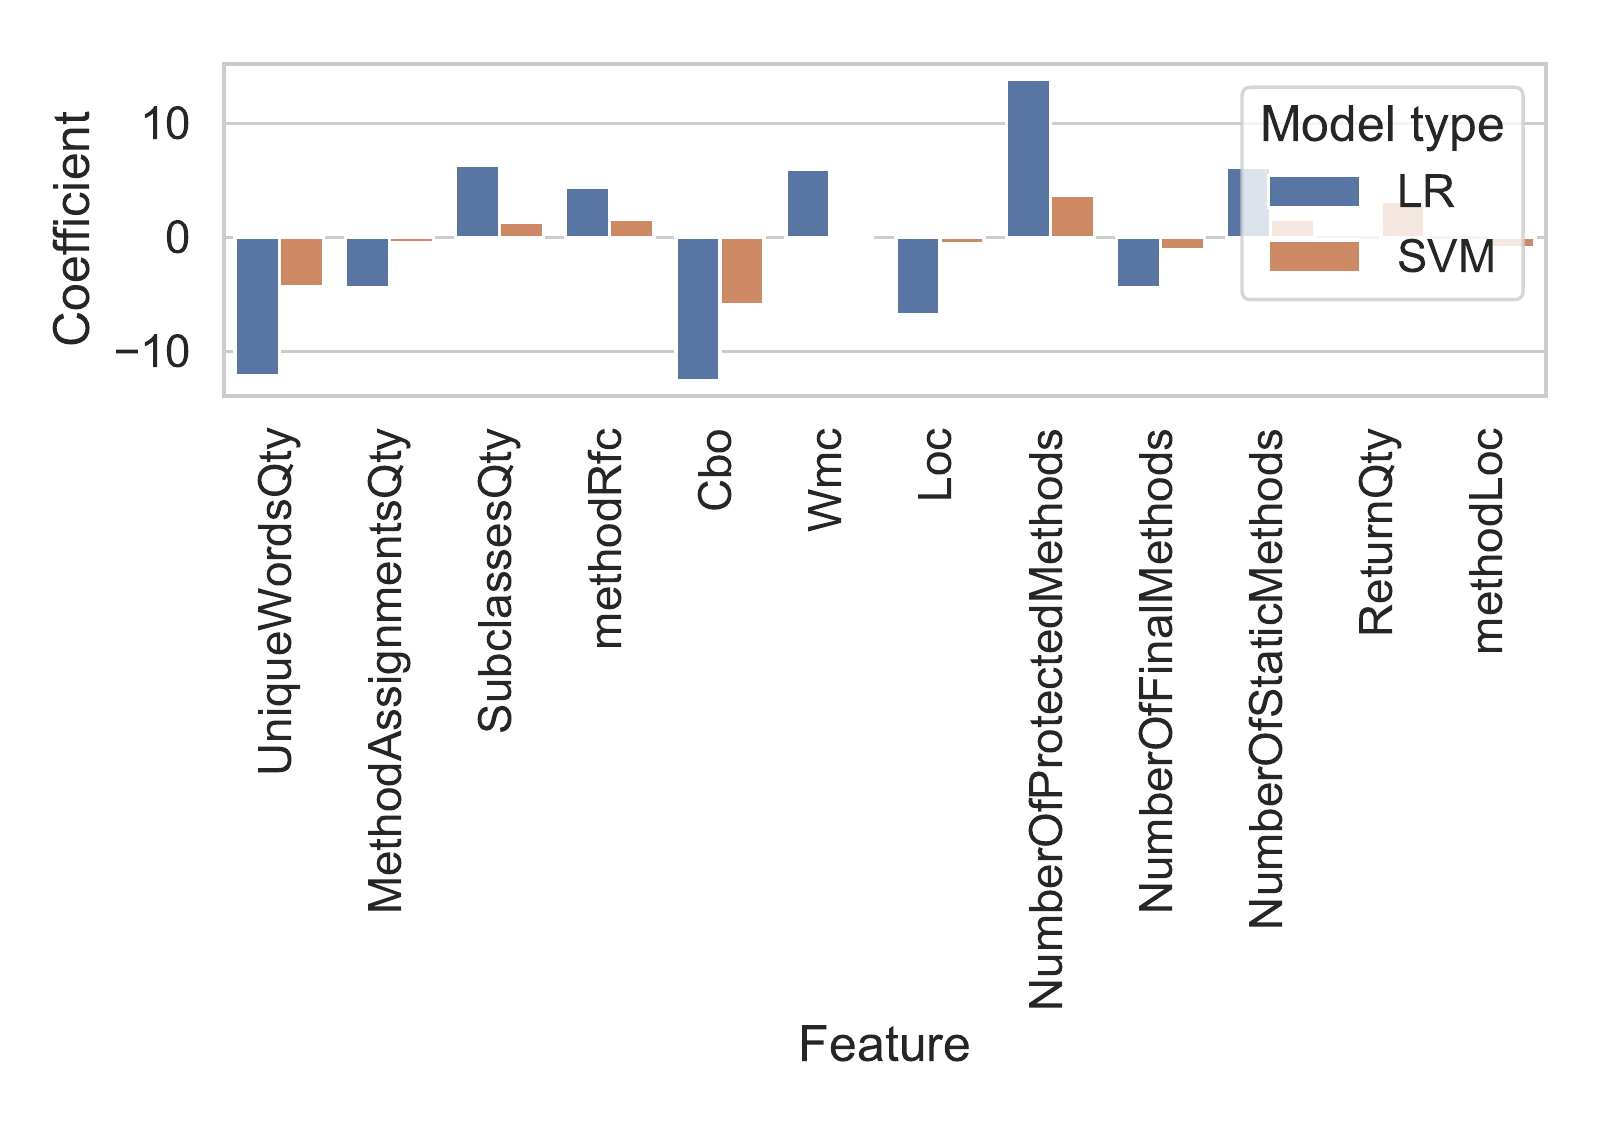}
    \caption[Coefficients ING trained model]{Coefficients for models trained on ING data}\label{fig:coefs-ING}
\end{figure}

\begin{figure}[htbp]
    \includegraphics[width=0.45\textwidth]{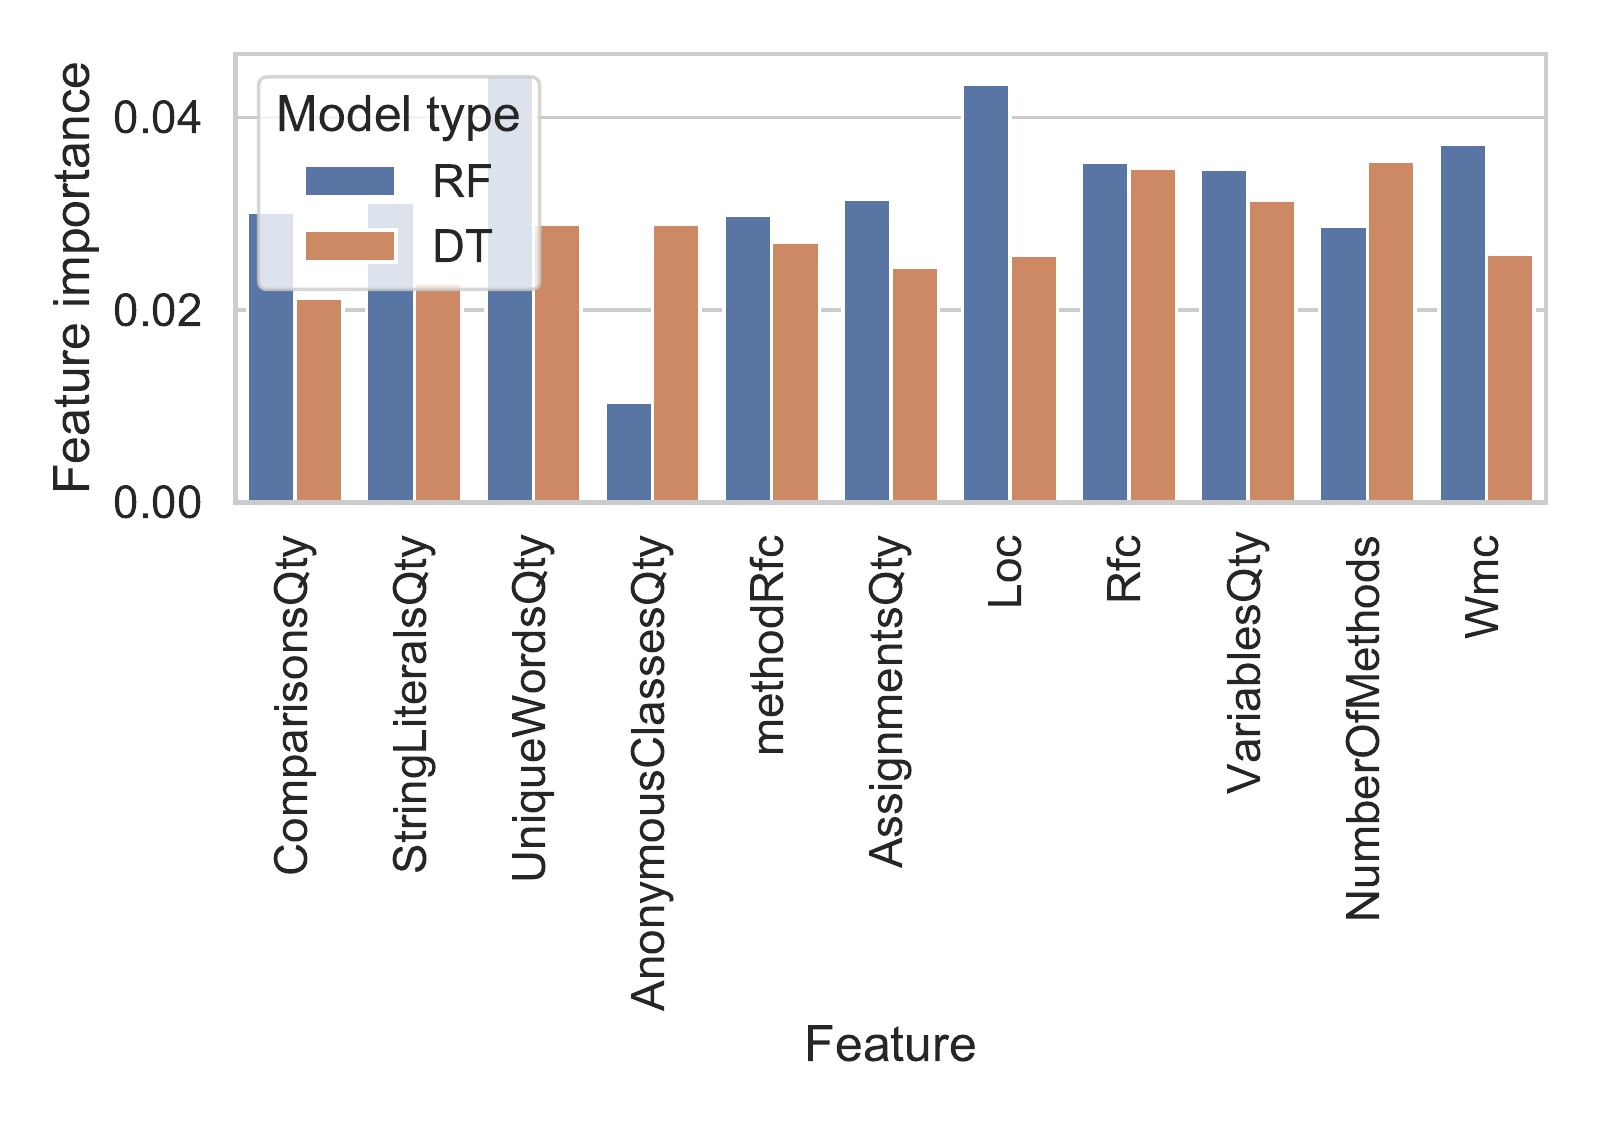}
    \caption[Feature importances open-source trained model]{Feature importance for models trained on open-source data}\label{fig:feat-importances-oss}
\end{figure}
\begin{figure}[htbp]
    \includegraphics[width=0.45\textwidth]{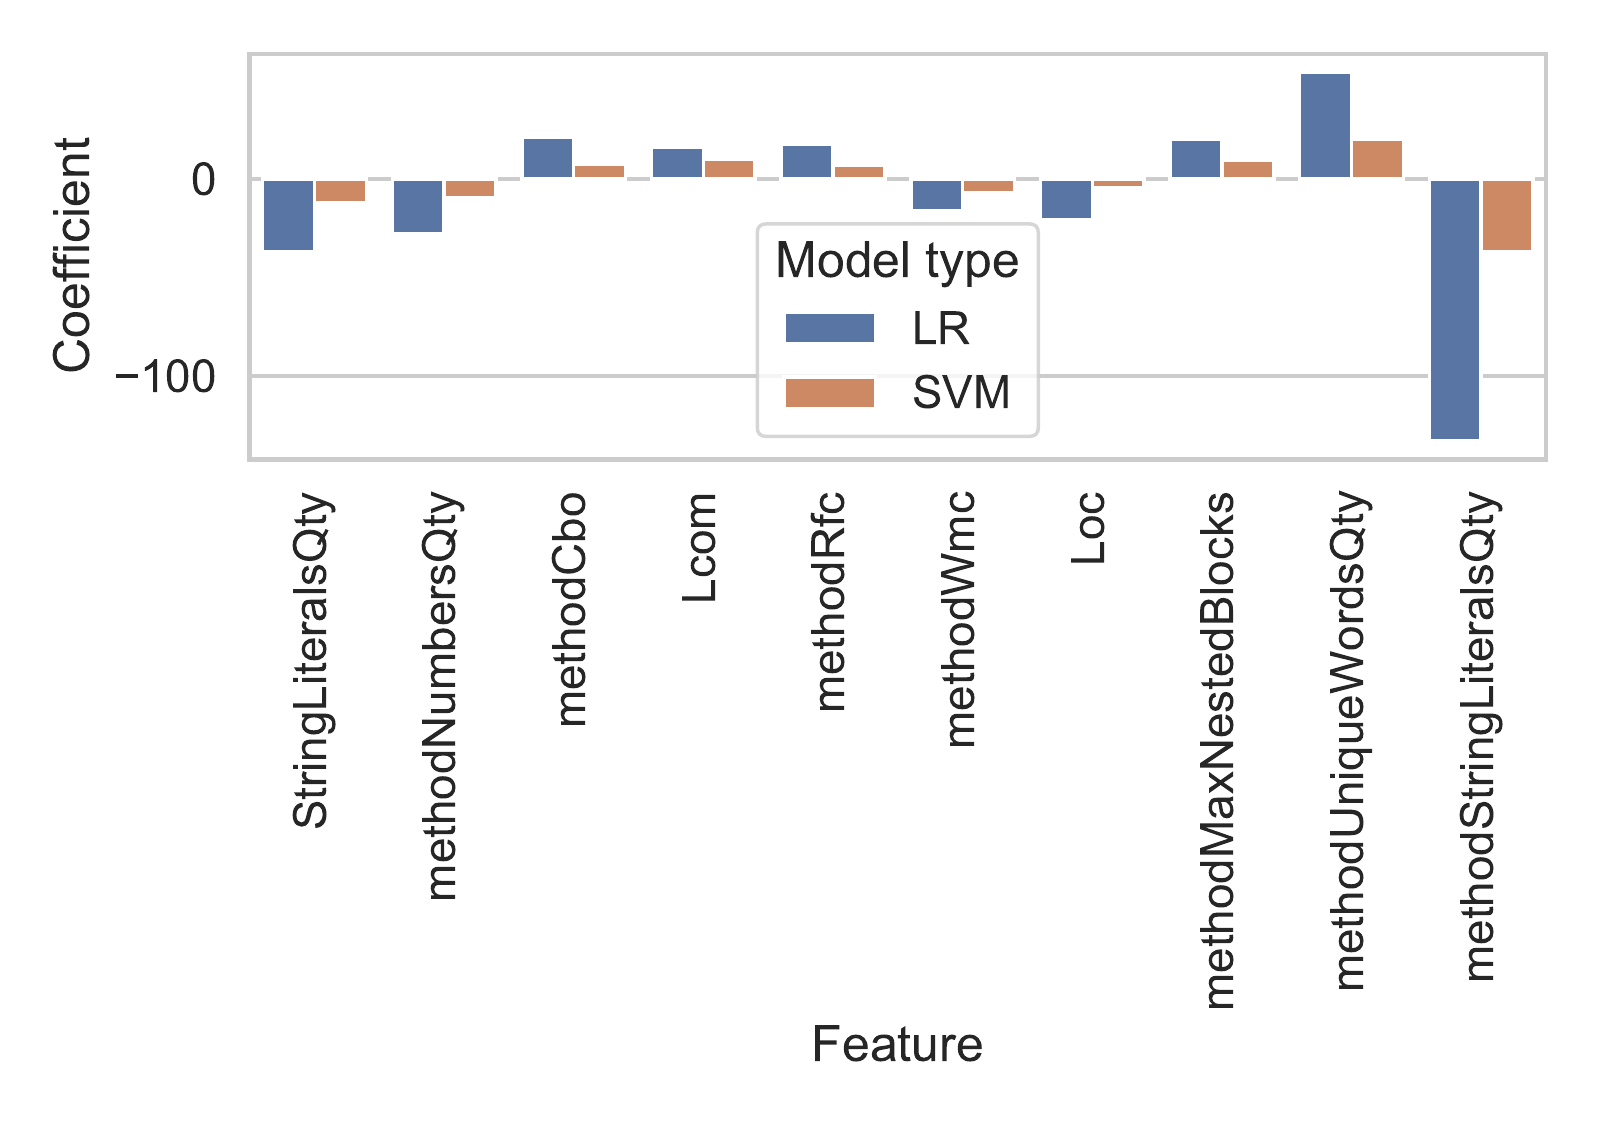}
    \caption[Coefficients open-source trained model]{Coefficients for models trained on open-source data}\label{fig:coefs-oss}
\end{figure}

\subsection{Hyperparameters best-performing models}\label{app:hyperparams}
\begin{table}[htbp]
    \begin{tabular}{ll}
\toprule
Model type &     RF \\
\midrule
bootstrap                &  False \\
ccp\_alpha                &    0.0 \\
criterion                &   gini \\
max\_depth                &     24 \\
max\_features             &   log2 \\
min\_impurity\_decrease    &    0.0 \\
min\_samples\_leaf         &      1 \\
min\_samples\_split        &      2 \\
min\_weight\_fraction\_leaf &    0.0 \\
n\_estimators             &    100 \\
\bottomrule
\end{tabular}

    \begin{tabular}{ll}
\toprule
Model type &       DT \\
\midrule
ccp\_alpha                &      0.0 \\
criterion                &  entropy \\
max\_depth                &       12 \\
min\_impurity\_decrease    &      0.0 \\
min\_samples\_leaf         &        1 \\
min\_samples\_split        &        2 \\
min\_weight\_fraction\_leaf &      0.0 \\
splitter                 &     best \\
\bottomrule
\end{tabular}

    \begin{tabular}{ll}
\toprule
Model type &     LR \\
\midrule
C                 & 81.796 \\
dual              &  False \\
fit\_intercept     &   True \\
intercept\_scaling &      1 \\
max\_iter          &    100 \\
multi\_class       &   auto \\
penalty           &     l2 \\
solver            &   saga \\
tol               &    0.0 \\
\bottomrule
\end{tabular}

    \begin{tabular}{ll}
\toprule
Model type &            SVM \\
\midrule
C                 &          0.718 \\
dual              &          False \\
fit\_intercept     &           True \\
intercept\_scaling &              1 \\
loss              &  squared\_hinge \\
max\_iter          &           1000 \\
multi\_class       &            ovr \\
penalty           &             l1 \\
tol               &            0.0 \\
\bottomrule
\end{tabular}

    \begin{tabular}{lr}
\toprule
Model type &    NB \\
\midrule
var\_smoothing & 0.000 \\
\bottomrule
\end{tabular}

    \caption{Parameters for the best-performing ING trained models}\label{tbl:app-params-ING}
\end{table}
\begin{table}[htbp]
    \begin{tabular}{ll}
\toprule
Model type &     RF \\
\midrule
bootstrap                &  False \\
ccp\_alpha                &    0.0 \\
criterion                &   gini \\
max\_features             &   log2 \\
min\_impurity\_decrease    &    0.0 \\
min\_samples\_leaf         &      1 \\
min\_samples\_split        &      2 \\
min\_weight\_fraction\_leaf &    0.0 \\
n\_estimators             &    200 \\
\bottomrule
\end{tabular}

    \begin{tabular}{ll}
\toprule
Model type &       DT \\
\midrule
ccp\_alpha                &      0.0 \\
criterion                &  entropy \\
max\_features             &     log2 \\
min\_impurity\_decrease    &      0.0 \\
min\_samples\_leaf         &        1 \\
min\_samples\_split        &        2 \\
min\_weight\_fraction\_leaf &      0.0 \\
splitter                 &   random \\
\bottomrule
\end{tabular}

    \begin{tabular}{ll}
\toprule
Model type &     LR \\
\midrule
C                 & 77.681 \\
dual              &  False \\
fit\_intercept     &   True \\
intercept\_scaling &      1 \\
max\_iter          &    500 \\
multi\_class       &   auto \\
penalty           &     l2 \\
solver            &   saga \\
tol               &    0.0 \\
\bottomrule
\end{tabular}

    \begin{tabular}{ll}
\toprule
Model type &            SVM \\
\midrule
C                 &          2.504 \\
dual              &          False \\
fit\_intercept     &           True \\
intercept\_scaling &              1 \\
loss              &  squared\_hinge \\
max\_iter          &           1000 \\
multi\_class       &            ovr \\
penalty           &             l2 \\
tol               &            0.0 \\
\bottomrule
\end{tabular}

    \begin{tabular}{lr}
\toprule
Model type &    NB \\
\midrule
var\_smoothing & 0.000 \\
\bottomrule
\end{tabular}

    \caption{Parameters for the best-performing open-source trained models}\label{tbl:app-params-oss}
\end{table}
\FloatBarrier{}
\section{Confusion matrices and agreement of experts with model predictions}\label{app:confusion-matrices}

\begin{table}[htbp]
    \centering
    \begin{tabular}{lllll}
\toprule
{} &         TP &         TN &        FP &       FN \\
\textbf{Model type} &            &            &           &          \\
\midrule
\textbf{RF        } &  179 (46\%) &  177 (46\%) &   20 (5\%) &   5 (1\%) \\
\textbf{DT        } &  153 (40\%) &  171 (44\%) &   26 (6\%) &  31 (8\%) \\
\textbf{LR        } &  158 (41\%) &  156 (40\%) &  41 (10\%) &  26 (6\%) \\
\textbf{SVM       } &  161 (42\%) &  155 (40\%) &  42 (11\%) &  23 (6\%) \\
\textbf{NB        } &  165 (43\%) &  133 (34\%) &  64 (16\%) &  19 (4\%) \\
\bottomrule
\end{tabular}

    \caption[Confusion matrix ING trained model]{Confusion matrix for models trained and validate on ING code}
\end{table}

\begin{table}[htbp]
    \centering
    \begin{tabular}{lllll}
\toprule
{} &         TP &         TN &         FP &        FN \\
\textbf{Model type} &            &            &            &           \\
\midrule
\textbf{RF        } &  885 (46\%) &  423 (22\%) &  563 (29\%) &   34 (1\%) \\
\textbf{DT        } &  743 (39\%) &  411 (21\%) &  575 (30\%) &  176 (9\%) \\
\textbf{LR        } &  880 (46\%) &  569 (29\%) &  417 (21\%) &   39 (2\%) \\
\textbf{SVM       } &  885 (46\%) &  561 (29\%) &  425 (22\%) &   34 (1\%) \\
\textbf{NB        } &  914 (47\%) &  255 (13\%) &  731 (38\%) &    5 (0\%) \\
\bottomrule
\end{tabular}

    \caption[Confusion matrix open-source trained model]{Confusion matrix for models trained on open-source code and validated on ING code}
\end{table}

\FloatBarrier{}

\section{Survey example}\label{app:survey-deets}
\begin{figure}[htbp]
    \centering
    \includegraphics[width=0.45\textwidth]{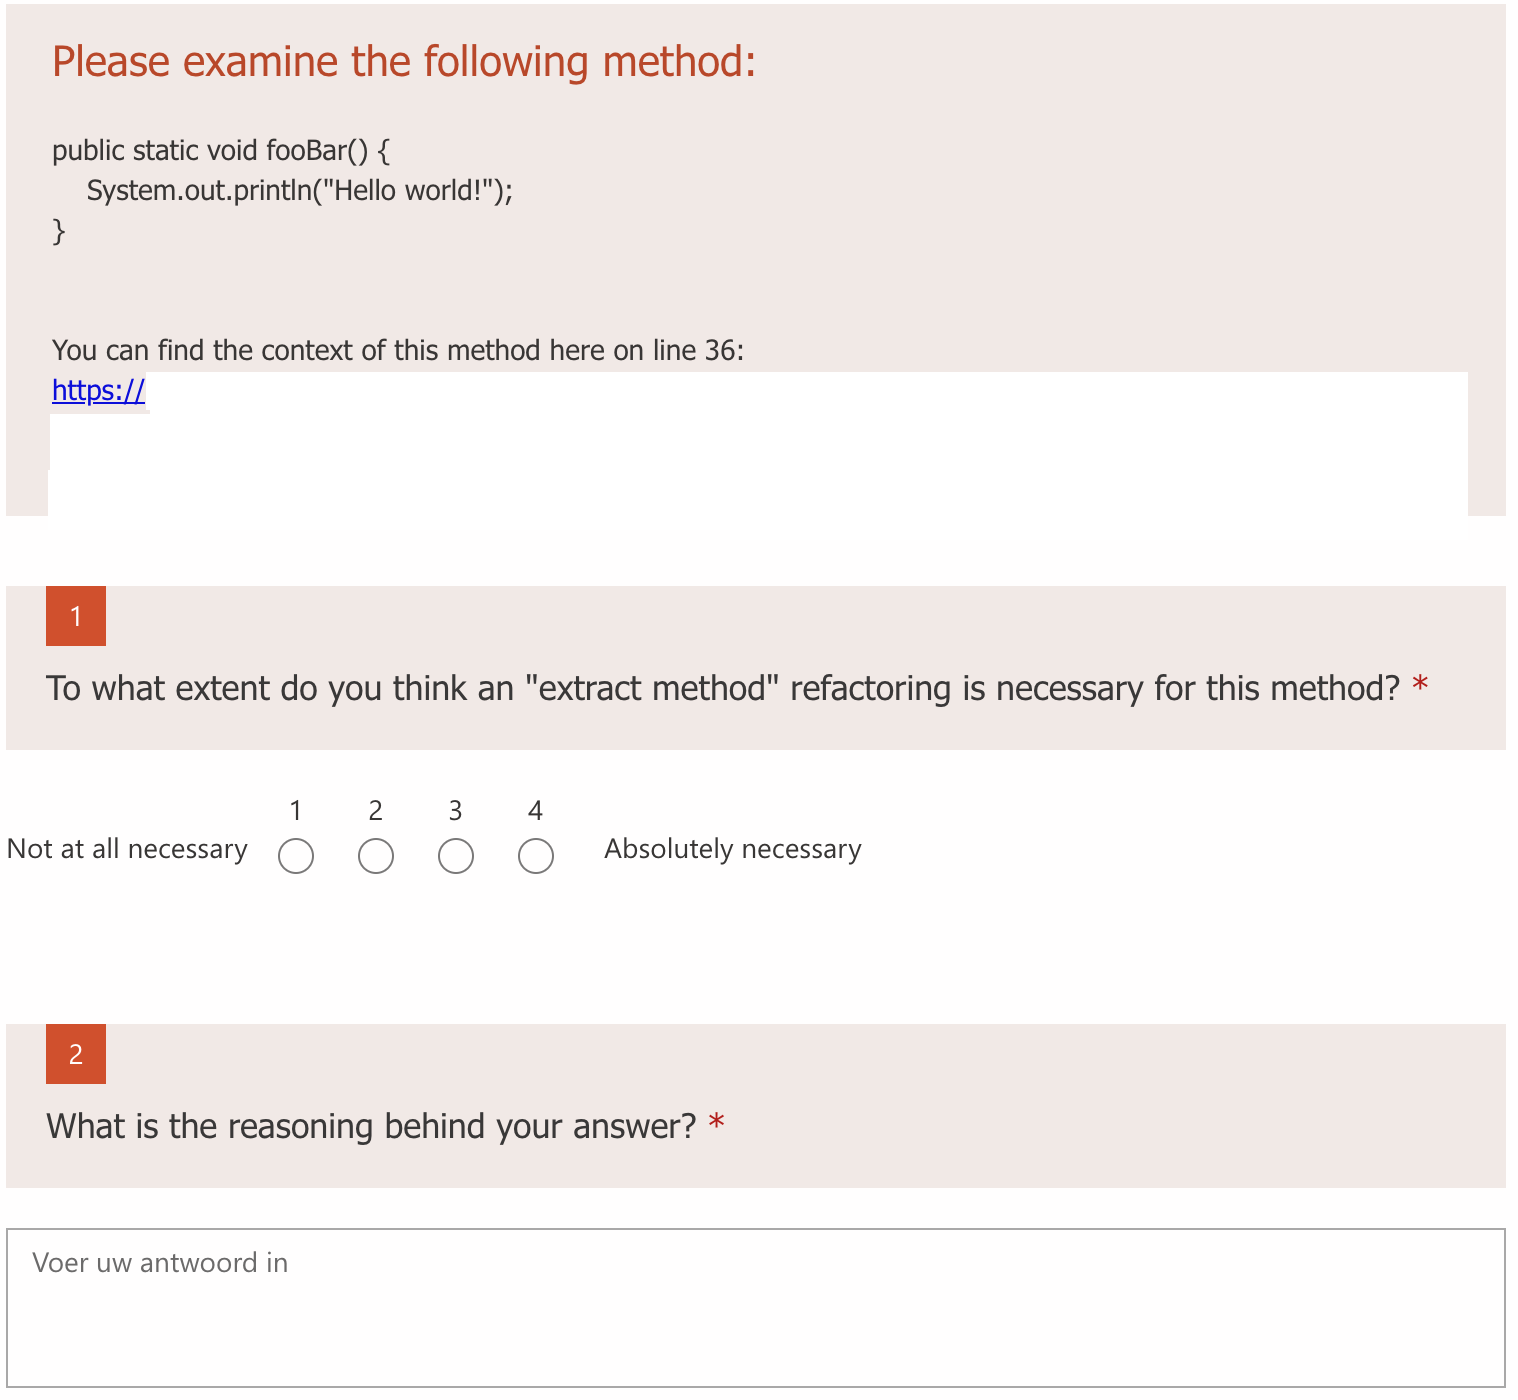}
    \caption[Survey example question]{Example of how a question would look like in the survey.}\label{fig:survey-example}
\end{figure}
% \begin{figure}[htbp]
%     \includegraphics[width=0.45\textwidth]{chapters/5/figures/comment}
%     \caption[Recommendation example]{Example of a refactoring recommendation on a merge made by our model. We include a link to give feedback and a link to an explanation in case the developer is unfamiliar with the refactor in question}\label{fig:ref-rec}
% \end{figure}

\subsection{Expert agreement with model}
\begin{table}[htbp]
    \centering
    \begin{tabular}{lrrrr}
    \toprule
    {}                & \(R_A\) & \(N_A\) & \(N_D\) & \(R_D\) \\
    \textbf{Expert  } &         &         &         &         \\
    \midrule
    \textbf{1       } & 13      & 10      & 0       & 7       \\
    \textbf{2       } & 14      & 7       & 3       & 6       \\
    \textbf{3       } & 10      & 7       & 3       & 10      \\
    \textbf{4       } & 11      & 9       & 1       & 9       \\
    \textbf{5       } & 17      & 10      & 0       & 3       \\\midrule
    \textbf{All/Mean} & 65      & 43      & 7       & 35      \\
    \bottomrule
\end{tabular}

    \caption[Agreement of the experts with the model's prediction]{Agreement of the experts with the model's predictions.}
\end{table}
